# Supplementary material for: Emergent stability in complex network dynamics
Source: arXiv:2007.04890 source file (2023-04-22)
Supplement: Supplementary file 1 [file SupplementaryInformation_new.tex]

%%\documentclass[12pt,a4paper]{article}
%%\usepackage{fullpage}
%%\usepackage{setspace}
%%\usepackage{sidecap}
%%\usepackage{wrapfig}
%%\usepackage{amsfonts}
%%\usepackage{amsmath, amssymb}
%%\usepackage{amsthm}
%%\usepackage{textcomp}
%%\usepackage{graphicx}
%%\usepackage{cite}
%%\usepackage[nottoc]{tocbibind}
%%\usepackage[sort&compress]{natbib}
%%\usepackage[numbers,sort&compress]{natbib}
%%\usepackage{hyperref}
%%\usepackage{color}
%%\usepackage[all]{xy}\xyoption{all}
%%\linespread{1.5}
%%\usepackage{commath}
%%%\usepackage{graphicx}
%%\usepackage{graphicx,epsfig}
%%\usepackage{fancyhdr}
%%\usepackage{calc}
%%%\usepackage[sort&compress]{natbib}
%%\usepackage{setspace}
%%\usepackage{amsfonts}
%%\usepackage{subfigure}
%%\usepackage{hyperref}
%%\usepackage{mathrsfs}
%%\usepackage[pdftex]{graphicx}
%%\usepackage{amsmath}
%%\usepackage{booktabs,hyperref}
%\hypersetup{colorlinks=true}
%%\usepackage{float,caption,hypcap}
%%\usepackage{verbatim}
%%\usepackage{tikz}
%\usetikzlibrary{positioning}
%%\usepackage[framemethod=TikZ]{mdframed}
%%\usepackage{xfrac}
%
%
%\makeatletter
%\newcommand{\rom}[1]{\romannumeral #1}
%\newcommand{\Rom}[1]{\expandafter\@slowromancap\romannumeral #1@}
\makeatother

\expandafter\def\expandafter\normalsize\expandafter{%
	\normalsize
	\setlength\abovedisplayskip{0pt}
	\setlength\belowdisplayskip{5pt}
	\setlength\abovedisplayshortskip{0pt}
	\setlength\belowdisplayshortskip{5pt}
}

\setlength{\parindent}{0em}
\setlength{\parskip}{3pt}

%\definecolor{Gray}{gray}{0.75}

%\newmdenv[backgroundcolor=Gray, leftmargin = 0pt, rightmargin = 0pt, linewidth = 0pt, roundcorner = 2 pt, innerleftmargin=5pt, innerrightmargin=5pt, innertopmargin=5pt, innerbottommargin=5pt]{Frame}

\numberwithin{equation}{section}            %% numbering the equation by section

%\begin{document}

%\newcommand{\av}[1]{\left \langle #1 \right \rangle}
%\newcommand{\av}[1]{\mathchoice
%{\left \langle {#1} \right \rangle}
%{\langle {#1} \rangle}
%{\langle {#1} \rangle}
%{\langle {#1} \rangle}
%}

%\newcommand{\E}{\mathcal{E}}
%\newcommand{\M}{\mathcal{M}}
%\newcommand{\N}{\mathcal{N}}
%\newcommand{\B}{\mathcal{B}}

\newcommand{\G}{Q}

\newcommand{\q}{q}
\renewcommand{\chi}{\mathscr{X}_{\rm nn}}
\renewcommand{\v}{\mathbf v}

\renewcommand{\S}{\mathcal{S}}
\newcommand{\nn}{\rm{nn}}
\newcommand{\Mi}{\av{M}_{i,\odot}}
\renewcommand{\M}{\av{M}_{\odot}}
\newcommand{\Mmu}{\av{M^\mu}_{\odot}}
%
%\renewcommand\section{\@startsection {section}{1}{\z@}%
%	{-3.5ex \@plus -1ex \@minus -.2ex}%
%	{2.3ex \@plus.2ex}%
%	{\normalfont\Large\bfseries}}
%
%%\renewcommand{\thesection}{\arabic{section}}
%
%%\title{\color{blue} \textbf{\\[10mm] Dynamic stability of complex networks \\[10mm] Supplementary information}}
%%\author{}
%\maketitle
%{\footnotesize
%\tableofcontents}
%\thispagestyle{empty}
%\pagebreak
%\pagestyle{plain}
%
%\pagenumbering{arabic}
%
%\pagebreak
%
%\clearpage

%%%%%%%%%%%%%%%%%%%%%%%%%%%%%%%
%% SUPPLEMENTARY INFORMATION %%
%%%%%%%%%%%%%%%%%%%%%%%%%%%%%%%

%\documentclass[12pt,a4paper]{article}

\makeatletter

\definecolor{Gray}{gray}{0.75}

%\makeatletter
%\renewcommand{\rom}[1]{\romannumeral #1}
%\renewcommand{\Rom}[1]{\expandafter\@slowromancap\romannumeral #1@}
%\makeatother

\setlength{\parindent}{0em}
\setlength{\parskip}{5pt}

\numberwithin{equation}{section}            %% numbering the equation by section

\renewcommand{\chi}{x_{\rm nn}}

\renewcommand\section{\@startsection {section}{1}{\z@}%
	{-3.5ex \@plus -1ex \@minus -.2ex}%
	{2.3ex \@plus.2ex}%
	{\normalfont\Large\bfseries}}

\title{\color{blue} \textbf{\\[10mm] Emergent stability in complex network dynamics \\[10mm] Supplementary information}}
%\author{}
\maketitle
\thispagestyle{empty}

\pagebreak
\tableofcontents
\thispagestyle{empty}
\pagebreak
\pagestyle{plain}

\pagenumbering{arabic}

\pagebreak

\maketitle

\section{Analysis framework}
\label{SecFramework}

Our work is based on two main pillars:\ (i) Analytical derivations, leading to our Jacobian ensemble; (ii) Numerical simulations, examining the relevance of our theoretical predictions. Naturally, our analytics rest on a set of approximations and clean model assumptions, as we outline below. Our numerical support, on the other hand, incorporates the full complexity of the system, using both model and empirical networks, and implementing the complete nonlinear dynamics of our testing ground illustrated in Fig.\ 2 of the main text (\textit{i.e}.\ not linearized or otherwise approximated). This allows us to test the performance of our analytical assumptions in realistic settings. Below we outline the main assumptions upon which we build our \textit{analytical} advances, and also list the extended numerical tests we perform to examine the applicability limits of each of these assumptions.

We begin with Eq.\ (3) of the main text, which we write here again, for convenience

\begin{equation}
\dod{x_i}{t} = 
M_0 \big( x_i(t), \m \f0i \big) + 
\g \sum_{j = 1}^{N}  \m Aij M_1 \big( x_i(t), \m \f1i \big) \m Gij M_2 \big(x_j(t), \m \f2i \big).
\label{Eq3}
\end{equation}

The equation has three components:\ The weighted network topology $A,G$; the rate parameters $\g$ and $\f_i = (\m \f0i,\m \f1i,\m \f2i)$, which we denote collectively by $\f$; and the dynamic functions $M_q(x)$, $q = 0,1,2$. We now list the assumptions we make on each of these components.

\subsection{Dynamics}
\label{SecAssumption1}

\textbf{\color{blue} Assumption 1}.\ 
In (\ref{Eq3}) we assume that the dynamic functions can be expressed as a Hahn power series around $x_i = 0$, writing

\begin{equation}
M_q(x_i,\m \f qi) = \sum_{n = 0}^{\infty} \m Cqn(\m \f qi) 
x_i^{\m \Gamma qn}
\label{Hahn}
\end{equation}    

for $q = 0,1,2$. Here $\m \Gamma qn$ represents a sequence of real powers, $\m \Gamma qn \in \mathbb{R}$, generalizing the classic Taylor expansion to include also negative, rational or irrational powers. This allows us to express via (\ref{Hahn}) practically any relevant nonlinear function including ones that cannot be Taylor expanded around zero. 

In (\ref{Hahn}) we distinguish between the coefficients $\m Cqn$ and the powers $\m \Gamma qn$. The former, we assume, depend on $\m \f qi$, and may therefore be distributed across all nodes. The latter, on the other hand are uniform, capturing the shared dynamic processes across all network components. Hence, our formulation asserts that the powers that participate in (\ref{Hahn}) define the \textit{system's} dynamics, while the coefficients capture each \textit{node's} potentially idiosyncratic rate parameters. This, we emphasize , is our \textit{assumption}, that the dynamics can be expressed in this way, \textit{i.e}., node/link specific coefficients, but fixed powers. The interpretation and rationale behind this assumption we discuss in the main text, and, in more detail, through the examples below.   

\textbf{Assumption 1's motivation}.\ To get a sense of Assumption 1 in practice we consider three functions that appear in our testing ground - logistic growth (Population), mass-action kinetics (Biochemical) and the Hill function (Regulatory). The first of these three can be expressed via (\ref{Hahn}) as

\begin{equation}
M_q(x_i,\m \f qi) = b_i x_i \left( 1 - \dfrac{x_i}{c_i} \right) = 
b_i x_i - \dfrac{b_i}{c_i}x_i^2
\label{Logistic}
\end{equation}

having coefficients $b_i$ and $-b_i/c_i$, and powers $x_i^1$ and $x_i^2$. This can be cast on the form of (\ref{Hahn}) by setting $\m C00 = b_i, \m C01 = -b_i/c_i$ and $\m \Gamma00 = 1, \m \Gamma01 = 2$. Here, in this context, Assumption 1 is taken to mean that all nodes undergo the same process of logistic growth, following the form $\sim x_i(1 - x_i)$, \textit{i.e}.\ the \textit{powers} $1$ and $2$. However this logistic process may be characterized by different node-specific \textit{rates}, namely, $b_i$, the growth rate and $c_i$, the environment carrying capacity, are potentially $i$-dependent. This potential diversity is expressed via the \textit{coefficients} $\m C00$ and $\m C01$, which are indeed the only factors in (\ref{Logistic}) that depend on $b_i,c_i$. This clearly demonstrates the different role of the two factors:\ the powers capture the defining features of logistic growth - linear reproduction ($x_i^1$) attenuated by quadratic competition ($-x_i^2$) and therefore they are identical for all nodes; the coefficients, on the other hand, incorporate the specific rates of these two processes, which may change across nodes or due to shifting environmental conditions. 

In mass-action-kinetics we consider interaction processes of the form $aX_i + bX_j \xrightarrow{\g} \m Xij$, in which $a$ copies of $X_i$ and $b$ copies of $X_j$ combine to form the compound molecule $\m Xij$. This, in (\ref{Eq3}) leads to an interaction term following $\g \m Gij x_i^a x_j^b$,  having the rate constant $\g \m Gij$ (potentially link-specific) and the powers $a,b$. Here the powers represent the \textit{order} of the interaction, which is determined by stoichiometry, and hence cannot be easily perturbed. On the other hand, the coefficient is the reaction \textit{rate}, which is, indeed, subject to external perturbation by, \textit{e.g}., changing temperature or chemical affinity.  

As our third example, we consider a Hill function, often encountered in regulatory or population dynamics, following

\begin{equation}
M_q(x_i,\m \f qi) \dfrac{x_i^h}{1 + \left(x_i b_i\right)^h} = 
\left( \dfrac{1}{b_i} \right) x_i^h -
\left( \dfrac{1}{b_i} \right)^2 x_i^{2h} + \dots = 
\sum_{n = 0}^{\infty} (-1)^n \left( \dfrac{1}{b_i} \right)^{n + 1}
x_i^{(n + 1)h}.
\label{Hill}
\end{equation}

Here we have $\m Cqn(\m \f qi) = (-1)^n (1/b_i)^{n + 1}$ and $\m \Gamma qn = (n + 1)h$. Therefore, in this example, $b_i$ is considered a \textit{rate parameter}, affecting the \textit{coefficients}, whereas $h$ is \textit{intrinsic}, embedded in the \textit{powers}. Indeed, $h$ here affects the functional form of $M_q(x)$, by controlling the saturation rate of the Hill function, while $b_i$ determines the upper value of the saturation, which, as our formalism indicates, is less intrinsic.

To summarize:\ we consider all (potentially nonlinear) functions $M_q(x)$ that can be expressed via (\ref{Hahn}); we allow diversity in the coefficients $\m Cqn$, but assume uniform powers $\m \Gamma qn$. Hence all $M_q(x)$ are of the same \textit{family} or \textit{functional form}, \textit{e.g}., $\sim b_i x(1 - x/c_i)$, but with distributed \textit{parameters} $b_i,c_i$. Therefore, \textit{parameters}, in our definition, are factors that affect $\m Cqn$, but do not feed into the powers $\m \Gamma qn$. 

\textbf{\color{blue} Outcome 1 - derivative functions}.
Throughout our derivation we apply different mathematical operations on $M_q(x)$, such as multiplication ($M_1 \times M_2$), division ($M_0/M_1$), derivation ($M_1^\prime$), inversion ($M_0^{-1}(x)$) or composition ($M_0(M_1(x))$). Each of these operations preserves the separation between $\m Cqn$ and $\m \Gamma qn$, and hence our distinction between the node/link dependent coefficients vs.\ the uniform powers is equally preserved. For example, in case $F(x) = M_1(x) \times M_2(x)$ it yields a new Hahn series, whose coefficients comprise products of the form $\m C1n \m C2m$ and whose powers are constructed from sums of the form $\m \Gamma1n + \m \Gamma2m$. Therefore, $F(x)$'s expansion continues to have parameter dependent coefficients alongside parameter \textit{in}dependent powers. A similar separation is preserved for each of the other operations mentioned above.

\textbf{Testing the limits of Assumption 1}.\
In Supplementary Sections \ref{SecMixedDynamics} and \ref{SecDistributedPowers} we challenge Assumption 1 and analyze systems with mixed-dynamics, in which nodes/links are characterized by two or more different power sets $\m \Gamma qn$, or by a continuum of powers. This helps generalize (\ref{Eq3}) to treat systems with several competing dynamic mechanisms.

\textbf{\color{blue} Assumption 2}.\
In (\ref{Eq3}) we take the interaction term to be factorizable, writing it in product from $M_1(x) \times M_2(x)$. This is, indeed, a common structure, observed in our range of social, biological and technological systems, as can be observed in Fig.\ 2 of the main text. It excludes, however, several forms of dynamics, most notably - diffusive dynamics, in which the interaction follows $M(x_j - x_i)$.   
 
\textbf{Testing the limits of Assumption 2}.\
This assumption, while helping our analytical derivations, is by no means essential, and can, in practice, be relaxed. We demonstrate this by deriving the Jacobian from our Power dynamics (Supplementary Section \ref{SecPowerDynamics}, in which the interaction is given by $M(x_i,x_j) \sim \sin(x_j - x_i)$. 

\textbf{\color{blue} Assumption 3}.\
Our final dynamic assumption is that the interactions are additive, allowing us to express them as $\sum_{j = 1}^N \m Aij \m Gij \cdots M_2(x_j)$. More generally, one can also write $M_2(\sum_{j = 1}^N \m Aij \m Gij x_j)$, in which $i$ receives a nonlinear cumulative input from its surrounding neighbors.
 
\textbf{Testing the limits of Assumption 3}.\
This assumption is challenged by our application to Population 2 dynamics in Sec.\ \ref{SecNonAdditiveDynamics}, which is specifically designed around the form $M_2(\sum_j \cdots)$ rather than $\sum_j \cdots M_2(x_j)$. 

\textbf{\color{blue} Assumption 4}.\
Equation (\ref{Eq3}) exhibits at least one fully positive fixed-point $\x^* = (x_1,\dots,x_N), x_i \ge 0$, around which we seek to construct $J$ and assess its stability. In this notation we denote the fixed-point by omitting the $t$ dependence, \textit{i.e}.\ $x_i$ instead of $x_i(t)$, expressing the fact that these are stationary states.

\textbf{Testing the limits of Assumption 4}.\
In Sec.\ \ref{SecExtinctionDynamics} we investigate population dynamics with a mixture of cooperative and adversarial interaction (positive/negative $\m Gij$), under which a varying fraction of nodes undergoes extinction. We seek the limits of our framework's applicability under these conditions by observing our predicted $J$-patterns on the set of surviving nodes.

\subsection{Weighted topology}
\label{SecTopology}

The weighted network topology is given by $A \otimes G$, where the Hadamard product $\otimes$ represents matrix multiplication element-by-element. The $N \times N$ adjacency matrix $A$ is large ($N \to \infty$) sparse ($\sum_{i,j} \m Aij/N^2 \ll 1$), has no isolated components and binary ($\m Aij \in \{ 0,1 \}$) with a vanishing diagonal ($\m Aii = 0$). The elements of the weight matrix $G \ge 0$ are drawn at random from $P(G)$, capturing the probability density for a random weight to have $\m Gij \in (G,G + \delta G)$. We categorize all nodes via their binary and weighted degrees

\begin{equation}
\begin{array}{ccc}
k_i = \displaystyle \sum_{j = 1}^N \m Aij,
& \,\,\,\,\,\,\,\, &
d_i = \displaystyle \sum_{j = 1}^N \m Aij \m Gij
\end{array},
\label{Degree}
\end{equation} 

the former discrete ($k_i = 1,2,\dots$) and the latter continuous ($d_i \in \mathbb{R}$). The network is, therefore, characterized by the degree-distribution $P(k)$, capturing the probability that a randomly selected node $i$ has $k_i = k$, and by the density function $P(d)$, capturing the probability density that $d_i \in (d, d + \delta d)$. For simplicity, we use a loose notation $P(x)$ to denote both discrete probability functions ($P(X = x)$ and continuous density functions ($P_X(x)$). Therefore, the specific meaning of $P(x)$ should be deduced from context, based on the nature of $x$, continuous or discrete.

In (\ref{Eq3}) both $P(k)$ and $P(d)$ can take any arbitrary form, including homogeneous (\textit{e.g.}, Poisson, exponential) or fat-tailed distributions (\textit{e.g.}, scale-free). This is clearly observed, for instance, in Fig.\ 3 of the main text, where we implement our analysis on both Erd\H{o}s-R\'{e}nyi (ER) networks and scale-free (SF) networks with different weight distributions, alongside an array of empirical networks. Having said that, we also emphasize that many of our results are linked to degree-heterogeneity, from the scaling of $\m Jij$ with $d_i,d_j$ to the asymptotic stability that relies on $\beta > 0$ in Eq.\ (9) of the main text. Therefore, such heterogeneity in $P(k)$ or $P(d)$, while, strictly speaking, is \textit{not} a necessary condition, does, in fact, represent an underlying motivation for parts of our analysis.

In our analysis we encounter several average quantities extracted from $P(k),P(d)$. Most naturally, the average degree $\av k$ or the average weighted degree $\av d$. Beyond these immediate statistics we also encounter \textit{neighborhood averages}, which we denote by

\begin{equation}
\av X_{i,\odot} = \dfrac{1}{d_i} \sum_{j = 1}^N \m Aij \m Gij X_j.
\label{NeighborAverage}
\end{equation}

This captures the weighted average over observable $X_j$ extracted from node $i$'s direct network neighbors. In (\ref{NeighborAverage}) we use the symbol $\odot$ to represent a \textit{neighborhood}, hence $i,\odot$ is the group of $i$'s direct neighbors. For example, $\av d_{i,\odot}$ represents the average weighted degree of all nodes surrounding $i$. This allows us to express the average neighbor node $\knn$, appearing in main text Eq.\ (6), via

\begin{equation}
\knn = \av d_\odot = \dfrac{1}{N} \sum_{i = 1}^N \av d_{i,\odot}.
\label{dnn}
\end{equation}   

Here, in addition to our paper's notation $\knn$, we also used our currently introduced $\odot$ to express the \textit{neighborhood} average. This form of neighborhood averaging is, in fact, naturally ingrained in our dynamic equation (\ref{Eq3}), where we can use (\ref{NeighborAverage}) to express the summation on the r.h.s.\ as

\begin{equation}
\sum_{j = 1}^{N}  \m Aij \m Gij M_2 \big(x_j,\m \f2j \big) =
d_i \av{M_2(x)}_{i,\odot} \equiv d_i \Mi.
\label{M2xOdot} 
\end{equation}

This represents a direct application of (\ref{NeighborAverage}) over the observable 

\begin{equation}
M_j = M_2(x_j,\m \f2j).
\end{equation}

Therefore, $\Mi$ denotes the (weighted) average value of $M_2(x_j,\m \f2j)$ within $i$'s direct neighborhood.

Finally, another form of averaging we encounter during our analysis is the degree-conditional averages $\av{X|d}$ and $\av{X|d}_\odot$. First we define the set

\begin{equation}
\G(d) = \Big\{i \in \{1,\dots,N\} \Big| d_i \in (d, d + \delta d) \Big\},
\label{Gk}
\end{equation}

comprising all nodes whose weighted degree is in the range $(d, d + \delta d)$. Such binning within the interval $(d, d + \delta d)$ is required since $d$ is a continuous variable, and hence writing $d_i = d$ yields a group of measure zero. The conditional averages are then defined as

\begin{eqnarray}
X(d) &=& \av{X|d} = \dfrac{1}{|\G(d)|} \sum_{i \in \G(d)} X_i
\label{avXd}
\\[5pt]
X_{\nn}(d) &=& \av{X|d}_\odot = \dfrac{1}{\G(d)} \sum_{i \in \G(d)} \av{X}_{i,\odot}
= \dfrac{1}{|\G(d)|} \sum_{i \in \G(d)} \dfrac{1}{d_i} 
\sum_{j = 1}^N \m Aij \m Gij X_j,
\label{avXnnd} 
\end{eqnarray}
  
where $|\G(d)|$ is the number of nodes in $\G(d)$. Here $X(d)$ is the average observable $X_i$ for nodes $i \in \G(d)$, thus, for example, $x(d)$ represents the average activity of nodes with weighted degree $d$. Similarly, when plotting $\m Wii$ vs.\ $d_i$ in Fig.\ 3 of the main text, then, formally speaking, we measured $W_{\rm Diag}(d)$, \textit{i.e}.\ the average diagonal term of $W$ over all nodes $i \in \G(d)$. 

The second average, $X_{\nn}(d)$ in (\ref{avXnnd}), is constructed from the neighborhood average taken over all nodes in $\G(d)$. It is, therefore, designed to characterize \textit{neighbors} of nodes in $\G(d)$, not the $\G(d)$ nodes themselves. For example, $x_{\nn}(d)$ is the average activity of a randomly selected node $j$, given that this node is a neighbor of $i \in \G(d)$. Hence (\ref{avXd}) averages over $i$, conditional on $i$'s degree, while (\ref{avXnnd}) averages over $i$'s \textit{neighbors} conditional on $i$'s degree. The former, we emphasize, captures a direct dependence on the node's degree, while the latter is indirect, since the conditionality is on the neighbor's degree.    

To express these conditional averages we use 

\begin{eqnarray}
X(d) &=& \av{X|d} = \av{X} f_X(d)
\label{fXd}
\\[5pt]
X_{\nn}(d) &=& \av{X|d}_\odot = \av{X}_\odot f_{X,\odot}(d)
\label{fXodotd}
\end{eqnarray}

where the functions $f_X(d)$ and $f_{X,\odot}(d)$ help link between the ensemble averages $\av X, \av X_\odot$ and and the $d$-conditioned averages $\av{X|d}$ and $\av{X|d}_\odot$. We, therefore arrive at four distinct forms of averaging:\ (i) $\av X$ - the typical value of observable $X$ of a randomly selected node; (ii) $\av X_\odot$ - the typical value of observable $X$ of a randomly selected neighbor; (iii) $\av{X|d}$ - the typical value of $X$ of a randomly selected node within $\G(d)$; (iv) $\av{X|d}_\odot$ - the typical value of $X$ of a randomly selected node, who has a neighbor within $\G(d)$. 

Averages (i) and (ii) above represent \textit{ensemble averages} and (iii) captures the direct dependence of observable $X_i$ on $d_i$. To evaluate (iv) via (\ref{fXodotd}) we list below several approaches by which to approximate $f_{X,\odot}(d)$:\

\textbf{Mean-field}.\
The classic mean-field approximation assumes that all components have a statistically similar surrounding. This translates to $f_{X,\odot}(d) \approx 1$ in (\ref{fXodotd}), namely that $X_{\nn}(d)$ is approximately independent of $d$. Under this approximation, individual nodes may be diverse, and hence $X(d)$ may be strongly dependent on $d$, yielding a potentially broadly distributed $X$ across all nodes. However, the neighborhoods are assumed to be statistically uniform, and hence all nodes are, on average, exposed to a similar set of neighbors. In simple terms, consider $i \in \G(d)$ and $j \in \G(d^\prime)$, where $d \ne d^\prime$. Node $i$'s observable $X_i$ is, on average $X(d)$, potentially distinct from $j$'s $X(d^\prime)$. Yet, $i$'s $k_i$ neighbors and $j$'s $k_j$ neighbors are both extracted from the same statistical pool, and therefore, regardless of the individual differences between $X_i$ and $X_j$, their \textit{neighborhoods} are, on average, the same, \textit{i.e}.\ $X_{\nn}(d) \approx X_{\nn}(d^\prime)$.

This approximation is exact in the limit where degree-correlations vanish, \textit{e.g}., the configuration model \cite{Newman2010} framework, where, indeed, the information about $i$'s degree has no bearing on the statistical properties of its neighbor $j$. It thus allows us to replace conditional averages $X_{\nn}(d)$ by the relevant ensemble average $\av{X}_\odot = X_{\nn}$. We emphasize that this approximation only neglects the indirect dependencies ($\odot$), but continues to enable the individual node diversity via $f_X(d)$, which may depend quite strongly on $d$.  

\textbf{\color{blue} Assumption 5}.\ 
In our derivation we employ a significantly weaker assumption than the mean-field above. While mean-field implied $f_{X,\odot}(d) \approx 1$, we, instead, assume that 

\begin{equation}
f_{X,\odot}(d) \sim F(d) d^\alpha,
\label{fXodotdalpha}
\end{equation}

where $F(d)$ is sub-polynomial, \textit{e.g}., $F(d) \sim \log(d)$, complemented by a polynomial dependence with a leading exponent $\alpha$. The exact structure of (\ref{fXodotdalpha}) depends on the specific observable $X$ and on the detailed weighted network topology, which determines the level of degree-correlations in the system, \textit{i.e}.\ how much it deviates from \textit{mean-field}. Specifically, in case $alpha = 0$, we have $f_{X,\odot}(d) \sim F(d)$, sub-polynomial. This represent \textit{weak degree-correlations}, in which $f_{X,\odot}(d) \ne 1$ (as in the mean-field approximation), but still, in the limit of large $d$, it does not \textit{scale} with $d$. 

Our derivation in the following sections can treat both strong ($\alpha \ne 0$) and weak ($\alpha = 0$) degree-correlations by introducing $\alpha$ where relevant. The specific value of $\alpha$, however, for any given observable $X$ can only be extracted from numerical/empirical data, as we have no analytical basis for \textit{a priori predicting} $\alpha$. Therefore, where relevant, we measure $f_{X,\odot}(d)$ explicitly, from each of our networks/dynamics to assess the weak/strong degree-correlations. 

\subsection{Parameters}
\label{SecAssumption6}

\textbf{\color{blue} Assumption 6}.\
The parameters $\f_i$ may be, potentially, distributed across all nodes. In our derivation we assume that the assignment of these parameters is done at random. Therefore, we expect negligible correlations between $\f_i$ and $A,G$. As a result, $i$'s parameters $\f_i$ are statistically independent of $i$'s degree $d_i$. Consequently, if we consider the conditional average $\av{\f_i|d}$, carried out over nodes with an assigned degree $d$, it is, statistically, the same as $\av{\f_i}$, \textit{i.e}.\ the \textit{ensemble average}. As an example, which will become useful below, we can, specifically apply this to the coefficients of the Hahn expansion in (\ref{Hahn}), writing

\begin{equation}
\av{\m Cqn(\m \f qi)|d} = \av{\m Cqn(\f)}, 
\label{ParameterAv}
\end{equation}

taken to mean that if we average any of (\ref{Hahn})'s coefficients associated specifically with nodes in $\G(d)$ we obtain the same outcome as averaging over the entire node ensemble. In simple terms \textit{parameter}-wise nodes sampled from $\G(d)$ are statistically similar to those from $\G(d^\prime)$. 

\subsection{Additional approximations}
\label{SecAdditionalApproximations}

While the above description outlines our fundamental \textit{model assumptions}, in some instances we also use approximations to these assumptions that help us (i) advance analytically where we cannot analyze the exact system; (ii) offer a more concise derivation, avoiding overly complicated and cumbersome calculations:

\textbf{\color{blue} Mean-field}.\
In few specific steps during our derivation we approximate $\av{M_q(x)} \approx M_q(\av{x})$ (see Sec.\ \ref{SecM2odot}). This is exact in case $M_q(x)$ is linear, and justified if $x$ is narrowly distributed. Another option, which occurs quite frequently in many relevant models, is that $M_q(x)$ is sub-linear, for example, the saturating function $M_2(x \to \infty) \to 1$ observed in many interactions. In this latter case, even if $x$ is broadly distributed, $M_q(x)$ is still bounded, and hence $\av{M_q(x)}$ can be evaluated via mean-field. We discuss the validity of this approximation in the relevant locations, and emphasize that, in most cases, it helps us avoid overly sophisticated notations and derivations, but, as our results indicate, it has little impact on the accuracy of our predictions.

\textbf{\color{blue} Star-approximation}.\
In Sec.\ \ref{SecPrincipleEigenvalue} we employ a star-approximation, simplifying $A$ into a single hub and spoke network. This is, of course, a crude simplification, needed only to extract the principal eigenvalue $\lambda$ (Eq.\ (8) of the main text), but unrelated to our derivation of the Jacobian $J$ itself. Hence the ensemble $\Ew$ is derived under Assumptions 1 - 6 above, and only $\lambda$ requires the star simplification. Due to the approximate nature of Sec.\ \ref{SecPrincipleEigenvalue}'s derivation, we accompany is by extensive numerical support, covering $\sim 10^4$ independently sampled Jacobian matrices.

%%%%%%%%%%%%%%%%%%%%%%%%%%%%%%%%%%%%%%%%%%%%%%%%%%%%%%%%%%%%%%%%%%%%%%%%%%%%%%%%%%%%% 
%%%%%%%%%%%%%%%%%%%%%%%%%%%%%%%%%%%%%%%%%%%%%%%%%%%%%%%%%%%%%%%%%%%%%%%%%%%%%%%%%%%%% 
{\color{blue} \rule{12cm}{1mm}}
\vspace{2mm}  	
\section{The Jacobian ensemble $\Ew$}
\label{SecJacobian}

To analyze stability we seek the structure of the Jacobian matrix $J$, as extracted from the system's specific nonlinear interaction mechanisms. We first rewrite Eq.\ (\ref{Eq3}) as

\begin{equation}
\dod{x_i}{t} = F_i \big( \mathbf{x}(t) \big), 
\label{Dynamics}   
\end{equation}

where

\begin{equation}
F_i \big( \mathbf{x}(t) \big) = 
M_0 \big( x_i(t), \m \f0i \big) + \g \sum_{j = 1}^{N}  
\m Aij M_1 \big( x_i(t), \m \f1i \big) \m Gij M_2 \big(x_j(t), \m \f2j \big),  
\label{Fix}
\end{equation}

and denote its fixed-point(s) by $\mathbf{x^*} = (x_1, \dots x_N)^{\top}$, omitting the $t$-dependence to capture their stationary state. These fixed-points are obtained by solving the equilibrium equation 

\begin{equation}
F_i(\mathbf{x^*}) = 0.
\label{FixedPoint1}
\end{equation}

To assess the dynamic stability of each of Eq.\ (\ref{FixedPoint1})'s solutions we track their response to small perturbations, via the Jacobian

\begin{equation}
\m Jij = \left. \dfrac{\partial F_i(\mathbf{x})}{\partial x_j} \right|_{\mathbf{x} = \mathbf{x}^*},
\label{Jij}
\end{equation}

whose structure we obtain below. Writing

\begin{equation}
J = (A - I) \otimes W 
\label{JQD}
\end{equation}
 
we treat separately the diagonal terms $\m Jii = - \m Wii$ and the off-diagonal terms $\m Jij = \m Aij \m Wij$ ($I$ represents the identity matrix).

\subsection{The fixed-points $\mathbf{x^*}$} 
\label{SecFixedPoint}

We consider systems of the form (\ref{Dynamics}) that exhibit at least one fully positive fixed-point $\mathbf{x^*}$. First, using Eq.\ (\ref{Fix}) we write 

\begin{equation}
M_0 (x_i,\m \f0i) + \g \sum_{j = 1}^{N} \m Aij M_1 (x_i,\m \f1i) \m Gij M_2 (x_j,\m \f2j) = 0,
\label{FixedPoint}
\end{equation} 

seeking the potentially multiple equilibrium solutions of the system. Next, we use (\ref{M2xOdot}) to express the sum on the r.h.s.\ of the equation, obtaining  

\begin{equation}
M_0 (x_i,\m \f0i) + M_1 (x_i, \m \f1i) \g d_i \Mi = 0,
\label{FixedPointi}
\end{equation}

a direct equation for $i$'s fixed-point value $x_i$. For certain dynamics Eq.\ (\ref{FixedPointi}) has a \textit{trivial} solution in which $M_0(x_i) = M_1 (x_i) = 0$. Most often this solution captures an inactive state in which all $x_i = 0$. Such solutions are treated separately in Sec.\ \ref{TrivialSolution}. Here we focus on the Jacobian around the non-trivial states of the system, where $M_0(x_i,\m \f0i) \ne 0$. 

For these non-trivial cases we rewrite (\ref{FixedPointi}) as

\begin{equation}
R_i(x_i) = \dfrac{1}{\Mi \g d_i} \equiv q_i,
\label{Rxi}
\end{equation}

where 

\begin{equation}
R_i(x_i) = R_i(x_i,\m \f0i,\m \f1i) = - \dfrac{M_1(x_i,\m \f1i)}{M_0(x_i,\m \f0i)}
\label{Rxi2}
\end{equation}

and $q_i$ defined in (\ref{Rxi}) is node $i$'s \textit{inverse degree}, whose value scales as $q_i \sim d_i^{-1}$. The function $R_i(x_i)$ is directly attainable from the system's dynamics, through $M_0(x_i,\m \f0i)$ and $M_1(x_i,\m \f1i)$. This function depends on $i$ through the parameters $\m \f0i,\m \f1i$, and hence $R_i(x_i)$ is potentially distinct from $R_j(x_j)$. 

We can now extract $x_i$ by inverting the function $R_i(x_i)$ in (\ref{Rxi}), providing us with

\begin{equation}
x_i = R_i^{-1}(q_i),
\label{xdRinv}
\end{equation} 

in which $i$'s fixed-point activity is described in terms of its inverse degree. In certain cases $R_i(x_i)$ in non-monotonic, and hence $R_i^{-1}(q_i)$ is ill-defined. This indicates that Eq.\ (\ref{FixedPoint}) has several solutions, capturing multiple fixed-points of the system. For example, in Fig.\ \ref{FigRInverse}a we illustrate a function $R(x)$ in which $R(x) = q$ has three distinct solutions, represented by the red, yellow and green dots. Therefore, $R^{-1}(x)$ assumes three separate values at $x = q$, formally, an undefined function (Fig.\ \ref{FigRInverse}b). To observe each of these solutions via (\ref{xdRinv}) we focus on the different \textit{branches} of $R(x)$ separately:\ first we plot $R(x)$. Then if it is non-monotonous, we identify its extremum points. This allows us to construct the different invertible branches of $R(x)$, for instance the one including only the maximum point (Branch 1, Fig.\ \ref{FigRInverse}c,d), the one including only the minimum point (Branch 2, Fig.\ \ref{FigRInverse}e,f) or the branch traversing through the intermediate points between these two extrema (Branch 3, Fig.\ \ref{FigRInverse}g,h). Each of these constructions \textit{is} invertible, and allows us to analyze all fixed-points independently using Eq.\ (\ref{xdRinv}).

%%%%%%%%%%%%%%%%%%%%%%%%%%%%%%%%%%%%%%%%%%%%%%%%%%%%%%%%%%%%%%%%%%%%%%%%%%%%%%%%%% 
%%%%%%%%%%%%%%%%%%%%%%%%%%%%%%%%%%%%%%%%%%%%%%%%%%%%%%%%%%%%%%%%%%%%%%%%%%%%%%%%%% 
\begin{figure}
\includegraphics[width=16cm]{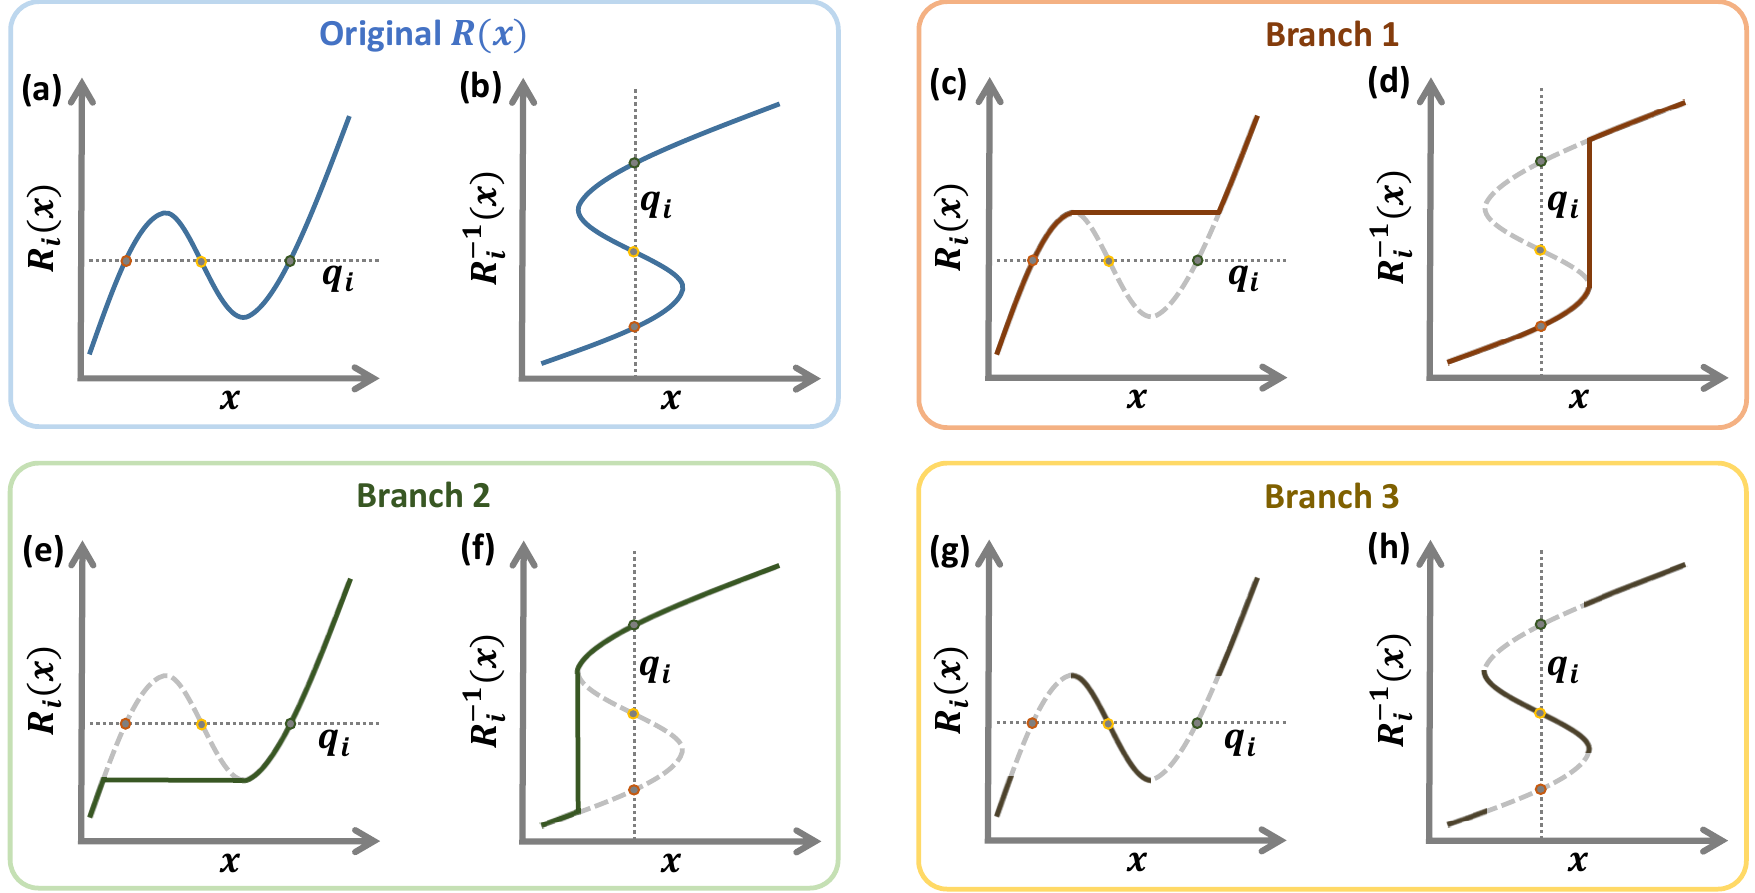}
\vspace{-7mm}
\caption{\footnotesize \color{blue} \textbf{Inverting a non-monotonic $R(x)$}.\
(a) In case $R(x)$ in (\ref{Rxi}) is non-monotonic its inverse function is ill-defined. 
(b) This leads in Eq.\ (\ref{xdRinv}) to multiple solutions (orange, yellow, green), describing a potentially multi-stable system. To treat this we construct three functions, corresponding to the different branches of $R(x)$:\
(c)-(d) Branch 1, in which the only solution to (\ref{xdRinv}) is the orange fixed-point;
(e)-(f) Branch 2, providing the green fixed-point;
(g)-(h) Branch 3, for the intermediate yellow fixed-point.   
}
\label{FigRInverse}
\end{figure}
%%%%%%%%%%%%%%%%%%%%%%%%%%%%%%%%%%%%%%%%%%%%%%%%%%%%%%%%%%%%%%%%%%%%%%%%%%%%%%%%%% 
%%%%%%%%%%%%%%%%%%%%%%%%%%%%%%%%%%%%%%%%%%%%%%%%%%%%%%%%%%%%%%%%%%%%%%%%%%%%%%%%%% 

\subsection{Diagonal terms $W_{ii}$ and $W(d)$}
\label{SedDiagonal}

Using (\ref{Fix}) and (\ref{Jij}) we can now write the diagonal Jacobian terms as
		
\begin{equation}
\m Wii = \left. \frac{\partial F_i({\bf x})}{ \partial x_i} \right|_{\bf x=x^*}
= \left. \left( M_0^{\prime}(x_i,\m \f0i) + M_1^{\prime}(x_i,\m \f1i) \g
\sum_{j = 1}^{N} \m Aij \m Gij M_2(x_j,\m \f2j) \right) \right|_{\bf x=x^*},
\label{Dii}
\end{equation}
		
where $M_0^{\prime}(x) = \partial M_0 / \partial x$ and $M_1^{\prime}(x) = \partial M_1 / \partial x$. Once again, we use (\ref{M2xOdot}) to express the sum on the r.h.s., obtaining

\begin{equation}
\m Wii = M_0^{\prime}(x_i,\m \f0i) \Big|_{\bf x=x^*} + 
\g d_i M_1^{\prime}(x_i,\m \f1i) \Big|_{\bf x=x^*} \Mi,
\label{Dii2}
\end{equation}

in which we condense the summation over $M_2(x_j, \m \f2j)$ into the neighborhood average $\Mi$. Finally, expressing the fixed-point $\mathbf{x^*}$ via (\ref{xdRinv}) and substituting the inverse degree $q_i$ in place of $(\g \Mi d_i)^{-1}$, as per Eq.\ (\ref{Rxi}), we write

\begin{equation}
\m Wii = M_0^{\prime}\big(R_i^{-1}(q_i),\m \f0i \big) + 
\dfrac{1}{q_i} M_1^{\prime}\big(R_i^{-1}(q_i),\m \f1i \big).
\label{Dii2}
\end{equation}

Next we use the definition of $R_i(x_i)$ in (\ref{Rxi2}) to write $M_0(x_i,\m \f0i) = - M_1(x_i,\m \f1i) / R_i(x_i)$, which provides

\begin{equation}
M_0^{\prime}(x_i,\m \f0i) = - \dfrac{M_1^{\prime}(x_i,\m \f1i)}{R_i(x_i)} + 
\dfrac{M_1(x_i,\m \f1i) R_i^{\prime}(x_i)}{R_i^2(x_i)}.
\label{M0prime}
\end{equation}

Substituting (\ref{M0prime}) into (\ref{Dii2}) and replacing $x_i$ by $R_i^{-1}(q_i)$ we obtain

\begin{equation}
\m Wii = - \dfrac{M_1^{\prime}\big( R_i^{-1}(q_i), \m \f1i \big)}{q_i} + 
\dfrac{M_1\big( R_i^{-1}(q_i), \m \f1i \big) R_i^{\prime}\big( R_i^{-1}(q_i) \big)}{q_i^2} + \dfrac{M_1^{\prime}\big( R_i^{-1}(q_i), \m \f1i \big)}{q_i},
\label{Dk2}
\end{equation}
 
where we used the fact that $R_i(R_i^{-1}(q_i)) = q_i$ to obtain the $q_i$ and $q_i^2$ terms in the denominators. Collecting all terms, we arrive at

\begin{equation}
\m Wii = \dfrac{1}{q_i^2} Y_i \big( R_i^{-1}(q_i), \m \f0i, \m \f1i \big),
\label{Dk3}
\end{equation} 

where $Y_i(x) = M_1(x, \m \f1i) R_i^{\prime}(x)$. 

To obtain the asymptotic scaling of $\m Wii$ with $d_i$ we use the Hahn expansion to express $Y_i(x)$ in the form of a power series, as shown in (\ref{Hahn}). Seeking the asymptotic limit $d_i \rightarrow \infty$, we derive our Hahn expansion around $q_i \sim d_i^{-1} \rightarrow 0$. Hence, we write

\begin{equation}
Y_i \big( R_i^{-1}(q_i), \m \f0i, \m \f1i \big) = 
\sum_{n = 0}^{\infty} B_n(\m \f0i, \m \f1i) q_i^{\Phi_n},
\label{YLaurent}
\end{equation}
		
and below, examine the leading terms only. 

Following Outcome 1 in Sec.\ \ref{SecAssumption1} we assert that in (\ref{YLaurent}) the coefficients $B_n = B_n(\m \f0i, \m \f1i)$, \textit{i.e}.\ depending on the specific system parameters $\f$. These coefficients are therefore node-specific, since generally $\m \f qi \ne \m \f qj$. The powers $\Phi_n$, however, are independent of $\f$, and are therefore uniform for all nodes. Indeed, $Y_i(x)$  is directly constructed from $M_q(x_i,\m \f qi)$ through basic function operations:\ multiplication ($M_1 R^\prime$), division ($M_1/M_0$), inversion ($R^{-1}$) and derivation ($R^\prime$). As explained in Outcome 1, each of these operations preserves the separation between coefficients and powers. Hence $\Phi_n$ are determined by $\m \Gamma qn$ in (\ref{Hahn}), but remain independent of the coefficients $\m Cqn$. Consequently, since $\m \Gamma qn$ are node independent, so are $\Phi_n$. 

Taking the limit $q_i \to 0$ we keep only the leading power $\Phi_0$ in (\ref{YLaurent}), \textit{i.e}.\ $Y_i (R_i^{-1}(q_i),\m \f0i,\m \f1i) \approx B_0(\m \f0i,\m \f1i) q_i^{\Phi_0}$. This in Eq.\ (\ref{Dk3}) predicts

\begin{equation}
\m Wii = B_0(\m \f0i,\m \f1i) q_i^{-\mu},
\label{Wiiqimu}
\end{equation} 
   
where

\begin{equation}
\mu = 2 - \Phi_0. 
\label{alpha}
\end{equation}

Equation (\ref{Wiiqimu}) provides the dependence of the diagonal Jacobian weight $\m Wii$	on $i$'s inverse degree $q_i$; it is exact up to higher powers $q_i^{\Phi_1},q_i^{\Phi_2},\dots$, which vanish under $q_i \rightarrow 0$. To complete our derivation we seek $W(d) = \av{\m Wii|d}$, namely the conditional average over $\m Wii$ given that $i \in \G(d)$. Using (\ref{avXd}) we express this average as

\begin{equation}
W(d) = \dfrac{1}{|\G(d)|} \sum_{i \in \G(d)} \m Wii = 
\dfrac{1}{|\G(d)|} \sum_{i \in \G(d)} B_0(\m \f0i,\m \f1i) q_i^{-\mu},
\label{W0d1}
\end{equation}  

where in the last step, we expressed $\m Wii$ via Eq.\ (\ref{Wiiqimu}). Next we recall Assumption 6, stating that the parameters, here $\m \f0i$ and $\m \f1i$, are randomly assigned, independently of $d_i$. This allows us, following Eq.\ (\ref{ParameterAv}), to extract the coefficient $B_0(\m \f0i,\m \f1i)$ from the summation in (\ref{W0d1}), and replace it by the ensemble average $\av{B_0(\f)}$. We also reintroduce the complete expression for $q_i$ in (\ref{Rxi}), thus rewriting $W(d)$ as

\begin{equation}
W(d) = \av{B_0(\f)} \dfrac{1}{|\G(d)|} \sum_{i \in \G(d)} 
\big( \g \Mi d_i \big)^{\mu}.
\label{W0d2}
\end{equation}    

To advance further we note that:\ (i) $\g$ is a constant, and (ii) by definition, all $i \in \G(d)$ have $d_i = d$ (or more accurately $d_i \in (d,d + \delta d)$). This allows us to extract these two factors out of the summation, and further simplify (\ref{W0d2}) into the form

\begin{equation}
W(d) = \av{B_0(\f)} \g^\mu d^\mu \dfrac{1}{|\G(d)|} \sum_{i \in \G(d)} 
\Mi^\mu = 
\Big( \av{B_0(\f)} \g^\mu \av{M^\mu | d}_\odot \Big) d^\mu,
\label{W0d3}
\end{equation}    

where, in the final step, we used the neighborhood conditional average defined in (\ref{avXnnd}), to express the sum over $\Mi$. We can now use Eq.\ (\ref{fXodotd}) to write this conditional average as 

\begin{equation}
\av{M^\mu | d}_\odot = \Mmu f_{M,\odot}(d),
\label{MmufModot}
\end{equation}

where $\Mmu$ is the network ensemble average, and $f_{M,\odot}(d) = \av{M^\mu | d}_\odot / \Mmu$ accounts for $\av{M^\mu | d}_\odot$'s degree conditionality. Collecting all terms we arrive at

\begin{equation}
W(d) = \Big( \av{B_0(\f)} \g^\mu \Mmu \Big) f_{M,\odot}(d) d^\mu,
\label{W0d4}
\end{equation}

in which the prefactor (in parenthesis) comprises all terms that do not contribute to the degree dependence. Next, to complete our derivation, we seek the value of $\Mmu$, which we recall is equal to $\av{M_2^\mu(x)}_\odot$, the average of $M_2^\mu(x_j,\m \f2j)$ over all \textit{neighbor} nodes $j$.

\subsubsection{Evaluating $\av{M_2^\mu(x)}_{\odot}$}
\label{SecM2odot}

Our derivation of $W(d)$ indicates the importance of the neighborhood average

\begin{equation}
\Mmu = 
\dfrac{1}{N} \sum_{i = 1}^N \av{M_2^\mu(x)}_{i,\odot} = 
\dfrac{1}{N} \sum_{i = 1}^N \dfrac{1}{d_i} \sum_{j = 1}^N \m Aij \m Gij M_2^\mu(x_j),
\label{M2odot}
\end{equation}

capturing the mean value of $M_2^\mu(x)$ over all neighborhoods. To link (\ref{M2odot}) to the weighted network topology $A,G$ we use the mean-field approximation of Sec.\ \ref{SecAdditionalApproximations}. We note that throughout our derivation this is the only component where we employ this approximation. Indeed, $\Mmu$, as opposed to, \textit{e.g}., $x_i$ or $W(d)$, that were calculated above, is an aggregated function, capturing an ensemble average. It is therefore natural to evaluate this function using a mean-field approach that builds on averaging the behavior of Eq.\ (\ref{Dynamics}).

 We first define the weighted nearest neighbor activity as

\begin{equation}
x_{\nn} = \av{x}_{\odot} = \dfrac{1}{N} \sum_{i = 1}^N 
\dfrac{1}{d_i} \sum_{j = 1}^{N} \m Aij \m Gij x_j,
\label{xodot}
\end{equation}

and its corresponding nearest neighbor weighted degree as

\begin{equation}
\knn = \av{d}_{\odot} = \dfrac{1}{N} \sum_{i = 1}^N 
\dfrac{1}{d_i} \sum_{j = 1}^{N} \m Aij \m Gij d_j.
\label{kappa}
\end{equation}

Hence, the average nearest neighbor node is characterized by activity $x_{\nn}$ and degree $\knn$. While $x_{\nn}$ depends on the system's dynamics (\ref{Dynamics}), $\knn$ is fully determined by the weighted topology $A \otimes G$ through the network's weighted degree density $P(d)$. In the absence of degree correlations and under a symmetric $A,G$ we have \cite{Gao2016}

\begin{equation}
\knn = \dfrac{\av{d^2}}{\av{d}},
\label{k2overk}
\end{equation}

where $\av{d^n}$ is the $n$th moment of $P(d)$. For a homogeneous network in which $P(d)$ is bounded this predicts $\knn \approx \av d$, however, if the network is highly heterogeneous, \textit{i.e}.\ $P(d)$ is fat-tailed, we have $\knn \gg \av d$. In case the network is not symmetrical, \textit{i.e}.\ a directed $\m Aij$ or asymmetric weights $\m Gij \ne \m Gji$, we distinguish between the in/out degrees of all nodes as

\begin{equation}
\begin{array}{cc}
d_{i,\rm in} = \displaystyle \sum_{j = 1}^N \m Aij \m Gij;
&
d_{i,\rm out} = \displaystyle \sum_{j = 1}^N \m Aji \m Gji
\end{array},
\label{Sinout}
\end{equation} 

obtaining \cite{Gao2016}

\begin{equation}
\knn = \dfrac{\av{d_{\rm in} d_{\rm out}}}{\av{d}},
\label{SinOutOverS}
\end{equation}

incorporating a mixed moment - the average over the product $d_{i,\rm in} d_{i,\rm out}$.

More generally, in case the network also features measurable degree-correlations we use the conditional density function $P(d|d^{\prime})$ to express the probability density to observe $d_i \in (d, d + \delta d)$, given that $i$'s neighbor has degree $d^{\prime}$. This allows us to write \cite{Boccaletti2006}

\begin{equation}
\knn = \int_{d_{\rm min}}^{\infty} \int_{d_{\rm min}}^{\infty} d P(d|d^{\prime})P(d^{\prime}) 
\dif d \dif d^{\prime},
\label{kappaDegCorr}
\end{equation}

accounting for the potential degree dependence between neighboring nodes. In all cases, from (\ref{k2overk}) to the more general (\ref{kappaDegCorr}), under extreme degree-heterogeneity, $\knn$ may diverge with system size as \cite{Newman2010}

\begin{equation}
\knn \sim N^{\beta},
\label{knnNBeta}
\end{equation} 

with $\beta$ determined by the network/weight heterogeneity. 

To link $\Mmu$ to $\knn$ and $x_{\nn}$ we use the mean-field formalism presented in Ref.\ \cite{Gao2016}, allowing to use to write a direct equation for a \textit{nearest neighbor} node. While the precise derivation and validity limits of this formalism are detailed therein, here, for conciseness, we use a brief, shorthand, derivation, outlining all the crucial approximations along the path. We begin by writing our fixed-point condition in the form of (\ref{FixedPoint1}), namely

\begin{equation}
F_i(\x^*) = 0.
\label{MFFixedPoint}
\end{equation} 

We then apply our nearest neighbor averaging to write

\begin{equation}
\av{F_i(\x^*)}_\odot = 0, 
\end{equation}

which taking $F_i(\x^*)$ from Eq.\ (\ref{FixedPointi}), provides

\begin{equation}
\av{M_0(x_i)}_\odot + g \av{M_1(x_i) d_i \Mi}_\odot = 0
\end{equation}

We can employ the mean-field approximation to break down the second average on the l.h.s.\ and write it as a product of three separate averages, \textit{i.e}.\ we neglect correlations between the terms. This brings us to

\begin{equation}
\av{M_0(x_i)}_\odot + g \av{M_1(x_i)}_\odot \av{d_i}_\odot \av{\Mi}_\odot = 0,
\end{equation}

which we can simplify term by term:\ first we use, again, the mean-field approximation of Sec.\ \ref{SecAdditionalApproximations} to write $\av{M_0(x_i)}_\odot \approx M_0(\av x_\odot) = M_0(x_{\nn})$ and, analogously $\av{M_1(x_i)}_\odot \approx M_1(x_{\nn})$. Next, we note that $\av{d_i}_\odot$ is, by definition equal to $\knn$. Finally if we write $\av{\Mi}_\odot$ explicitly we obtain

\begin{equation}
\av{\Mi}_\odot = 
\dfrac{1}{N} \sum_{m = 1}^N \dfrac{1}{d_m} \sum_{j = 1}^N \m Amj \m Gmj \av{M_2(x_j)}_{j,\odot},
\end{equation} 

an average over all neighbors' neighbors, which, under our mean-field assumption is identical to averaging over all neighbors. Hence, for the last term we write $\av{\Mi}_\odot = \av{M_2(x_j)}_\odot \approx M_2(x_{\nn})$, again employing Sec.\ \ref{SecAdditionalApproximations}'s mean-field assumption. Collecting all terms this brings us to  

\begin{equation}
M_0(x_{\nn}) + \g \knn M_1(x_{\nn})M_2(x_{\nn}) = 0,
\label{Gao}
\end{equation} 

a self-consistent equation for the average neighbor (degree $\knn$) activity $x_{\nn}$;\ we once again refer the reader to Ref.\ \cite{Gao2016} for a more formal derivation of (\ref{Gao}). Using $R(x_{\nn}) = -M_1(x_{\nn})/M_0(x_{\nn})$ as in (\ref{Rxi}) we arrive at

\begin{equation}
Z(x_{\nn}) = \dfrac{1}{\g \knn} \equiv q_{\nn},
\label{Zchi}
\end{equation}

where $Z(x) = R(x)M_2(x)$ is a dynamic function, fully determined by $M_0(x),M_1(x),M_2(x)$ in (\ref{Eq3}), and $q_{\nn}$ is the inverse nearest neighbor degree.

By inversion we obtain

\begin{equation}
x_{\nn} = Z^{-1}(q_{\nn}),
\label{Zchi2}
\end{equation}

and hence

\begin{equation}
M_2(x_{\nn}) = M_2 \big( Z^{-1}(\q_{\nn}) \big).
\label{M2chi}
\end{equation}

Similarly to $R_i(x_i)$ in (\ref{Rxi}) the dynamic function $Z(x)$ may also be non-invertible in case the system has multiple fixed-points. We treat this by considering the different branches of $Z(x)$, following a similar analysis to the one shown in Fig.\ \ref{FigRInverse}. Below, in Sec.\ \ref{SecRegulatory} we show in detail how we treat such non-ivertibility, which arises naturally during our analysis of Regulatory dynamics. 
 
To obtain the asymptotic scaling of $M_2(x_{\nn})$ on $\knn$ we use the Hahn expansion to express (\ref{M2chi}) in the form of a power series around $\q_{\nn} \rightarrow 0$, \textit{i.e}.\ large $\knn$. Hence we write

\begin{equation}
M_2 \big( Z^{-1}(\q_{\nn}) \big) = \sum_{n = 0}^{\infty} G_n \q_{\nn}^{\Psi_n},
\label{M2Laurent}
\end{equation}

where $\Psi_n$, once again, is a set of real powers in ascending order with $n$. In the limit of large $\knn$ (small $\q_{\nn}$) the expansion in (\ref{M2Laurent}) is dominated by the leading power $\Psi_0$, predicting that

\begin{equation}
M_2(x_{\nn}) \sim \knn^{\xi},
\label{M2xi}
\end{equation}

where 

\begin{equation}
\xi = -\Psi_0.
\label{kappaxi}
\end{equation}

As in the case of $Y_i(R^{-1}(q_i)$ in (\ref{YLaurent}), also here, thanks to Outcome 1 of Sec.\ \ref{SecAssumption1} the powers $\Psi_n$ are directly linked to the powers $\m \Gamma qn$ of the dynamic functions $M_q(x)$ in (\ref{Hahn}). Indeed, to arrive at the composite function $M_2(Z^{-1}(x))$, we used standard operations of division ($R = -M_1/M_0$), multiplication ($Z = RM_2$), inversion ($Z^{-1}(x)$) and finally composition ($M_2(Z^{-1}(x))$) - all maintaining the separation of powers and coefficients. 

To complete our derivation we refer back to $\Mmu = \av{M_2^\mu(x)}_\odot$. Through our mean-field approximation we write $\Mmu \approx M_2^\mu(x_{\nn})$, which using (\ref{M2xi}) provides $\Mmu \sim \knn^{\xi \mu}$. With this at hand we now return to $W(d)$ in (\ref{W0d4}) and replace the term $\Mmu$ with $\knn^{\xi \mu}$, obtaining

\begin{equation}
W(d) \sim \Big( \av{B_0(\f)} \g^\mu \Big) \knn^{\xi \mu} f_{M,\odot}(d) d^\mu.
\label{W0d5}
\end{equation} 

One more step remains to fully characterize $W(d)$, extracting the unknown function $f_{M,\odot}(d)$. Therefore, to complete our analysis we seek to evaluate $f_{M,\odot}(d)$, which, according to Eq.\ (\ref{MmufModot}), represents the ratio

\begin{equation}
f_{M,\odot}(d) = \dfrac{\av{M^\mu | d}_\odot}{\Mmu}
\label{fXodotd2}
\end{equation}

between the degree conditional average $\av{M^\mu | d}_\odot$ and the ensemble average $\Mmu$. In accordance with Assumption 5 (Eq.\ (\ref{fXodotdalpha}) of Sec.\ \ref{SecTopology}) we examine whether we observe a polynomial dependence of the form $f_{M,\odot}(d) \sim F(d) d^\alpha$ or, alternatively, only the sub-polynomial $F(d)$ with $\alpha = 0$. Therefore, in Fig.\ \ref{FigFk} we extract $f_{M,\odot}(d)$ numerically, by simulating each of our dynamical systems, and calculating both $\av{M^\mu | d}_\odot$ and $\Mmu$ - the first by averaging the value of $M_2^\mu(x_i)$ over all neighborhoods surrounding a degree $d$ node, and the second by averaging over \textit{all} neighborhoods, independently of degree. Taking the ratio $\av{M^\mu | d}_\odot / \Mmu$ we obtain, numerically, the precise form of $f_{M,\odot}(d)$, for our seven models, each with its five underlying networks ($35$ systems altogether). Quite consistently, we find that $f_{M,\odot}(d)$ is sub-polynomial, \textit{i.e}.\ $\alpha = 0$, and, in fact, can be well-approximated by $f_{M,\odot}(d) \approx 1$. This indicates that with respect to $\Mmu$ our weak-dependency assumption (sub-polynomial $f_{M,\odot}(d)$), and, in fact, even the stronger mean-field
approximation ($f_{X,\odot}(d) \approx 1$) can capture, quite accurately, the system's dynamics.

%%%%%%%%%%%%%%%%%%%%%%%%%%%%%%%%%%%%%%%%%%%%%%%%%%%%%%%%%%%%%%%%%%%%%%%%%%%%%%%
%%%%%%%%%%%%%%%%%%%%%%%%%%%%%%%%%%%%%%%%%%%%%%%%%%%%%%%%%%%%%%%%%%%%%%%%%%%%%%%
\begin{figure}[t]
\includegraphics[width=16cm]{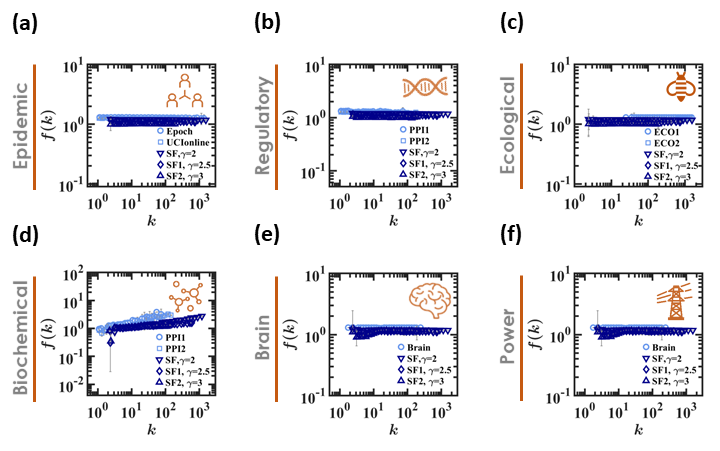}
\vspace{-10mm}
\caption{\footnotesize \color{blue} \textbf{Evaluating the degree correction function $f_{M,\odot}(d)$}.\ We used Eq.\ (\ref{fXodotd2}) to numerically evaluate $f_{M,\odot}(d) = \av{M^\mu | d}_\odot / \Mmu$, capturing the role of degree-correlations on the average neighbor activity. Results were obtained for each of our dynamic models implemented on both model and relevant empirical networks. In all cases we find that $f_{M,\odot}(d)$ is largely independent of $d$, roughly following $f_{M,\odot}(d) \sim 1$. Consequently, this correction to the mean-filed assumption $\av{X|d}_\odot \approx \av{X}_\odot$) has a negligible impact on our predicted scaling patterns.
}
\label{FigFk}
\end{figure}
%%%%%%%%%%%%%%%%%%%%%%%%%%%%%%%%%%%%%%%%%%%%%%%%%%%%%%%%%%%%%%%%%%%%%%%%%%%%%%%
%%%%%%%%%%%%%%%%%%%%%%%%%%%%%%%%%%%%%%%%%%%%%%%%%%%%%%%%%%%%%%%%%%%%%%%%%%%%%%%

This outcome, we emphasize, is not at all surprising. Indeed, the meaning of $\av{X|d}_\odot$, as defined in (\ref{avXnnd}), is the average of $X_j$ carried our over the \textit{neighbors} of $i$ ($\m Aij = 1$), under the condition that $i$'s weighted degree is around $d$ ($i \in \G(d)$). The crucial point is that this condition is on $i$, while the averaging is on $i$'s neighborhood, not on $i$ itself. Therefore, the information that $i \in \G(d)$ has only an indirect influence on the value of $X_j$, when averaged over $i$'s $k_i$ nearest neighbors. This indirect effect underlies the observed weak (sub-polynomial) dependence of $\av{X|d}_\odot$ on $d$.   

We can now characterize the different factors that shape $W(d)$ in (\ref{W0d5}). The first terms in the parenthesis depend on the global parameters $\f,\g$, and hence we can express it implicitly via the coefficient $C(\f,g)$. Following is the scaling with $\knn$, which is a global \textit{network} parameter, determined by $A \otimes G$, multiplying all diagonal terms, irrespective of $d$. This brings us to the last two terms that explicitly depend on $d$:\ $f_{M,\odot}(d)$ which we found to have a negligible effect, and $d^\mu$, which, in the limit of large $d$ dominates the scaling of $W(d)$. Taken together this provides

\begin{Frame}
\begin{equation}
W(d) \sim C(\f,\g) \knn^{\xi \mu} d^{\mu}, 
\label{Dkalpha}
\end{equation}
\end{Frame}
\vspace{-3mm}	
where $\mu$ and $\xi$ are taken from (\ref{alpha}) and (\ref{kappaxi}), respectively. Using our Jacobian structure $J = (A - I) \otimes W$, we construct the diagonal of $J$ as

\begin{equation}
\m Jii = - W(d_i),
\label{JiiWdi}
\end{equation}

precisely recovering Eq.\ (5) of the main text; see our more detailed discussion of this and other related points in Sec.\ \ref{SecJijPuzzle}. 

Equation (\ref{JiiWdi}) describes our ensemble approximation:\ the \textit{real} Jacobian diagonal terms are provided by (\ref{Dii}), which is exact, and may be potentially distinct even for nodes with identical degrees. These \textit{exact} terms are measured numerically and represented by symbols in Fig.\ 3 of the main text. Our \textit{analytically predicted} Jacobians, on the other hand, approximate these exact terms by estimating each diagonal entry via (\ref{JiiWdi}). This evaluates $\m Jii$ by substituting $i$'s weighted degree $d_i$ into (\ref{Dkalpha}), yielding an identical entry for all nodes of similar degree. Such approximation is designed to capture $\m Jii$'s ensemble average, namely 

\begin{equation}
- W(d) = \dfrac{1}{|\G(d)|} \sum_{i \in \G(d)} \m Jii,
\label{AvJii}
\end{equation}    

the average diagonal Jacobian entry for nodes of degree $d_i \in (d, d + \delta d)$. This analytical construction is represented by the orange solid lines in Fig.\ 3 of the main text, and shown to accurately capture the exact $J$ (blue symbols).

\subsection{The off-diagonal terms $\m Wij$ and $W(d_1,d_2)$}
\label{SecOffDiagonal}

\newcommand{\W}{\m {\widetilde W}ij}
\newcommand{\Ws}{\widetilde W}

The off-diagonal Jacobian terms are given by

\begin{equation}
\m Wij = \left. \frac{\partial F_i({\bf x})}{ \partial x_j} \right|_{\bf x=x^*}
= \left. \dfrac{\partial}{\partial x_j} \left( M_0(x_i, \m \f 0i) + M_1(x_i, \m \f 1i) 
\g \sum_{j = 1}^{N} \m Aij \m Gij M_2(x_j, \m \f 2j) \right) \right|_{\bf x=x^*},
\label{Qij}
\end{equation}

which after collecting only the terms that explicitly depend on $x_j$ reduces to

\begin{equation}
\m Wij = M_1(x_i,\m \f1i) \g \m Aij \m Gij M_2^{\prime}(x_j,\m \f2j) \Big|_{\mathbf{x = x^*}}.
\label{Qij2}
\end{equation}

Expressing the fixed-point activities via (\ref{xdRinv}) we write (\ref{Qij2}) in the form

\begin{equation}
\m \Ws ij = M_1 \big( R_i^{-1}(q_i),\m \f1i \big) 
\g \m Aij
M_2^{\prime} \big( R_j^{-1}(q_j),\m \f2j \big),
\label{Wij}
\end{equation}

where $\m \Ws ij = \m Wij / \m Gij$ is the \textit{weight-less} off-diagonal Jacobian entry. This naturally giver rise to two dynamic functions

\begin{eqnarray}
M_1 \big( R_i^{-1}(q_i),\m \f1i \big) &=& 
\sum_{n = 0}^{\infty} K_n(\m \f1i) \q_i^{\Pi_n}
\label{M1Rinv}
\\[5pt]
M_2^{\prime} \big( R_j^{-1}(q_j),\m \f2j \big) &=& 
\sum_{n = 0}^{\infty} L_n(\m \f2j) \q_j^{\Theta_n},
\label{M2Rinv}
\end{eqnarray} 

both constructed directly from $M_q(x)$. Once again, thanks to Outcome 1 (Sec.\ \ref{SecAssumption1}) the powers $\Pi_n,\Theta_n$ are parameter independent, and hence uniform for all nodes pairs $i,j$. Taking the limit of small $q_i,q_j$ (large $d_i,d_j$) we keep only the leading powers of (\ref{M1Rinv}) and (\ref{M2Rinv}), which in (\ref{Wij}) provides

\begin{equation}
\m \Ws ij = \g \m Aij K_0(\m \f1i) L_0(\m \f2j) q_i^{\Pi_0} q_j^{\Theta_0} + \cdots,
\label{Qk1k25}
\end{equation}

exact upto higher order terms $q_i^{\Pi_1},q_j^{\Theta_1},\dots$. Using $q_i = (\Mi \g d_i)^{-1}$ as per Eq.\ (\ref{Rxi}), we arrive at

\begin{equation}
\m \Ws ij = \g \m Aij K_0(\m \f1i) L_0(\m \f2j) 
\left( \dfrac{1}{\Mi \g d_i} \right)^{\Pi_0}
\left( \dfrac{1}{\av{M}_{j,\odot} \g d_j} \right)^{\Theta_0},
\label{Wij2}
\end{equation}

in which the dependence on $d_i,d_j$ is made explicit.

Similar to our calculation of $W(d)$ from $\m Wii$, also here we seek to average $\m \Ws ij$ over the set $\G(d_1,d_2) = \{i,j = 1,\dots,N | \m Aij = 1, i \in \G(d_1), j \in \G(d_2)\}$, namely the set of all interacting node pairs ($\m Aij = 1$) whose degrees are $d_i \in (d_1 + \delta d_1), d_j \in (d_2 + \delta d_2)$. Hence we write

\begin{equation}
W(d_1,d_2) = \dfrac{1}{|\G(d_1,d_2)|} \sum_{(i,j) \in \G(d_1,d_2)} \m \Ws ij,
\label{Wd1d2}
\end{equation}

providing the average magnitude of the (weight-less) Jacobian entry linked to $i,j$ pairs within $\G(d_1,d_2)$. Carrying out this average we reconstruct the steps that have already led us to $W(d)$ in (\ref{W0d5}). Hence, to avoid a lengthy repetition, we simply follow the analysis along the already established path from (\ref{W0d1}) to (\ref{W0d5}):\ (i) The coefficients $K_0(\m \f1i), L_0(\m \f2j)$ are replaced by their ensemble averages (Assumption 6); (ii) The parameter $\g$ can be extracted out from the average (it is constant); (iii) $d_i$ and $d_j$ are replaced by $d_1$ and $d_2$, respectively, since all nodes in the summation are in $\G(d_1,d_2)$; (iv) The neighborhood averages $\Mi$ and $\av{M}_{j,\odot}$ translate to the degree conditioned averages $\av{M|d_1}_\odot$ and $\av{M|d_2}_\odot$. These $d$-averages can be expressed via (\ref{MmufModot}) as

\begin{equation}
\begin{array}{ccc}
\av{M|d_1}_\odot = \M f_{M,\odot}(d_1)
& \,\,\,\,\,\,\, &
\av{M|d_2}_\odot = \M f_{M,\odot}(d_2)
\end{array},
\end{equation}

in which $\M$ is the ensemble average (independent of $d$) and $f_{M,\odot}(d)$ has been already shown to have a negligible contribution to the degree-scaling (Fig.\ \ref{FigFk}). Substitutions (i) - (iv) leave us with

\begin{equation}
W(d_1,d_2) = \Big( \g^{1 - \Pi_0 - \Theta_0} \av{K_0(\f)} \av{L_0(\f)} \Big) 
\M^{-\Pi_0 - \Theta_0} d_1^{-\Pi_0} d_2^{-\Theta_0},
\label{Wd1d22}
\end{equation}

where we have, indeed, neglected the terms associated with $f_{M,\odot}(d)$. 

As we are only interested in the asymptotic scaling with $d_1,d_2$ we neglect all terms that do not contribute the scaling, namely all terms in the parenthesis. We also use our analysis in Sec.\ \ref{SecM2odot}, where we have shown that $\M \sim \knn^\xi$ to express the relevant term in (\ref{Wd1d22}). This leads us to our final result 

\begin{equation}
W(d_1,d_2) \sim \knn^{\xi(\nu + \rho)} d_1^{\nu} d_2^{\rho}
\label{k1betak2zeta}
\end{equation}

where

\begin{equation}
\begin{array}{cc}
\nu = -\Pi_0, & \rho = -\Theta_0,
\end{array}
\end{equation}
		
and $\xi$ is taken from (\ref{kappaxi}).

\subsection{Piecing together the $\m Jij$ puzzle}
\label{SecJijPuzzle}

We now refer back to Eq.\ (\ref{JQD}) to bring together the diagonal $\m Jii$ in (\ref{JiiWdi}) and the off-diagonal $\m Wij$ derived above. First, we recall that for the off-diagonal terms our derivation provided us with $W(d_1,d_2)$, which is aggregated from the weight-less $\W$ of (\ref{Wij}). To obtain the actual off-diagonal terms of $J$ we must reintroduce the weights as $\m Wij = \m Gij W(d_i,d_j)$, namely multiply (\ref{k1betak2zeta}) by $\m Gij$ and replace $d_1,d_2$ by $d_i,d_j$ (this substitution $d_1 \to d_i,d_2 \to d_j$ is similar to the substitution $d \to d_i$ conducted in (\ref{JiiWdi}), see discussion that followed therein). Next, we piece all our results together to construct the complete Jacobian as appears in Eq.\ (\ref{JQD}), \textit{i.e}.\ $J = (A - I) \otimes W$, obtaining

\begin{equation}
\m Jij = \m Aij \m Wij - I_{ij} \m Wii = 
- I_{ij} C(\f,g) \knn^{\xi \mu} d_i^{\mu} +
\m Aij \m Gij \knn^{\xi(\nu + \rho)} d_i^{\nu} d_j^{\rho}.
\label{JijDiagOffDiag}
\end{equation}

The first term on the r.h.s.\ represents the (negative) diagonal entries, and second term captures the off-diagonal entries, which are non-zero only if $\m Aij = 1$. As we are only interested in the sign of the principle eigenvalue, but not in its specific magnitude, we have the degree of freedom to multiply $J$ by an arbitrary constant. We therefore normalize $J$ by $\knn^{-\xi(\nu + \rho)}$, providing

\begin{Frame}
\begin{eqnarray}
\m Jii &\sim& - C(\f,g) \knn^{\eta} d_i^{\mu} 
\label{JiiJij1}
\\[8pt]
\m Jij &\sim& d_i^{\nu} \m Aij \m Gij d_j^{\rho}
\label{JiiJij2}
\end{eqnarray}
\end{Frame}

for the diagonal and off-diagonal terms respectively, with $\eta = \xi(\mu - \nu - \rho)$ - recovering Eqs.\ (4) and (5) of the main text.

\begin{Frame}
Equations (\ref{JiiJij1}) and (\ref{JiiJij2}) describe the asymptotic structure of the diagonal and off-diagonal Jacobian terms, as extracted from the dynamics of Eq.\ (\ref{Dynamics}). The resulting $J$ is characterized by several distinct structural and dynamic inputs:\ $A$, the network topology, which determines the non-vanishing off-diagonal elements. Together with the link weights $G$ it also determines the degrees $d_i,d_j$ and the average neighbor degree $\knn$. The exponents 

\vspace{-6mm}
\begin{equation}
\Omega = (\eta, \mu, \nu, \rho)
\label{Omega}
\end{equation} 

are independent of the network topology, extracted from the dynamic functions $M_q(x)$. These exponents are universal in the sense that they do not depend of the specific model \textit{parameters} $\g,\f$, but rather on the powers $\m \Gamma qn$ in (\ref{Hahn}), grouping together all systems which follow the same \textit{model}, \textit{i.e}.\ Epidemic, Regulatory etc. The coefficient $C$, in contrast, is non-universal, and its value is determined by the specific rate-constants and time-scales driving Eq.\ (\ref{Dynamics}), for example, the distribution of $\f$ or the value of $\g$; here we do not attempt to predict the magnitude of this coefficient. In the limit of sufficiently large $d_i$ and $d_j$, and, where applicable - in the limit of large $\knn$, the specific finite value of $C$ has negligible impact on the principal eigenvalue of $J$ as we explicitly show in Sec.\ \ref{SecPrincipleEigenvalue}. Hence, in this limit, stability is asymptotically determined by the exponents $\Omega$, irrespective of $C$. The meaning is that the \textit{model} can be asymptotically stable or unstable, regardless of its specific \textit{parameters}.   
\end{Frame}

\subsubsection{Impact of $P(d)$ and $\knn$}
\label{ImpactPkKappa}

%%%%%%%%%%%%%%%%%%%%%%%%%%%%%%%%%%%%%%%%%%%%%%%%%%%%%%%%%%%%%%%%%%%%%%%%%%%%%%%%%%%%%%%%
%%%%%%%%%%%%%%%%%%%%%%%%%%%%%%%%%%%%%%%%%%%%%%%%%%%%%%%%%%%%%%%%%%%%%%%%%%%%%%%%%%%%%%%%
\begin{figure}[t]
\begin{Frame}
{\color{blue} {\textbf{The ensemble $\Ew$ summary}}}.\ 
Staring from Eq.\ (\ref{Dynamics}) we use $M_0(x),M_1(x)$ and $M_2(x)$ to construct the functions

\begin{equation}
\begin{array}{ccc}
R(x) = -\dfrac{M_1(x)}{M_0(x)}, & 
Y(x) = M_1(x) R^{\prime}(x), & 
Z(x) = R(x)M_2(x).
\end{array}
\label{FunctionsFrame}
\end{equation}

For each of these functions, we set the parameters $\m \f qi$ to their ensemble averages. The powers we extract below are, in any case, independnet of these parameters. From (\ref{FunctionsFrame}) we extract the four relevant power-series expansions

\begin{equation}
\begin{array}{cc}
M_2 \big( Z^{-1}(x) \big) = \displaystyle 
\sum_{n = 0}^{\infty} G_n x^{\Psi_n}, & 
Y \big( R^{-1}(x) \big) = \displaystyle
\sum_{n = 0}^{\infty} B_n x^{\Phi_n}, 
\\ \\
M_1 \big( R^{-1}(x) \big) = \displaystyle 
\sum_{n = 0}^{\infty} K_n x^{\Pi_n}, &
M_2^{\prime} \big( R^{-1}(x) \big) = \displaystyle 
\sum_{n = 0}^{\infty} L_n x^{\Theta_n}
\end{array}
\label{HahnFrame}
\end{equation}

whose leading powers determine the dynamic exponents $\Omega = (\eta, \mu, \nu, \rho)$ as

\begin{equation}
\begin{array}{cccc}
\mu = 2 - \Phi_0, & 
\nu = -\Pi_0, &
\rho = -\Theta_0, &
\eta  = -\Psi_0 (\mu - \nu - \rho).
\end{array}
\label{ExponentsFrame}
\end{equation}

To construct $J \in \Ew$ (around a non-trivial fixed-point) we first assign the network/weights $A,G$, then extract the weighted degrees $d_i$ of all nodes and the nearest neighbor degree $\knn$ from Eq.\ (\ref{kappa}). The resulting $J$ satisfies 

\begin{eqnarray}
\m Jii &\sim& -C \knn^{\eta} d_i^{\mu}
\label{JiiFrame}
\\[8pt]
\m Jij &\sim& d_i^{\nu} \m Aij \m Gij d_j^{\rho},
\label{JijFrame}
\end{eqnarray}

where the constant $C > 0$ is arbitrary.
\end{Frame}
\end{figure} 
%%%%%%%%%%%%%%%%%%%%%%%%%%%%%%%%%%%%%%%%%%%%%%%%%%%%%%%%%%%%%%%%%%%%%%%%%%%%%%%%%%%%%%%%
%%%%%%%%%%%%%%%%%%%%%%%%%%%%%%%%%%%%%%%%%%%%%%%%%%%%%%%%%%%%%%%%%%%%%%%%%%%%%%%%%%%%%%%%

In this derivation we considered the scaling of $J$ on the weighted degrees $d_i,d_j$, and on the nearest neighbor degree $\knn$. Valid under the general assumptions listed in Sec.\ \ref{SecFramework}, the discussion becomes especially relevant when $P(d)$ is fat-tailed, \textit{e.g.}, scale-free, where degrees, indeed, span orders of magnitude, and the scaling relationships reach their asymptotic limit. Specifically, as the hub-degrees and the nearest neighbor degree can potentially diverge with $N$, we can obtain our predicted asymptotic classes.

\textbf{The role of $\knn$}.\
While $d_i$ is a node specific attribute, that captures a specific dependency between the $i$th diagonal term and $i$'s weighted degree, the pre-factor $\knn^{\eta}$ in (\ref{JiiJij1}) represents a network aggregated parameter, indeed - a \textit{constant}, whose impact is often negligible in the asymptotic limit of large $d$. We include it in our analysis, however, because under extreme degree-heterogeneity, we may observe that $\knn$ diverges as $\knn \sim N^{\beta}$ (\ref{knnNBeta}), and therefore \textit{can} potentially impact the system's stability in the limit $N \rightarrow \infty$. For example, in a random scale-free network where $P(d) \sim d^{-\gamma}$, we can use $\knn = \av{d^2}/\av{d}$ in (\ref{k2overk}) to obtain

\begin{equation}
\knn \sim 
\left\{
\begin{array}{lcc}
N & & \gamma < 2
\\
N^{3 - \gamma} & & 2 \le \gamma < 3
\\
\log(N) & & \gamma \ge 3
\end{array}
\right.,
\label{kappavsN}
\end{equation}

which scales with $N$ as long as $\gamma < 3$. There are, however, broad conditions, that arise quite naturally in many real systems, in which the $\knn$ term in (\ref{JiiJij1}) can be neglected, helping us simplify the stability analysis:

\textbf{Finite $\knn$}.\ In case $\gamma \ge 3$, $\knn$ no longer scales with $N$, it behaves as a constant and has no impact in the asymptotic limit. Under these conditions it suffices to write Eq.\ (\ref{JiiJij1}) as $\m Jii \sim -Cd_i^{\mu}$, with $\knn$ effectively encapsulated within $C$.

\textbf{Bounded activities}.\ In some models the activities $x_i$ are bounded. For example, in spreading processes, from epidemics to cascading failures, the activities satisfy $0 \le x_i \le 1$. Under these conditions the leading power in the power-series expansion of (\ref{xdRinv}) is zero, and hence $x(d \rightarrow \infty) \sim 1$. The result is that the nearest neighbor activity $x_{\nn}$, associated with degree $\knn$ is itself bounded, and even if $\knn \rightarrow \infty$ as in Eq.\ (\ref{kappavsN}), we still have $x_{\nn} \sim 1$. Consequently $M_2(x_{\nn})$ in (\ref{M2chi}) also approaches a constant value, and therefore the leading power in the expansion (\ref{M2Laurent}) is $\Psi_0 = 0$. This provides, based on Eq.\ (\ref{kappaxi}), $\xi = 0$, which in turn leads to $\eta = 0$ in (\ref{JiiJij1}), again resulting in $\m Jii \sim -Cd_i^{\mu}$, independent of $\knn$.

\textbf{Saturating $M_2(x)$}.\ Another common feature in many relevant models is that $M_2(x_j \rightarrow \infty) \rightarrow 1$. This represents the saturating impact of node $j$ on its nearest neighbor $i$, as frequently observed in regulatory processes or in population dynamics. Once again, we have $M_2(x_{\nn}) \sim 1$ in the limit of large $x_{\nn}$, providing $\xi = 0$, and consequently $\eta = 0$ in (\ref{JiiJij1}).  

These rather frequent scenarios, observed, \textit{e.g}., in our Epidemic, Regulatory, Population and Power dynamics provide a simplifies $J$, in which $\eta = 0$, omitting $\knn$ from the stability analysis. In Biochemical and Inhibitory, on the other hand, we have $\eta \ne 0$, and hence the $\knn$ term cannot be neglected.

%\clearpage

\subsection{$J$ around a trivial fixed-point}
\label{TrivialSolution}

Our derivation up to this point relied on the function $R_i(x_i) = -M_1(x_i,\m \f1i)/M_0(x_i,\m \f0i)$, which becomes undefined in case $M_0(x_i,\m \f0i) = 0$. This represents a \textit{trivial} fixed-point, in which the activities satisfy

\begin{equation}
x_i = M_0^{-1}(0,\m \f0i).
\label{xM0Inverse}
\end{equation} 

Returning to Eq.\ (\ref{FixedPoint}), we write

\begin{equation}
M_0 (x_i,\m \f0i) + \g \sum_{j = 1}^N \m Aij \m Gij M_1(x_i,\m \f1i) M_2(x_j,\m \f2j) = 0,
\label{FixedPointi2}
\end{equation}

which, if $M_0 (x_i,\m \f0i) = 0$, can only be solved by setting either $M_1(x_i,\m \f1i) = 0$ for all $i$ or $M_2(x_j,\m \f2j) = 0$ for all $j$. In the first case we write

\begin{equation}
x_i = M_1^{-1}(0,\m \f1i),
\label{xM1inverse}
\end{equation}

and in the second case we have

\begin{equation}
x_j = M_2^{-1}(0,\m \f2j).
\label{xM2inverse}
\end{equation}

In principle such conditions may arise under a general $x_i$, including $x_i \ne 0$. However, having \textit{all} $x_i$ satisfy at least two of the conditions (\ref{xM0Inverse}), (\ref{xM1inverse}) and (\ref{xM2inverse}) is extremely unlikely under a \textit{natural} selection of $M_0(x), M_1(x)$ and $M_2(x)$, unless one specifically designs these functions to sustain such solutions. Indeed, one must sets all links $\m Aij$, weights $\m Gij$ and rate constants $\f,\g$, together with the functional form of $M_0(x), M_1(x)$ and $M_2(x)$ to have a non-zero $\mathbf{x}^*$ that simultaneously solves all $N$ equations of (\ref{FixedPointi2}). Such \textit{fine-tuning}, indeed a specific and highly non-random design, is excluded from our derivation, which is centered around complex, typically random, and most often heterogeneous systems. In simple terms, the probability for such solution to exist within our dynamic ensemble is practically zero.  

The natural exception to the above fine-tuned solution is the trivial solution $x_i = 0$ for all $i$, which, indeed, arises in many real-world systems, including ones examined in the present analysis. For example, in Epidemic dynamics, the healthy state $x_i = 0$ has $M_0(x_i,\m \f0i) = -f_i x_i = 0$, and $M_2(x_j) = x_j = 0$, hence satisfying (\ref{xM0Inverse}) and (\ref{xM2inverse}). In Population 1, the null-state has $M_0(x_i,\m \f0i) = b_ix_i(1 - x_1/c_i) = 0$, $M_1(x_i,\m \f1i) = x_i = 0$ and $M_2(x_j,\m \f2j) = F(x_j) = 0$, satisfying all three conditions simultaneously. Finally, in Inhibitory and Regulatory, the null-state has $M_0(x_i = 0,\m \f0i) = M_1(x_i = 0,\m \f1i) = 0$ and $M_0(x_i = 0,\m \f0i) = M_2(x_j = 0,\m \f2j) = 0$, respectively, once again satisfying two of the conditions (\ref{xM0Inverse}) - (\ref{xM2inverse}). This specific state - the null state $\mathbf{x}^* = (0,\dots,0)^{\top}$ - cannot be analyzed via the above derivation, and requires a dedicated treatment. 

To obtain $J$ around the null state we use (\ref{Dii2}) and (\ref{Qij2}) to write

\begin{eqnarray}
\m Wii &=& M_0^{\prime}(0) + \g M_1^{\prime}(0) d_i M_2(0)
\label{DiiTrivial}
\\[5pt]
\m Wij &=& \g M_1(0) \m Aij \m Gij M_2^{\prime}(0),
\label{WijTrivial}
\end{eqnarray}

omitting, for simplicity, the parameter terms $\m \f qi$. Several distinct cases arise (Table \ref{TableNull}):\

%%%%%%%%%%%%%%%%%%%%%%%%%%%%%%%%%%%%%%%%%%%%%%%%%%%%%%%%%%%%%%%%%%%%%%%%%%%%%%%%%%%%%%%%%
%%%%%%%%%%%%%%%%%%%%%%%%%%%%%%%%%%%%%%%%%%%%%%%%%%%%%%%%%%%%%%%%%%%%%%%%%%%%%%%%%%%%%%%%%
\begin{table}[h!]
\includegraphics[width=16cm]{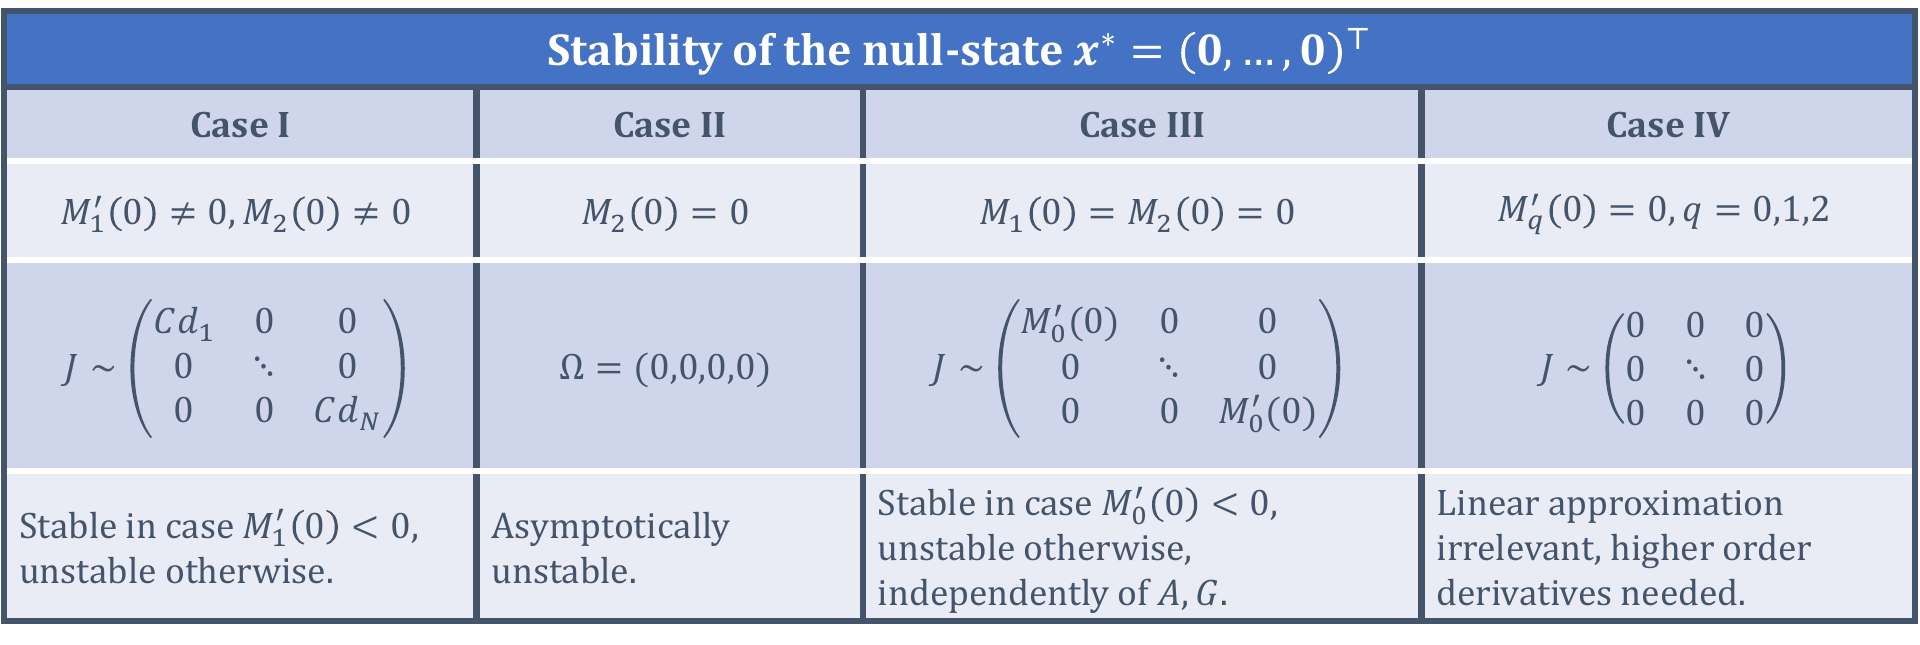}
\vspace{-8mm}
\caption{\footnotesize \color{blue} \textbf{Stability of the null-state $\x^* = (0,\dots,0)^\top$}.\
The null-state cannot be treated via our general formalism, and hence we analyze it separately. Our analysis distinguishes between four cases, depending on the values of $M_q(0)$ and $M_q^\prime(0)$.}
\label{TableNull}
\end{table}
%%%%%%%%%%%%%%%%%%%%%%%%%%%%%%%%%%%%%%%%%%%%%%%%%%%%%%%%%%%%%%%%%%%%%%%%%%%%%%%%%%%%%%%%%
%%%%%%%%%%%%%%%%%%%%%%%%%%%%%%%%%%%%%%%%%%%%%%%%%%%%%%%%%%%%%%%%%%%%%%%%%%%%%%%%%%%%%%%%%

%%%%%%%%%%%%%%%%%%%%%%%%%%%%%%%%%%%%%%%%%%%%%%%%%%%%%%%%%%%%%%%%%%%%%%%%%%%%%%%%%%%%% 
%%%%%%%%%%%%%%%%%%%%%%%%%%%%%%%%%%%%%%%%%%%%%%%%%%%%%%%%%%%%%%%%%%%%%%%%%%%%%%%%%%%%% 

\textbf{Case I}.\ In case $M_1^{\prime}(0)$ and $M_2(0)$ are both non zero, we have the diagonal terms scaling as $\m Wii \sim d_i$, corresponding to $\mu = 1$. Here, since $M_2(0) \ne 0$, the null-solution of (\ref{FixedPointi2}) inevitably requires that $M_1(0) = 0$, \textit{i.e}.\ condition (\ref{xM1inverse}). Consequently, the off-diagonal terms in (\ref{WijTrivial}) all vanish, indicating that the interactions, in this case, have no linear contribution, and are only expressed via higher order nonlinear terms. In $\Ew$ this is captured by taking the limit $\nu,\rho \rightarrow -\infty$, deep within the asymptotically stable regime in case $\m Jii$ is negative ($M_1^\prime(0) < 0$), or the unstable regime if it is positive ($M_1^\prime(0) > 0$). As an example, we consider the dynamics $\dif x_i/\dif t = - f_i x_i - \g \sum_{j = 1}^N \m Aij \m Gij x_i/(1 + x_j)$, in which the interaction is of deactivating nature. Using (\ref{DiiTrivial}) we write $\m Jii = -1 - \g d_i$, which, indeed, under large $d_i$, scales as $\m Jii \sim -d_i^{\mu}$ with $\mu = 1$. The off-diagonal terms, in this dynamics vanish as per Eq.\ (\ref{WijTrivial}).    

\textbf{Case II}.\ If, however $M_2(0) = 0$, \textit{i.e}.\ condition (\ref{xM2inverse}),
 we have both $\m Wii$ and $\m Wij$ independent of $d_i,d_j$, predicting $J \in \Ew$ with $\Omega = (0,0,0,0)$. This captures an asymptotically unstable fixed point. We observe this, for example, in the healthy state of Epidemic dynamics. There we have $M_0^{\prime}(0) = f_i$, $M_2(0) = 0$ and $M_1(0)M_2^{\prime}(0) = 1$. Together this leads to $\m Wii, \m Wij \sim \rm const$, \textit{i.e}.\ lacking any scaling with $d_i$ and $d_j$. Indeed, we show in the Sec.\ \ref{ModelsSIS} that the healthy state of the Epidemic model is asymptotically unstable, recovering a well-established result on the spread of epidemics on scale-free networks \cite{PastorSatorras2001a}.  

\textbf{Case III}.\ A third scenario is when both conditions (\ref{xM1inverse}) and (\ref{xM2inverse}) are satisfied, \textit{i.e}.\ $M_1(0) = M_2(0) = 0$. The off-diagonal terms in (\ref{WijTrivial}) vanish in this case, indicating that the interactions are super-linear, having no linear component. The diagonal terms become $\m Wii = M_0^{\prime}(0)$, independent of the network structure. Therefore, in such dynamics stability is fully determined by the sign of $\m Wii$, unstable in case $M_0^{\prime}(0) \ge 0$ and stable otherwise. We encounter such conditions in Population 1, where $M_1(x) = x$ and $M_2(x) = x/(1 + x)$, both zero when $x = 0$. The self-dynamics in this case has $M_0(x) = b_ix(1 - x/c_i)$, whose derivative around $x = 0$ provides $\m Wii = b_i > 0$. This dynamics is, therefore, always unstable around the trivial fixed-point. 

Note that Cases II and III are of different nature. While Case II is a specific member of $\Ew$, with all exponents being zero, Case III's instability is unrelated to $\Ew$. To understand this consider Epidemic's trivial state, which is in Case II, vs.\ that of Population 1, which is in Case III. The former can potentially be stable, if, for instance the recovery rate $f_i$ is large enough. Its instability only emerges asymptotically in the limit of large and heterogeneous networks, \textit{i.e}.\ our asymptotically unstable class. Therefore it is an integral system within out ensemble $\Ew$. Indeed, this form of asymptotic instability emerges from the interplay between topology ($P(d),N$) and dynamics ($\Omega$), representing  a direct outcome of our theoretical framework. Case III dynamics, in contrast, have an intrinsically unstable null state, even under low dimension (small $N$) or non-heterogeneous degrees ($P(d)$ homogeneous). Their null state instability, is, therefore, not driven by the topology/dynamics interplay, ingrained in our $J$-ensemble, but rather it is independent of topology. Indeed, as we discuss in Sec.\ \ref{SecPopulation1}, in Population 1 the null state is always unstable, even in a one-dimensional system.     

\textbf{Case IV}.\ The final case is where $M_0^{\prime}(0) = M_1^\prime(0) = M_2^{\prime}(0) = 0$, which occurs when these functions are super-linear around $x = 0$. Under these conditions the linear approximation becomes irrelevant and higher order terms must be included to capture the fixed-point dynamics. As an example, we consider our Regulatory dynamics, having $M_0(x,\f_i) = -f_i x^a, M_1(x) = 1$ and $M_2(x) = x^h/(1 + x^h)$. For $a,h > 1$ the first derivatives vanish around $x = 0$, and $J$ is void. Consequently, under these conditions the null state Jacobian vanishes, and hence cannot be used to assess the system's stability. Such cases, where $J$ is irrelevant require specific treatment, independent of our formalism, which is specifically focused on $J$. Fortunately, this treatment under Case IV, is quite straightforward, as we demonstrate in our analysis of the Regulatory dynamics in Sec.\ \ref{SecRegulatory}.   

To summarize, our analytical framework of (\ref{FunctionsFrame}) - (\ref{JijFrame}) is designed to treat the non-trivial fixed-points of (\ref{Dynamics}). If, however, the system exhibits also a null $\x^* = (0,\dots,0)^{\top}$ state, we must treat this state specifically, following the case by case analysis presented above. Fortunately, these null state Jacobians are straightforward to analyze, and can be done alongside our general analytical derivation. 

{\color{blue} \rule{12cm}{1mm}}
\vspace{2mm}  		
\section{Principle eigenvalue of $J \in \Ew$}
\label{SecPrincipleEigenvalue}

While the principal eigenvalue $\lambda$ of $J \in \Ew$ is difficult to obtain analytically, we find that simplifying $A$ into a \textit{star-network} can provide a rather reliable prediction, especially since we are only focused on whether $\lambda$ is positive/negative, not on its specific value. We first distinguish between two families of dynamics:\ the first has $\s = 1$, describing cooperative interactions, in which the off-diagonal terms $\m Jij > 0$. This is observed, for example, in Regulatory or in Epidemic, where $j$ positively contributes to its neighbor $i$'s activity. The second option, $\s = 0$, describes adversarial interactions, where $j$' activity has a negative impact on $x_i$. This can be indirect, such as in Inhibitory, where $x_j$ decreases $i$'s \textit{growth rate}, or direct, such as in Biochemical, where $j$ directly depletes the $i$ population via chemical binding.     

\textbf{\color{blue} The star-construction}.\
The structure of $J$ in (\ref{JiiFrame}) - (\ref{JijFrame}) depends strongly on the network degrees through $d_i,d_j$ and $\knn$. Recalling the mean-field approximation of Sec.\ \ref{SecTopology}, we can capture the stability of the system by examining the dynamics of a typical neighborhood. We therefore consider a single node, with weighted degree $\knn$, \textit{i.e}.\ a typical neighbor. Since weights $\m Gij$ are randomly distributed, uncorrelated with degree (Sec.\ \ref{SecTopology}), we can extract our neighbor's unweighted degree $k$ from its weighted $\knn$ via $\knn \approx \av{G} k$, which using Eq.\ (7) of the main text provides 

\begin{equation}
k \propto \knn \sim N^\beta
\label{Beta}
\end{equation}

a potential divergence with system size in case $P(k)$ is fat-tailed.

This construction captures the environment of a typical hub in, \textit{e.g}., a scale-free network. Indeed, such hubs in a scale-free environment can be viewed as a collection of weakly coupled \textit{stars}, that are only sparsely linked to each other \cite{Brenner2017}. Under these conditions we have the $(k + 1) \times (k + 1)$ network

\begin{equation}
\begin{split}
A 
&= \begin{bmatrix}
0 &1 &1&\ldots&1 \\
1 &0 &0&\ldots&0 \\
\vdots& &\ddots &&\vdots \\
1&0 &0& \dots&0
\end{bmatrix}
\end{split},
\label{AijStar}
\end{equation}

capturing a single, highly connected node, surrounded by $k$ small nodes.

\subsection{Jacobians with positive weights $\s = 1$}

We now use (\ref{JiiFrame}) and (\ref{JijFrame}), to construct the Jacobian of the star-network (\ref{AijStar}), which under cooperative interactions takes the form 

\newcommand{\Sknn}{\tilde{d}_{\rm nn}}  
  
\begin{equation}
\begin{split}
J
&= 
- C \Sknn^{\eta}
\begin{bmatrix}
k^{\mu} & 0 & \ldots & 0 \\
0 & 1 & \ldots &0 \\
\vdots & & \ddots & \vdots \\
0 & 0 & \dots & 1
\end{bmatrix}
+
\begin{bmatrix}
0 & k^{\nu} & \ldots & k^{\nu} \\
 k^{\rho} & 0 &\ldots & 0 \\
\vdots & & \ddots & \vdots \\
 k^{\rho} & 0 & \dots & 0
\end{bmatrix},
\end{split}
\label{JijStar}
\end{equation}

where $C > 0$ and the off-diagonal terms are all positive. In (\ref{JijStar}) we used $\Sknn$ to express the nearest neighbor degree in our star construction, which is potentially distinct from $\knn$ of the originally approximated scale-free network. Lacking an \textit{a priori} estimate for this parameter we express is as 

\begin{equation}
\Sknn \sim N^{\alpha},
\label{Alpha}
\end{equation}

leaving us a degree of freedom to later tune $\alpha$ such that the prediction from our star construction best captures the observed results from the actual complete networks (note:\ $\alpha$ in (\ref{Alpha}) is unrelated to that of (\ref{fXodotdalpha}) in Sec.\ \ref{SecTopology}). Hence, $\beta$, characterizing the star-hub ($k$), is extracted from $A$ via (\ref{dnn}) and $\alpha$ is a tunable parameter, which we select for the star-model to best fit the complete network results. 

\begin{Frame}
We emphasize that the star approximation in (\ref{AijStar}) by no means captures the complete behavior of an actual network, as indeed it represents but a crude representation of an isolated single node environment. However, our goal here is to examine stability vs.\ instability - a feature that only depends on the \textit{sign} of the principal eigenvalue, not on its specific value, and is, therefore, insensitive to the detailed structure of $A$. As we show in Fig.\ 4 of the main text, the star approximation, while highly stylized, is, indeed, sufficient to capture this $J$ characteristic. 
\end{Frame}

To obtain the principal eigenvalue we solve the linear equation

\begin{equation}
J \mathbf{v} = \lambda \mathbf{v}.
\label{Jxlambdax}
\end{equation}

Using the symmetry of (\ref{JijStar}), we seek a solution of the form $\mathbf{v} = (a, b, b, \dots, b)^{\top}$, allowing us to reduce (\ref{Jxlambdax}) into

\begin{eqnarray}
- C \Sknn^{\eta} k^{\mu} a + k k^{\nu} b &=& \lambda a
\label{StarEivEq1}
\\[7pt]
k^{\rho} a - C \Sknn^{\eta} b &=& \lambda b.
\label{StarEivEq2}
\end{eqnarray}  

Note that in $\mathbf{v}$ the specific values of $a,b$ have no significance, only the ratio $a/b$, as we are only interested in the \textit{direction} of the eigenvector, not its magnitude. We therefore arbitrarily set $a = 1$, allowing us to solve (\ref{StarEivEq1}) - (\ref{StarEivEq2}) and obtain

\begin{equation}
\lambda = \dfrac{1}{2}
\left(
-C \Sknn^{\eta} (k^{\mu} + 1) + 
\sqrt{C^2 \Sknn^{2 \eta} (k^{\mu} + 1)^2 - 
4C^2 \Sknn^{2 \eta} k^{\mu} + 4k^{1 + \nu + \rho}}
\right),
\label{PEV}
\end{equation}

where, of the two solutions, we selected only the one in which the square-root is added (rather than subtracted), as we seek the \textit{largest} eigenvalue. Focusing on the limit 

\begin{equation}
\lim_{N \rightarrow \infty} \big( \lambda \big),
\label{LambdaNlarge}
\end{equation}

we use (\ref{Beta}) and (\ref{Alpha}) to rewrite (\ref{PEV}) as

\begin{eqnarray}
\lambda &\sim& \dfrac{1}{2}
\left(
-C N^{\alpha \eta} \big( N^{\beta \mu} + 1  \big) 
\right.
\nonumber \\
&+&
\left.
\sqrt{C^2 N^{2\alpha \eta} (N^{\beta \mu} + 1 )^2 +
4 \left[ 
-C^2 N^{2\alpha \eta + \beta \mu} + N^{\beta (1 + \nu + \rho)} 
\right]}
\right),
\label{PEV2}
\end{eqnarray}

in which we replace $\Sknn$ and $k$ by $N^{\alpha}$ and $N^{\beta}$, respectively. In (\ref{PEV2}) we ignore the pre-factors of the $N$-scaling, focusing only on the powers ($\alpha, \beta$), hence substituting the equality sign $=$ with the asymptotic scaling operator $\sim$. 

\vspace{3mm}
\textbf{\color{blue} The case where $\mu > 0$}.\ First we analyze $\lambda$ under $\mu > 0$. Here, we write $N^{\beta \mu} \gg 1$, simplifying (\ref{PEV2}) in the limit $N \rightarrow \infty$ into

\begin{equation}
\lambda \sim \dfrac{1}{2}
\left(
-C N^{\alpha \eta + \beta \mu} + \sqrt{C^2 N^{2(\alpha \eta + \beta \mu)} +
4 \left[ 
-C^2 N^{2\alpha \eta + \beta \mu} +
N^{\beta (1 + \nu + \rho)} 
\right]}
\right).
\label{PEV1mupositive}
\end{equation}

Extracting the common terms out of the product we rewrite (\ref{PEV1mupositive}) as

\begin{equation}
\lambda \sim \dfrac{1}{2}
C N^{\alpha \eta + \beta \mu} 
\left(
-1 + \sqrt{1 +
4 \left( 
- N^{-\beta \mu} +
\dfrac{1}{C^2} N^{\sigma} 
\right)}
\right),
\label{PEV2mupositive}
\end{equation}

where 

\begin{equation}
\sigma = \beta \left( 1 + \nu + \rho - 2\mu - 2 \dfrac{\alpha}{\beta} \eta \right).
\label{Sigma}
\end{equation}

Note that in (\ref{PEV2mupositive}) the term $N^{-\beta \mu} \le 1$, as $\mu > 0$. Therefore, in case $\sigma \ge 0$, the $N^{\sigma}$ term dominates the r.h.s.\ of the equation, providing, under $N \rightarrow \infty$,

\begin{equation}
\lambda \sim \dfrac{C}{\sqrt{C^2}} N^{\frac{1}{2}\sigma + \alpha \eta + \beta \mu}.
\label{SigmaPositive}
\end{equation}

Using the fact that $C > 0$ it becomes guaranteed that $\lambda$ in (\ref{SigmaPositive}) is positive, \textit{i.e}.\ the system is \textit{unstable}. 

Next we consider the case $\sigma < 0$. Under these conditions $N^{\sigma} \ll 1$, allowing us to expand the square-root in (\ref{PEV2mupositive}) to first order, providing

\begin{equation}
\lambda \sim \dfrac{1}{2}
C N^{\alpha \eta + \beta \mu} 
\left(
-1 + 1 + 2 
\left(
-N^{- \beta \mu} + \dfrac{1}{C^2} N^{\sigma}
\right)
\right) = 
-C N^{\alpha \eta} + \dfrac{1}{C} N^{\sigma + \alpha \eta + \beta \mu}.
\label{PEV3mupositive}
\end{equation}

We can rewrite this in the form of Eq.\ (8) of the main text, obtaining

\begin{equation}
\lambda \sim N^Q \left( 1 - \dfrac{C}{N^{S}} \right),
\label{Eq11MainText1}
\end{equation}

where

\begin{eqnarray}
Q &=& \sigma + \alpha \eta + \beta \mu
\label{QMainText1}
\\[5pt]
S &=& \sigma + \beta \mu.
\label{SMainText1}
\end{eqnarray}

As $N^Q$ is guaranteed to be positive, the sign of $\lambda$ depends on $S$:\ in case $S > 0$ the negative term in (\ref{Eq11MainText1}) satisfies $CN^{-S} \ll 1$, and hence we have $\lambda \sim N^Q > 0$, an unstable dynamics. If however $S < 0$, we have $-CN^{-S} \rightarrow -\infty$, predicting $\lambda < 0$, regardless of $C$, an asymptotically stable system. Consequently the system is stable as long as $S < 0$, which, using (\ref{SMainText1}), and taking $\sigma$ from (\ref{Sigma}), predicts the stability condition

\begin{equation}
\beta \left( 1 + \nu + \rho - \mu -2\dfrac{\alpha}{\beta} \eta \right) < 0.
\label{StabilityCondition}
\end{equation}

This condition reduces stability into a small set of \textit{relevant} parameters:\ $\beta$, characterizing the network topology $A$, and $\Omega = (\eta, \mu, \nu, \rho)$, associated with the dynamics through powers in the expansion of $M_q(x)$ in (\ref{Hahn}). The non-universal parameter $C = C(\f,\g)$ becomes irrelevant in the limit of sufficiently large $N$. Finally, $\alpha$ represents a degree of freedom to help tune the star approximation to best fit our ensemble of actual networks, as we do below. Note that condition (\ref{StabilityCondition}) can also be expressed as $\sigma + \beta \mu < 0$. This implies that if $\sigma > \beta \mu$ the system is unstable. This instability condition already contains the previously obtained condition of $\sigma > 0$, that led to Eq.\ (\ref{SigmaPositive}). Therefore, Eq.\ (\ref{StabilityCondition}) is sufficient to characterize the system's stability, covering both the $\sigma$ positive and the $\sigma$ negative cases. 

Finally, the case $S = 0$ in (\ref{Eq11MainText1}) represents sensitive stability, in which $\lambda$'s value is not asymptotically defined, and rather it depends on the coefficient $C$. In this class, stability in no longer a characteristic of the dynamic \textit{model}, but rather of its specific rate constants $\f$ and $\g$, as encapsulated within $C$. A trivial example is when $\beta = 0$, \textit{i.e}.\ a non fat-tailed $P(d)$, for example - Erd\H{o}s-R\'{e}nyi. Indeed, as we discuss in the main text, in such networks, stability can be tuned by the model parameters, lacking a defined asymptotic behavior. 

\vspace{3mm}
\textbf{\color{blue} The case where $\mu \le 0$}.\ 
Here, we have $N^{\beta \mu} \le 1$, and hence Eq.\ (\ref{PEV2}) can be approximated by  

\begin{equation}
\lambda \sim \dfrac{1}{2}
\left(
-C N^{\alpha \eta} + 
\sqrt{C^2 N^{2\alpha \eta} + 
4 \big[ -C^2 N^{2\alpha \eta + \beta \mu} + N^{\beta (1 + \nu + \rho)} \big]}
\right),
\label{PEV1munegative}
\end{equation}

leading to

\begin{equation}
\lambda \sim \dfrac{1}{2}
C N^{\alpha \eta}
\left(
-1 + \sqrt{1 + 4 
\left(
-N^{\beta \mu} +
\dfrac{1}{C^2} 
N^{\omega}
\right)
}
\right),
\label{PEV2munegative}
\end{equation}

where

\begin{equation}
\omega = \beta \left( 1 + \nu + \rho - 2\dfrac{\alpha}{\beta} \eta \right).
\label{omega}
\end{equation}

Equation (\ref{PEV2munegative}) features a summation of $N^{\beta \mu} \le 1$ with $N^\omega$, whose value depends on $\omega$. Therefore, as before, if $\omega > 0$, $\lambda$ becomes dominated by the $N^{\omega}$ term, following

\begin{equation}
\lambda \sim \dfrac{C}{\sqrt{C^2}}N^{\frac{1}{2}\omega + \alpha \eta}, 
\label{PEV3munegative}
\end{equation}

which is always positive, \textit{i.e.\ unstable}. If, however, $\omega < 0$, we use a linear approximation to write

\begin{equation}
\lambda \sim \dfrac{1}{2}
C N^{\alpha \eta} 
\left(
- 1 + 1 + 
2\left(
-N^{\beta \mu} + \dfrac{1}{C^2} N^{\omega}
\right)
\right) = 
-C N^{\alpha \eta + \beta \mu} +
\dfrac{1}{C} N^{\omega + \alpha \eta},
\label{PEV4munegative}
\end{equation} 

as before - a competition between a positive vs.\ a negative term. Collecting the powers we, once again, rewrite (\ref{PEV4munegative}) in the form 

\begin{equation}
\lambda \sim N^Q \left( 1 - \dfrac{C}{N^{S}} \right),
\label{Eq11MainText2}
\end{equation}

where this time

\begin{eqnarray}
Q &=& \omega + \alpha \eta 
\label{QMainText2}
\\[5pt]
S &=& \omega - \beta \mu.
\label{SMainText2}
\end{eqnarray} 

Stability is ensured if, for $N \rightarrow \infty$, the negative term dominates, namely if $S < 0$. Using (\ref{omega}) to express $\omega$ this provides

\begin{equation}
\beta \left( 1 + \nu + \rho - \mu - 2\dfrac{\alpha}{\beta} \eta \right) < 0,
\label{StabilityCondition2}
\end{equation}

recovering precisely the condition in (\ref{StabilityCondition}).

\begin{figure}
%\begin{center}
\includegraphics[width=16cm]{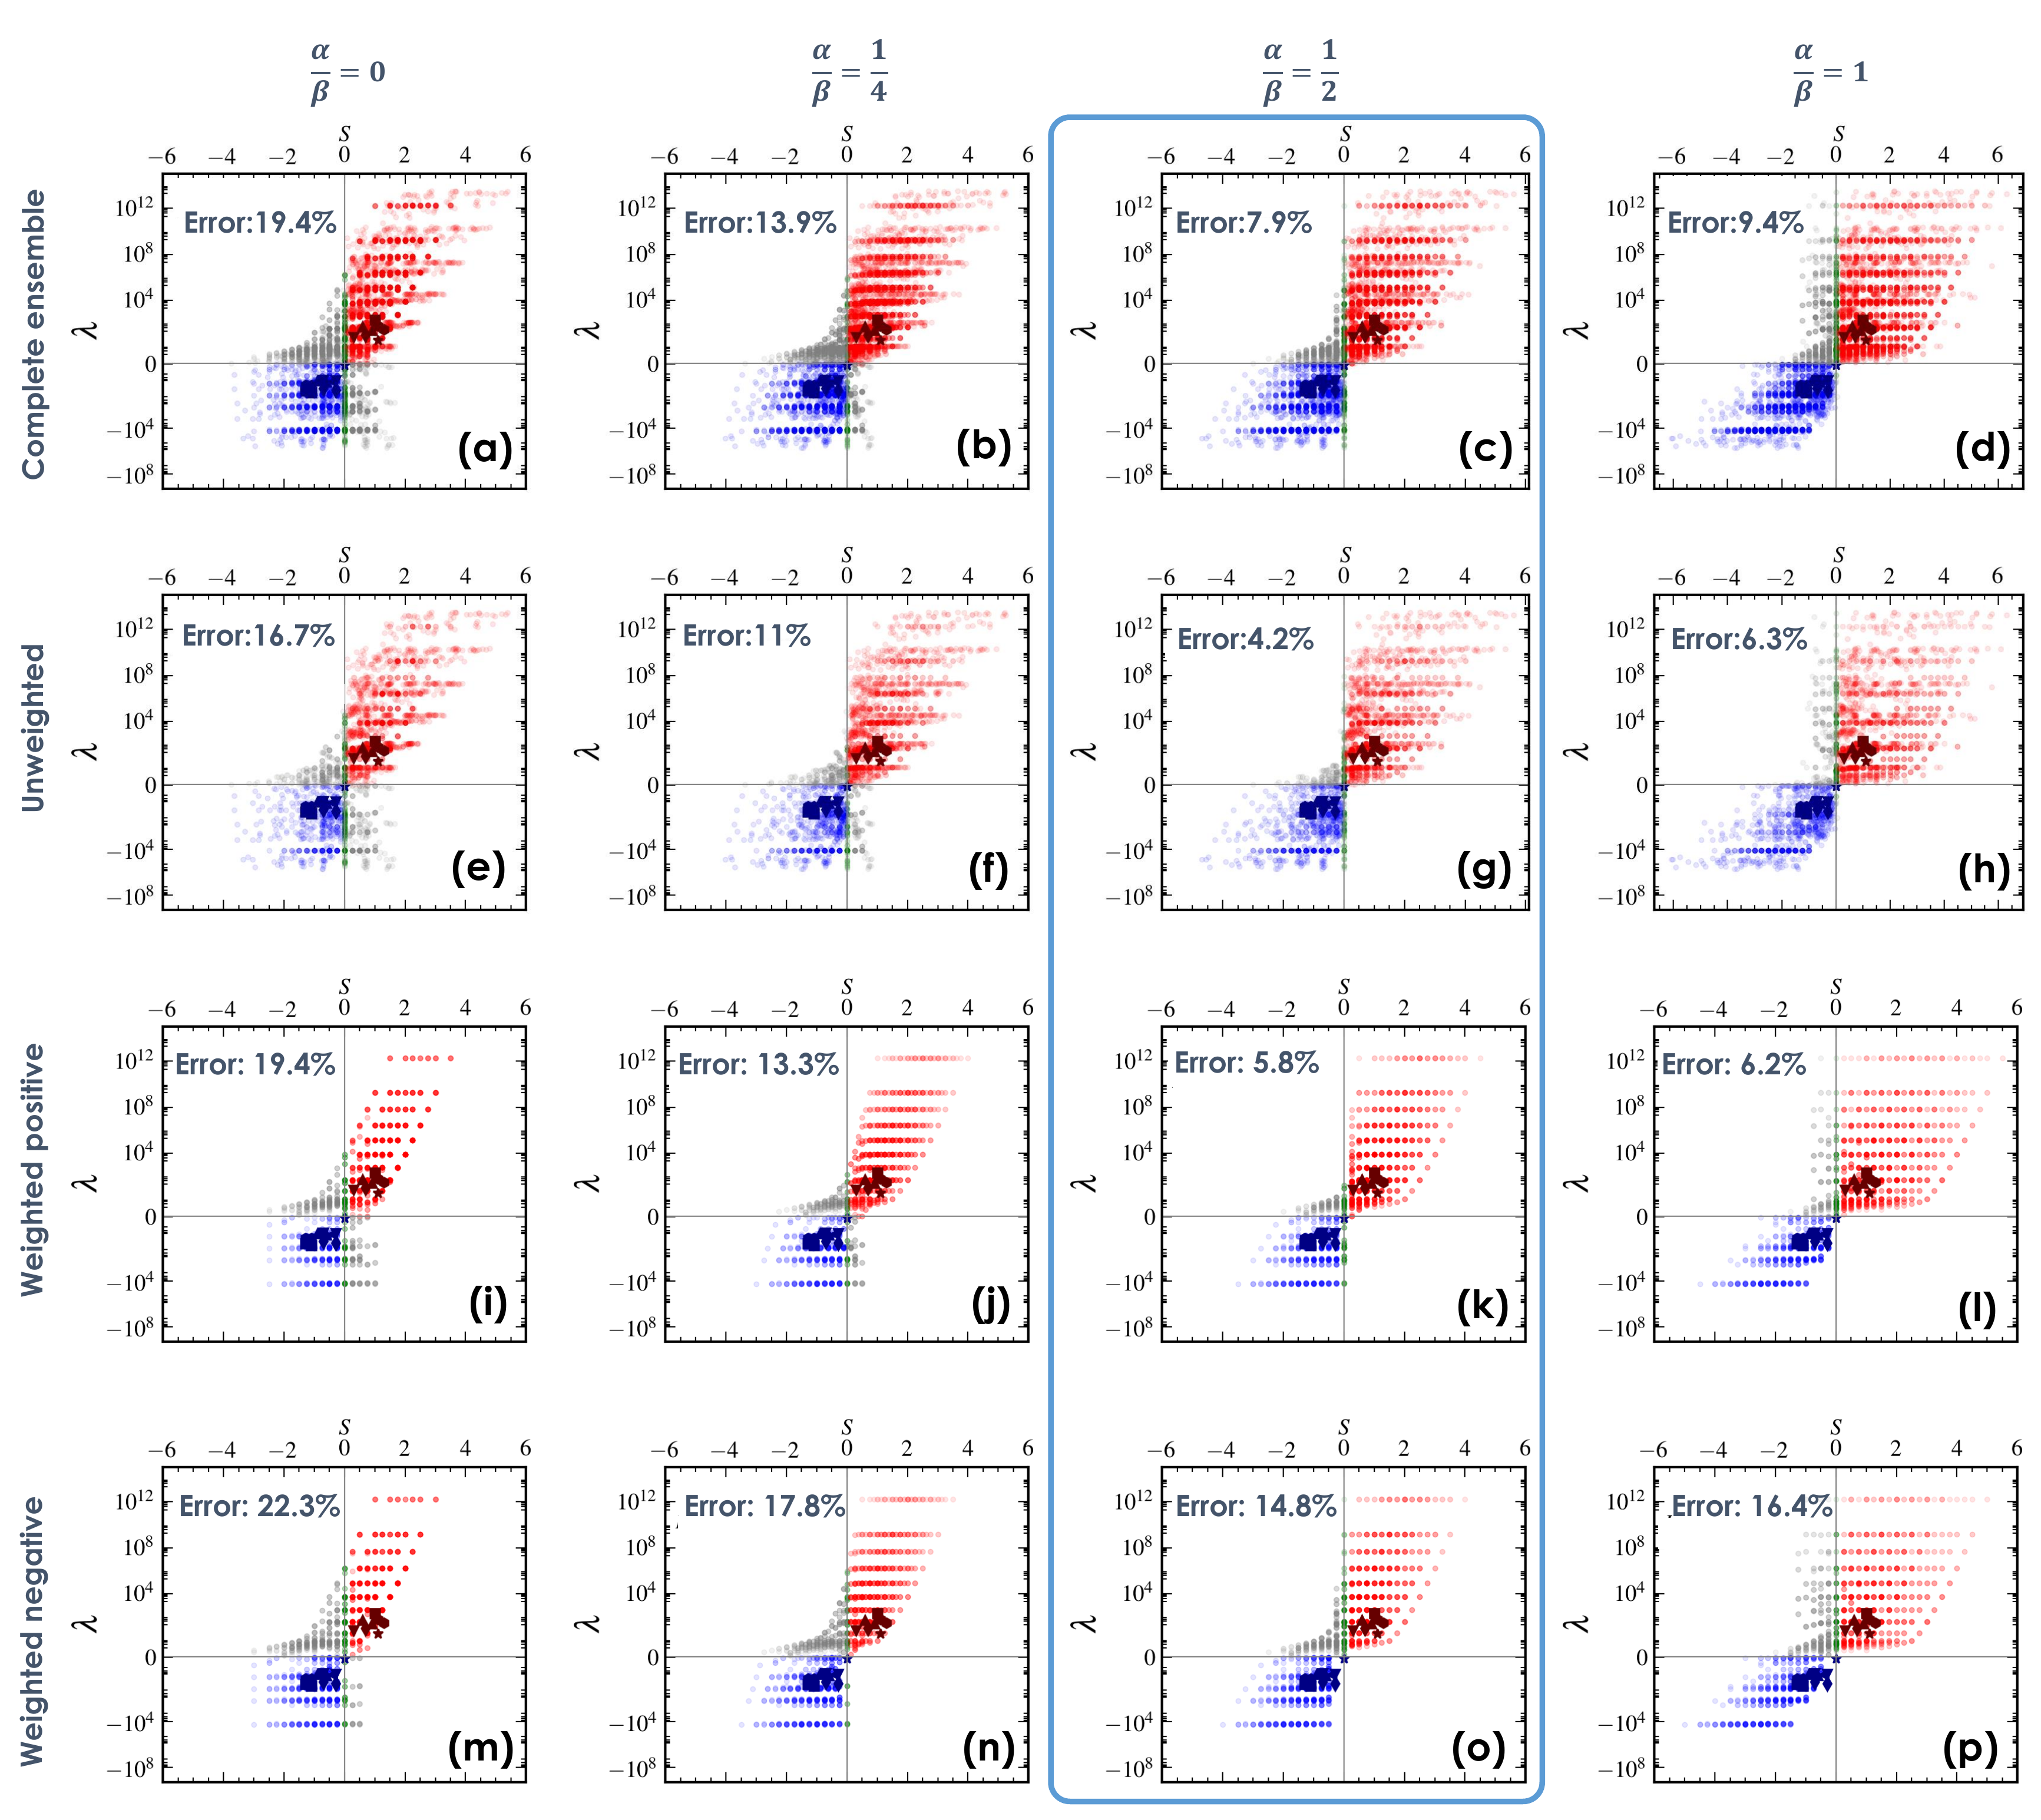}
\caption{\footnotesize \color{blue} \textbf{Tuning the parameter $\alpha$}.\ 
In Eqs.\ (\ref{StabilityCondition}) and (\ref{StabilityCondition2}) we have the degree of freedom to set $\alpha/\beta$ for the star approximation to best predict the stability of actual networks. We used our ensemble of $7,387$ $J$ matrices (Fig.\ 4a of main text) to predict stability using different values of $\alpha/\beta$. Quantifying the Error by the fraction of mis-classified $J$ matrices (grey dots), we find that setting $\alpha/\beta = 1/2$ (blue frame) provides the optimal fit:\ securing a $\sim 96\%$ correct classification (Error$= 4.2\%$) for unweighted networks, $\sim 94\%$ (Error$= 5.8\%$) for weighted networks and $\sim 85\%$ (Error$= 14.8\%$) for weighted networks with negative $\m Jij$. Here the empirical networks (Social 1,2; PPI 1,2; Power 1,2; Microbial 1/2) are highlighted in bold red/blue symbols}  
%\end{center}
\label{FigureTuningAlpha}
\end{figure}

\textbf{\color{blue} Tuning $\alpha$}.\
The parameter $\alpha$ represents a degree of freedom, rooted in the fact that the star approximation is a simplification, which can be optimized if we select this parameter such that the star best captures the complete network environment. We find that setting 

\begin{equation}
\alpha = \dfrac{\beta}{2}
\label{SettingAlpha}
\end{equation}

provides the optimal approximation, accurately predicting stability $\sim 96\%$ of the time for our $2,881$ unweighted networks, $\sim 94\%$ for our $2,290$ networks with distributed weights, and $\sim 85\%$ in our $2,216$ networks with negative links weights (Fig.\ \ref{FigureTuningAlpha}). This completes the stability analysis, providing the stability classifier

\begin{Frame}
\begin{equation}
S = \beta \left( 1 + \nu + \rho - \mu - \eta \right),
\label{S}
\end{equation}
\end{Frame}

as appears in Eq.\ (9) of the main text under $\s = 1$.

\subsection{Jacobians with negative weights $\s = 0$}
\label{SecNegativeS}

Adversarial interactions, in which $J$'s off-diagonal terms are negative confront us with more complex behaviors. Here, for example, $i$'s direct neighbor $j$ has a negative impact on $x_i$, but its second neighbor $m$ has an indirect positive effect, as it reduces $x_j$, and by that positively contributes to $x_i$. Our star approximation of (\ref{AijStar}), including only nearest neighbors, overlooks these indirect effects - and hence yields an identical outcome whether the interactions are cooperative, $\s = 1$, or adversarial, $\s = 0$. Therefore, to evaluate $S$ under negative $\m Jij$ we consider a fully connected network of 

\begin{equation}
k \sim N^{\beta}
\label{kNbeta}
\end{equation}

nodes, \textit{\`{a} la} May's original formulation \cite{May1972}. This, once again, we emphasize, is but a crude approximation, whose relevance we support via our extensive numerical testing (Fig.\ \ref{FigureTuningAlpha}). With \textit{all} nodes now having degree $k$, the resulting Jacobian takes the form

\begin{equation}
\begin{split}
J
&= 
- C k^{\eta}
\begin{bmatrix}
k^{\mu} & 0 & \ldots & 0 \\
0 & k^{\mu} & \ldots &0 \\
\vdots & & \ddots & \vdots \\
0 & 0 & \dots & k^{\mu}
\end{bmatrix}
-
\begin{bmatrix}
0 & k^{\nu + \rho} & \ldots & k^{\nu + \rho} \\
k^{\nu + \rho} & 0 & \ldots & k^{\nu + \rho} \\
\vdots & & \ddots & \vdots \\
k^{\nu + \rho} & k^{\nu + \rho} & \dots & 0
\end{bmatrix},
\end{split}
\label{JijFull}
\end{equation}
 
in which both the diagonal and the off-diagonal terms are preceded by a minus sign.

For a matrix of the form (\ref{JijFull}) the principal eigenvector is $\mathbf{v} = (1,-1,0,\dots,0)^{\top}$, whose associated eigenvalue is

\begin{equation}
\lambda = -C k^{\eta + \mu} + k^{\nu + \rho}. 
\label{lambdaNeg}
\end{equation}   

Using (\ref{kNbeta}) we rewrite (\ref{lambdaNeg}) in the form

\begin{equation}
\lambda = N^{Q} \left( 1 - \dfrac{C}{N^{S}} \right),
\label{lambdaNeg2}
\end{equation}   

where now

\begin{eqnarray}
Q &=& \beta (\nu + \rho)
\label{Qminus}
\\[5pt]
S &=& \beta (\nu + \rho - \mu - \eta).
\label{Sminus}
\end{eqnarray}

Hence under adversarial interactions the stability classifier is different from (\ref{S}), providing the stability condition

\begin{Frame}
\begin{equation}
S = \beta \left(\nu + \rho - \mu - \eta \right) < 0,
\label{Sneg}
\end{equation}
\end{Frame}

namely Eq.\ (9) of the main text, only this time, with $\s = 0$.

\textbf{\color{blue} The role of topology vs.\ dynamics}.\
The stability conditions (\ref{S}) or (\ref{Sneg}) are driven by five distinct exponents. The first four exponents $\Omega = (\eta, \mu, \nu, \rho)$ are determined by the dynamic model - Social, Regulatory, Population etc.\ - intrinsic to the system's inherent interaction mechanisms. These exponents are independent of the topology $A$ or of microscopic model parameters, encapsulated within $C$, and are therefore \textit{hardwired} into the system's dynamic behavior. For example, our formalism predicts that the SIS model (Epidemic) has $\Omega = (0,1,-1,0)$ (Sec.\ \ref{ModelsSIS}). This prediction is characteristic of the SIS model, namely it is an intrinsic feature of the SIS interaction mechanisms of infection and recovery. It is, therefore, insensitive to the specific rates of the model - predicting that $\Omega$ remains unchanged if, \textit{e.g.}, a disease has a high or low infection rate, or if it is transmitted via physical contact or aerosols. These will impact the constant $C$ in (\ref{JiiFrame}), but will have no impact on the universal scaling. Similarly, $\Omega$ is unaffected by $A$. Therefore, regardless of whether the disease spreads along the standard social network (Flu) or via sexual transmission (AIDS), as long as the \textit{mechanism} is SIS (or any other mechanism for that matter) $\Omega$ remains the same. The remaining exponent in our classifier, $\beta$, on the other hand, is independent of the dynamics, and determined solely by $A,G$, specifically by the weighted degree distribution $P(d)$, which characterizes the divergence of $\knn$ in the limit of large $N$. Hence, together, $S$ captures the emergence of stability/instability as driven by the interplay of topology ($\beta$), microscopic parameters ($C$) and dynamics ($\Omega$).

%%%%%%%%%%%%%%%%%%%%%%%%%%%%%%%%%%%%%%%%%%%%%%%%%%%%%%%%%%%%%%%%%%%%%%%%%%%%%%%%%%%%% 
%%%%%%%%%%%%%%%%%%%%%%%%%%%%%%%%%%%%%%%%%%%%%%%%%%%%%%%%%%%%%%%%%%%%%%%%%%%%%%%%%%%%% 
{\color{blue} \rule{12cm}{1mm}}
\vspace{2mm}  		
\section{Analyzing the dynamic models}	
\label{Models}
		
To demonstrate our formalism we examined several commonly used dynamic models, as listed in Fig.\ 2 of the main text. Below we extract the exponents $\Omega$ and the stability classifier $S$ for each of these models. The first five models are treated in this section, while the last two, Power and Population 2, which extend our application beyond the analytical framework of Sec.\ \ref{SecFramework}, are analyzes separately in Sec.\ \ref{SecExtendedDynamics}.

\subsection{Epidemic dynamics}
\label{ModelsSIS}

As our first demonstration we model epidemic spreading via the Susceptible-Infected-Susceptible (SIS) model \cite{PastorSatorras2015}, in which $x_i(t)$ captures the probability of infection of node $i$. Denoting the susceptible state by $\S$ and the infected state by $\I$, the model includes the following transitions  
	
\begin{eqnarray}
\I &\xrightarrow{f_i}& \S
\label{SIS1}
\\[7pt]
\I + \S &\xrightarrow{\m Gij}& 2\I,
\label{SIS2}
\end{eqnarray}

capturing the processes of recovery at a rate $f_i$, and infection at the pairwise interaction rate $\m Gij$. This gives rise to the dynamic equation \cite{Dodds2005}
	
\begin{equation}
\dod {x_i}{t} = -f_i x_i(t) + \g \sum_{j = 1}^N  \m Aij \m Gij \big( 1 - x_i(t) \big) x_j(t),
\label{SISDynamics}
\end{equation}
	
\noindent
in which $M_0(x_i, \m \f0i) = -f_i x_i$,, characterized by the single parameter $\m \f0i = \{f_i\}$, $M_1(x_i) = 1 - x_i$ and $M_2(x_j) = x_j$, both having no free parameters. The link weights $\m Gij$ capture the infection rate between all interacting individuals, and $\g$ is the average infection rate. 

\textbf{\color{blue} Null state}.\ First, we note that the SIS model exhibits a trivial fixed-point $\mathbf{x}^* = 0$, the \textit{healthy} state, in which $M_0(0) = M_2(0) = 0$. Together this classifies the SIS model into Case II of Table \ref{TableNull}, hence predicting the null-state Jacobian to follow $J \in \Ew$ with

\begin{equation}
\Omega = (0,0,0,0).
\label{SISTrivialOmega}
\end{equation} 

Using Eq.\ (\ref{S}) this provides $\S = \beta$, which for a fat-tailed $P(d)$, in which $\beta > 0$, predicts asymptotic instability. 

With this prediction our formalism retrieves an already well-established result, that the epidemic threshold of the SIS model vanishes under a scale-free topology \cite{PastorSatorras2001a}. Therefore, regardless of the specific parameters, $f_i, \g$, the pandemic state is always the only stable fixed-point of this model under degree-heterogeneous $A$. This is precisely the meaning of our observation here that $\mathbf{x}^* = (0,\dots,0)^{\top}$ is asymptotically unstable. However, while the original result was reported specifically for the Epidemic dynamics, using a dedicated analysis, in our formalism, this observation is but a special case of a broad class of potentially stable/unstable dynamics, all predictable via the $\Ew$ ensemble.  

\textbf{\color{blue} Pandemic state}.\ To obtain the relevant $J$ ensemble for the non-zero fixed-point/s, we seek the exponents $\Omega = (\eta, \mu, \nu, \rho)$. We begin by translating $M_q(x)$ into the relevant functions shown in (\ref{FunctionsFrame}), providing

\begin{eqnarray}
R(x) &=& -\dfrac{M_1(x)}{M_0(x)} = \dfrac{1 - x}{fx}
\label{SISR}
\\[7pt]
Y(x) &=& M_1(x)R^{\prime}(x) = \dfrac{x - 1}{fx^2}
\label{SISY}
\\[7pt]
Z(x) &=& R(x)M_2(x) = \dfrac{1}{f} - \dfrac{1}{f} x,
\label{SISZ}
\end{eqnarray}

where we used $f = \av f$ to denote the average recovery rate. Inverting $R(x)$ and $Z(x)$, we write 

\begin{eqnarray}
R^{-1}(x) &=& \dfrac{1}{fx + 1},
\label{SISRinv}
\\[7pt]
Z^{-1}(x) &=& 1 - f x,
\label{SISZinv}
\end{eqnarray}

allowing us to construct the Hahn expansions of (\ref{HahnFrame}) as

\begin{eqnarray}
M_2 \big( Z^{-1}(x) \big) &=& Z^{-1}(x) = 1 - fx
\label{SISM2Z}
\\[7pt]
Y \big( R^{-1}(x) \big) &=& \dfrac{R^{-1}(x) - 1}{f \times \big(R^{-1}(x) \big)^2} = 
-x - fx^2
\label{SISYR}
\\[7pt]
M_1 \big( R^{-1}(x) \big) &=& 1 - R^{-1}(x) = \dfrac{fx}{fx + 1} = fx - f^2x^2 + f^3x^3 - \cdots
\label{SISM1R}
\\[7pt]
M_2^{\prime} \big( R^{-1}(x) \big) &=& 1.
\label{SISM2R}
\end{eqnarray}
	
Here both $R(x)$ and $Z(x)$ are invertible, and therefore, the system exhibits only a single fixed-point apart from $\mathbf{x}^* = (0,\dots,0)^{\top}$. Each of the functions in (\ref{SISM2Z}) - (\ref{SISM2R}) is expressed as a Hahn power-series, in some cases a finite polynomial, \textit{e.g}., (\ref{SISM2Z}) or (\ref{SISYR}), and in others an infinite series, where we only write the leading terms around $x \rightarrow 0$. Here, coincidentally, the last function (\ref{SISM2R}) is a constant, \textit{i.e}.\ a trivial power-series in which the only participating power is $x^0$. We can list the relevant powers in these Hahn expansions as $\Psi_0 = 0, \Phi_0 = 1, \Pi_0 = 1$ and $\Theta_0 = 0$, which, using (\ref{ExponentsFrame}) provides

\begin{equation}
\begin{array}{cccc}
\mu = 2 - \Phi_0 = 1;
&
\nu = -\Pi_0 = -1;
&
\rho = -\Theta_0 = 0;
&
\eta = -\Psi_0 (\mu - \nu - \rho) = 0.
\end{array}
\label{SISOmega}
\end{equation}

Consequently the stability classifier in (\ref{S}) is $S = \beta(1 - 1 + 0 - 1 - 0) = - \beta$, which under $\beta > 0$ (\textit{i.e}.\ fat-tailed $P(d)$) predicts the asymptotic stability of the pandemic state, indeed, reconfirming Ref.\ \cite{PastorSatorras2001a}.

\subsection{Regulatory dynamics}
\label{SecRegulatory}

We used the Michaelis-Menten model to capture gene regulation in sub-cellular networks \cite{Karlebach2008}. Here, Eq.\ (\ref{Dynamics}) tracks the level of gene expression $x_i(t)$, as regulated via its interacting genes, providing 
		
\begin{equation}
\dod {x_i}{t} = -f_i x_i^a(t) + \g \sum_{j = 1}^N \m Aij \m Gij \frac{x_j^h(t)}{1 + x_j^h(t)}.
\label{Regulatory}
\end{equation}
		
The self-dynamic term $M_0(x_i,\m \f0i) = -f_ix_i^a$ captures biochemical processes \cite{Barzel2011}, such as degradation ($a = 1$) or dimerization ($a = 2$). The interaction terms $M_1(x_i) = 1, M_2(x_j) = x_j^h/(1 + x_j^h)$ describe genetic activation, a \textit{switch-like} dynamics, which ranges from $M_2(0) = 0$ to $M_2(x_j \rightarrow \infty) = 1$, capturing the activation of gene $i$ by gene $j$. The Hill coefficient $h$ governs the rate of saturation of $M_2(x)$, often associated with the level of cooperation in gene regulation \cite{Karlebach2008}. The exponents $a$ and $h$, are, in this case, expressed in the \textit{powers} $\m \Gamma qn$ of (\ref{Hahn}), and are hence rendered \textit{intrinsic}, thus taken to be uniform for all nodes/links (see Secs.\ \ref{SecMixedDynamics} and \ref{SecDistributedPowers}, where we break this assumption). The parameters $f_i,\m Gij$, on the other hand, capture the specific rates of all processes, which are potentially diverse across all nodes/links. Similarly, the average interaction rate $\g$ is also subject to external perturbation by the cell's environmental conditions.

\textbf{\color{blue} Null state}.\ Regulatory dynamics exhibit a trivial solution $\textbf{x}^* = (0,\dots,0)^{\top}$, capturing cell-death. Following (\ref{DiiTrivial}) and (\ref{WijTrivial}) we write

\begin{eqnarray}
\m Wii &=& af_i x^{a - 1} \Big|_{x = 0}
\label{DiiMMTrivial}
\\[7pt]
\m Wij &=& \m Aij \m wij \left. \dfrac{hx^{h - 1}}{(1 + x^h)^2} \right|_{x = 0}.
\label{WijMMTrivial}
\end{eqnarray}

Both terms vanish in case $a,h > 1$. This represents Case IV of Sec.\ \ref{TrivialSolution} (Table \ref{TableNull}), in which the linear regime is void. Under these conditions, the stability of the null state must be treated by resorting to higher orders, which are not within the scope of our formalism. Fortunately, thanks to the fact that the higher order expansion is around the trivial point $\textbf{x}^* = (0,\dots,0)^{\top}$, the analysis becomes straightforward. Indeed, for $x_i \rightarrow 0$, Eq.\ (\ref{Regulatory}) approaches

\begin{equation}
\dod{x_i}{t} = -f_i x_i^a + \g \sum_{j = 1}^N \m Aij \m Gij x_j^h 
\longrightarrow
\left\{
\begin{array}{lcc}
-f_i x_i^a &  & a < h
\\[8pt]
\displaystyle \g \sum_{j = 1}^N \m Aij \m Gij x_j^h &  & a \ge h
\end{array}
\right.,
\end{equation}

being dominated by the negative term if $a < h$, and by the positive term otherwise. For the specific case of $a = h$, both terms have similar dependence on $x_i$. However, since the positive interaction term scales with $d_i$ ($g\sum_{j = 1}^N \m Aij \m Gij = gd_i$), it will asymptotically dominate the dynamics ($d_i \gg f_i/g$ for sufficiently large hubs), predicting instability also under $a = h$. As a consequence the null state is stable if $a < h$ and unstable otherwise. 

The remaining scenario is the specific case where $a = h = 1$, precisely the dynamics we analyze in the main text under Regulatory. Here (\ref{DiiMMTrivial}) and (\ref{WijMMTrivial}) provide $\m Wii = f_i$ and $\m Wij = \m Aij \m Gij$, both independent of $d_i, d_j$. This corresponds to $J \in \Ew$, with

\begin{equation}
\Omega = (0,0,0,0),
\end{equation} 

an asymptotically unstable fixed-point, as per Case II of Sec.\ \ref{TrivialSolution}. Therefore, while $\textbf{x}^* = (0,\dots,0)^{\top}$ may generally be stable, if the system is large and heterogeneous it will inevitably avoid this undesired state.

\textbf{\color{blue} Active fixed-points}.\ We now return to our formalism to analyze the stability of the non-vanishing states. First, we construct the three functions summarized in (\ref{FunctionsFrame}):\

\begin{eqnarray}
R(x) &=& -\dfrac{M_1(x)}{M_0(x)} = \dfrac{1}{f x^a}
\label{RegulatoryR}
\\[7pt]
Y(x) &=& M_1(x)R^{\prime}(x) = - \dfrac{a}{f x^{a + 1}}
\label{RegulatoryY}
\\[7pt]
Z(x) &=& R(x)M_2(x) = \dfrac{x^h}{f (x^a + x^{a + h})},
\label{RegulatoryZ}
\end{eqnarray}

where, once again, we use $f = \av f$ to represent ensemble average over $f_i$. Inverting $R(x)$, we write 

\begin{equation}
R^{-1}(x) = f^{-\frac{1}{a}} x^{-\frac{1}{a}},
\label{RegulatoryRinv}
\end{equation}

allowing us to construct the Hahn expansions (\ref{HahnFrame})

\begin{eqnarray}
Y \big( R^{-1}(x) \big) &=& -\dfrac{a}{f} 
\left( \dfrac{1}{fx} \right)^{-\frac{a + 1}{a}} = 
a f^{\frac{1}{a}} x^{\frac{a + 1}{a}}
\label{RegulatoryYR}
\\[7pt]
M_1 \big( R^{-1}(x) \big) &=& 1 = x^0
\label{RegulatoryM1R}
\\[7pt]
M_2^{\prime} \big( R^{-1}(x) \big) &=& 
\dfrac{h f^{-\frac{h - 1}{a}}x^{-\frac{h - 1}{a}}}
{\Big( 1 + f^{-\frac{h}{a}}x^{-\frac{h}{a}} \Big)^2} = 
h f^{\frac{h + 1}{a}} x^{\frac{h + 1}{a}} - 
2h f^{\frac{2h + 1}{a}} x^{\frac{2h + 1}{a}} + \cdots.
\label{RegulatoryM2R}
\end{eqnarray}

In each of these expansions we write the leading terms in the $x \rightarrow 0$ limit:\ in (\ref{RegulatoryYR}) and (\ref{RegulatoryM1R}) the expansion features a single term, \textit{i.e}.\ a pure monomial, and in (\ref{RegulatoryM2R}) we show the first two terms of the relevant Hahn expansion. To obtain $\Omega$ we extract only the leading \textit{powers} $\Phi_0 = (a + 1)/a, \Pi_0 = 0, \Theta_0 = (h + 1)/a$, ignoring the \textit{coefficients}, \textit{e.g}., $af^{1/a}$ or $hf^{(h + 1)/a}$. We can now use (\ref{ExponentsFrame}) to extract the dynamic exponents as

\begin{equation}
\begin{array}{ccc}
\mu = 2 - \Phi_0 = \dfrac{a - 1}{a};
&
\nu = -\Pi_0 = 0;
&
\rho = -\Theta_0 = - \dfrac{h + 1}{a}.
\end{array}
\label{RegulatoryOmega}
\end{equation}

To obtain the final exponent $\eta$ we must calculate $M_2(Z^{-1}(x))$, requiring us to invert the function $Z(x)$ in (\ref{RegulatoryZ}). This becomes prohibitively complicated under a general $a$ and $h$, however, as we are only focused on the leading powers of $M_2(Z^{-1}(x))$, we can advance using an asymptotic analysis. Similar to the trivial fixed-point analysis, we once again, distinguish between $a \ge h$ and $a < h$. 

%%%%%%%%%%%%%%%%%%%%%%%%%%%%%%%%%%%%%%%%%%%%%%%%%%%%%%%%%%%%%%%%%%%%%%%
\begin{figure}[h!]
\includegraphics[width=16cm]{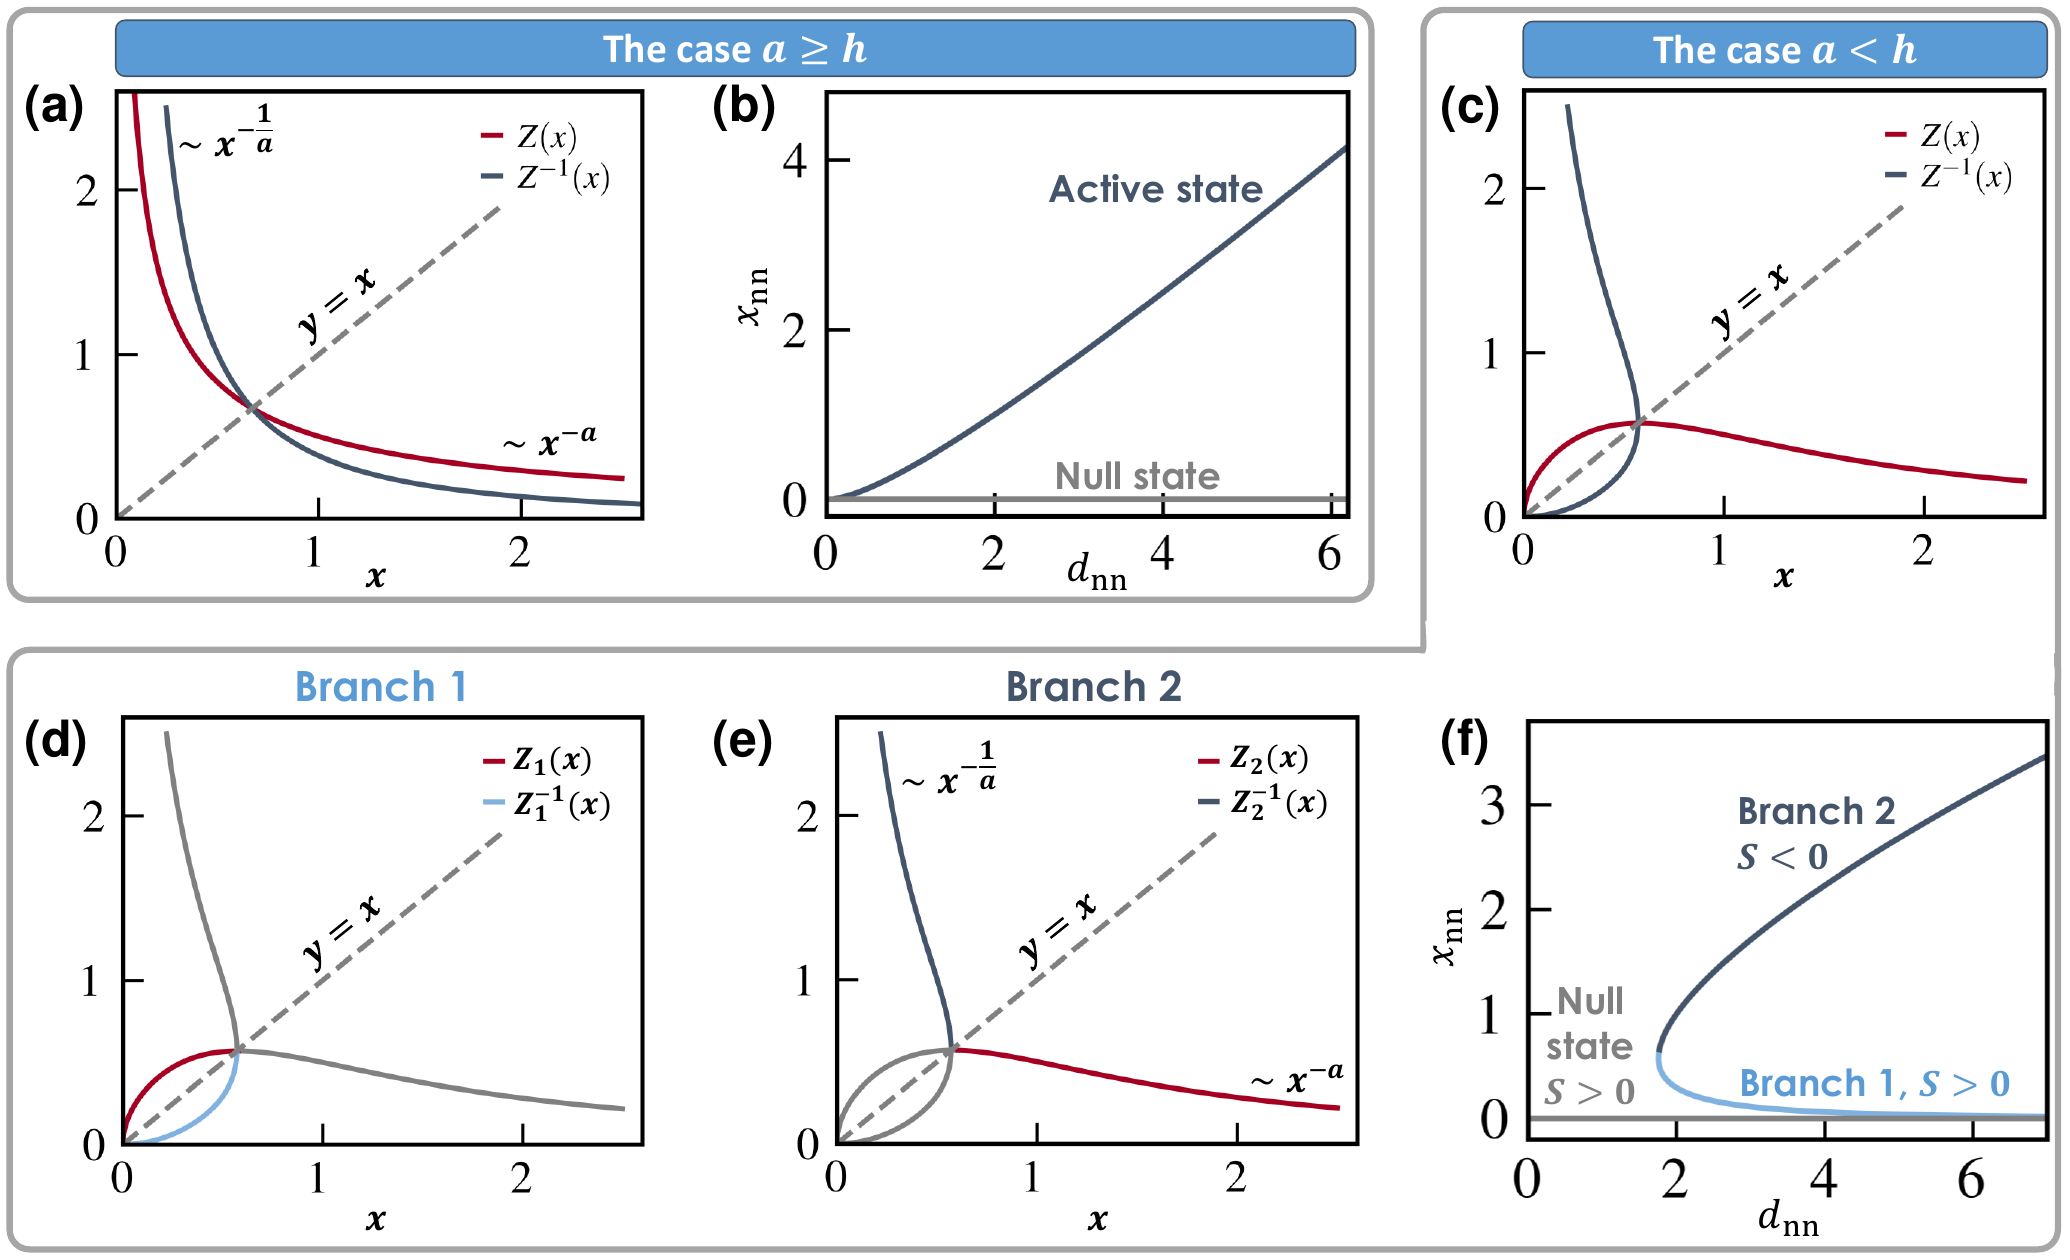}
\caption{\footnotesize \color{blue} \textbf{Analyzing $Z(x)$ in Regulatory dynamics}.\
(a) $Z(x)$ in (\ref{RegulatoryZ}) vs.\ $x$ (red) for $a \ge h$, set here to $a = 1,h = 1/2$. Here $Z(x)$ is monotonous and therefore we can obtain its inverse $Z^{-1}(x)$ for all $x$ (blue). Using the fact that $Z(x \to \infty) \sim x^{-a}$, we can extrapolate that its inverse has $Z^{-1}(x \to 0) \sim x^{-1/a}$.
(b) The nearest neighbor fixed-point activity $x_{\nn}$ vs.\ $\knn$, as obtained for Regulatory dynamics (\ref{Regulatory}) with $a > h$. Following Eq.\ (\ref{Zchi}), the limit $Z^{-1}(x \to 0)$ captured the active state (blue) in the limit of large $\knn$, predicting $\knn \sim x_{\nn}^{1/a}$. The null-state is also shown (grey).
(c) For $a < h$, $Z(x)$ is not monotonous (red) and therefore $Z^{-1}(x)$ is undefined (blue). To treat this we divide $Z(x)$ into two branches:\ Branch 1 to the left of the maximum point; Branch 2 to its right.
(d) In Branch 1 we have $Z_1(x \to 0) \sim x^{h - a}$ (red), providing $Z_1^{-1}(x \to 0) \sim x^{1/(h - a)}$ (light blue).
(e) In Branch 2 we have $Z_2(x \to \infty) \sim x^{-a}$ (red), and hence $Z_2^{-1}(x \to 0) \sim x^{-1/a}$ (dark blue).
(f) $x_{\nn}$ vs.\ $\knn$ under $a < h$. We observe three states:\ null-state (grey), active state (dark blue), intermediate state (light blue). Branch 1 has $Z_1^{-1}(x) \to 0$ in the limit of small $x$, describing a state in which $x_{\nn}$ decreases with $\knn$. This corresponds to the intermediate state, for which we obtain $S > 0$, \textit{i.e}.\ instability. Branch 2 has $Z_2^{-1}(x) \to \infty$, capturing a positive scaling between $\knn$ and $x_{\nn}$. Therefore Branch 2 is related to the active state, which is asymptotically stable ($S < 0$).
} 
\label{FigureRegulatory}
\end{figure}
%%%%%%%%%%%%%%%%%%%%%%%%%%%%%%%%%%%%%%%%%%%%%%%%%%%%%%%%%%%%%%%%%%%%%%%

\textbf{\color{blue} Regulatory dynamics under $a \ge h$}.\ 
Under these conditions $Z(x)$ is monotonous and therefore invertible. For $x \rightarrow \infty$ we have $Z(x) \sim x^{-a}$, which approaches zero (Fig.\ \ref{FigureRegulatory}a, red). Therefore, the inverse $Z^{-1}(x)$ tends to infinity as $x \rightarrow 0$ (blue). The form of this divergence can be obtained by mirroring the large $x$ behavior of $Z(x)$, providing $Z^{-1}(x) \sim x^{-1/a}$. This enables us to construct the final Hahn expansion to leading order as

\begin{equation}
M_2 \big( Z^{-1}(x) \big) \sim \dfrac{x^{-\frac{h}{a}}}{1 + x^{-\frac{h}{a}}} 
\sim 1 - x^{\frac{h}{a}} + \dots,
\label{Phi1_Regu}
\end{equation}  

in which the leading power is $\Psi_0 = 0$. As a result, we obtain, using (\ref{ExponentsFrame}) our final exponent

\begin{equation}
\eta = -\Psi_0 (\mu - \nu - \rho) = 0.
\label{RegulatoryEta1}
\end{equation}

Collecting the other exponents calculated above in (\ref{RegulatoryOmega}), we derive the stability classifier

\begin{equation}
S = \beta 
\left( 1 + 0 - \dfrac{h + 1}{a} - \frac{a - 1}{a} - 0 \right) = -\dfrac{h}{a}\beta < 0,
\end{equation}

indicating that for $a \ge h$ the non-trivial fixed-point is asymptotically stable.

\textbf{\color{blue} Regulatory dynamics under $a < h$}.\ 
For $a < h$, the function $Z(x)$ in (\ref{RegulatoryZ}) is non-monotonous, its inverse is undefined, and hence the system can potentially reside in multiple fixed-points. As an example, in Fig.\ \ref{FigureRegulatory}c we present $Z(x)$ for a specific choice of $f = 1, a = 3/2, h = 2$ (red), finding that it is, indeed, non-invertible. We therefore divide $Z(x)$ into its two branches, as shown in Fig.\ \ref{FigRInverse}:\ Branch 1 - from $x = 0$ upto the maximum point, and Branch 2 - from the maximum point to $x \rightarrow \infty$. This allows us to construct the two functions, $Z_1(x)$ (Fig.\ \ref{FigureRegulatory}d) and $Z_2(x)$ (Fig.\ \ref{FigureRegulatory}e), each of which \textit{is} invertible, and whose inverse function is associated with a distinct fixed-point of the system.

First we analyze $Z_1(x)$ (Fig.\ \ref{FigureRegulatory}d, red). As we are interested in the leading power of $M_2(Z_1^{-1}(x))$, we focus on the the behavior around $x \rightarrow 0$. Using (\ref{RegulatoryZ}) we write

\begin{equation}
Z_1(x \rightarrow 0) = x^{h - a} + \dots,
\label{RegulatoryZ1}
\end{equation}

where we include only the leading term, and, for simplicity, set $f = 1$. We therefore have 

\begin{equation}
Z_1^{-1}(x \rightarrow 0) = x^{\frac{1}{h - a}} + \dots,
\label{RegulatoryZ1Inv}
\end{equation} 

shown in Fig.\ \ref{FigureRegulatory}d (light blue), and consequently

\begin{equation}
M_2 \big( Z_1^{-1}(x \rightarrow 0) \big) = x^{\frac{h}{h - a}} + \dots.
\label{Phi2_Regu}
\end{equation}

This provides, for Branch 1, $\Psi_0 = h/(h - a)$, which, taking $\mu,\nu,\rho$ from (\ref{RegulatoryOmega}), predicts

\begin{equation}
\eta = -\Psi_0 (\mu - \nu - \rho) = \dfrac{h(a + h)}{a(a - h)}.
\label{RegulatoryEta1}
\end{equation}

Collecting all exponents we obtain

\begin{equation}
S = \beta 
\left(
1 + 0 - \dfrac{h + 1}{a} - \frac{a - 1}{a} - \dfrac{h(a + h)}{a(a - h)}
\right) = 2 \dfrac{h(a + 1)}{a(h - a)}.
\end{equation}

Under the condition $a < h$, $S$ is guaranteed to be positive. Therefore, Branch 1 is asymptotically unstable.

The fixed-point captured by Branch 1 has $Z_1^{-1}(x \rightarrow 0) \rightarrow 0$. This captures a state in which the nearest neighbor activity $x_{\nn}$ tends to zero as $\knn$ is increased. Indeed in Eq.\ (\ref{Zchi}) we have $x_{\nn} = Z^{-1}(\q_{\nn})$, in which $q_{\nn} \sim \knn^{-1}$ tends to zero in the limit $\knn \to \infty$, indicating that $Z_1^{-1}(x \rightarrow 0)$ captures the asymptotic behavior of $x_{\nn}$. This behavior, links Branch 1 to the intermediate state in the one-dimensional bifurcation diagram of Fig.\ \ref{FigureRegulatory}f (light blue), which is, indeed, characterized by $x_{\nn} \to 0$. This state is unstable in the low-dimensional system, and as our formalism now shows, it is also unstable in the asymptotic limit, via our ensemble $\Ew$.

Next, we analyze Branch 2, $Z_2(x)$, capturing the part of $Z(x)$ to the right of the maximum point (Fig.\ \ref{FigureRegulatory}e, red). Its asymptotic behavior is observed in the limit $x \rightarrow \infty$, where we have $Z_2(x) \sim x^{-a}$. Mirroring this behavior to the inverse $Z_2^{-1}(x)$, we have $Z_2^{-1}(x \rightarrow 0) \sim x^{-1/a}$ (dark blue), leading to

\begin{equation}
M_2 \big( Z^{-1}(x) \big) \sim \dfrac{x^{-\frac{h}{a}}}{1 + x^{-\frac{h}{a}}} 
\sim 1 - x^{\frac{h}{a}} + \dots,
\end{equation}  

namely $\Psi_0 = 0$. Hence, for Branch 2 we have

\begin{equation}
\eta = -\Psi_0 (\mu - \nu - \rho) = 0.
\label{RegulatoryEta2}
\end{equation}

Together with (\ref{RegulatoryOmega}) this provides

\begin{equation}
S = \beta 
\left( 1 + 0 - \dfrac{h + 1}{a} - \frac{a - 1}{a} - 0 \right) = -\dfrac{h}{a}\beta < 0,
\end{equation}

predicting, for this branch, that it is asymptotically stable. 

This branch, in which $Z^{-1}(x \rightarrow 0) \rightarrow \infty$ captures a state in which $x_{\nn}$ increases with $\knn$, corresponding to the \textit{active} state of Fig.\ \ref{FigureRegulatory}f (dark blue). In a low-dimensional system, the stability of this state depends on the system's specific parameters, \textit{i.e}.\ $f_i,\g$. Yet, our formalism shows that this state becomes asymptotically stable for large heterogeneous networks.

\subsection{Population 1 dynamics}
\label{SecPopulation1}

We consider mutualistic eco-systems, such as plant-pollinator networks or microbial communities, in which the interacting species exhibit symbiotic relationships. The species populations follow the dynamic equation 
	
\begin{equation}
\dod {x_i}{t} = b_i x_i(t) \left(1 - \frac{x_i(t)}{c_i} \right)
+ \g \sum\limits_{j = 1}^N \m Aij \m Gij x_i(t) F\big( x_j(t) \big).
\label{MDynamics}
\end{equation}  
		
The self-dynamics $M_0(x_i,\m \f0i) = b_i x_i (1 - x_i/c_i)$ captures logistic growth, driven by parameter $b_i$, the growth rate, and $c_i$, the environment carrying capacity. The mutualistic interactions are captured by $M_1(x_i) = x_i$ and $M_2(x_j) = F(x_j)$, where $F(x_j)$ represents the {\it functional response}, describing the positive impact that species $j$ has on species $i$. This functional response can take one of several forms, Holling types I - III \cite{Holling1959}:\ 

\begin{equation}
\begin{array}{ccccc}
F_{\rm I}(x) = x,
& \,\,\,\,\,\,\,\,\, &
F_{\rm II}(x) = \dfrac{x}{1 + x},
& \,\,\,\,\,\,\,\,\, &
F_{\rm III}(x) = \dfrac{x^h}{1 + x^h}
\end{array},
\label{Holling}
\end{equation}

type I featuring a linear response, and types II,III describing a saturating impact of $j$ on $i$. In our simulations we used Type II interactions, therefore $M_2(x_j) = x_j/(1 + x_j)$. 

\textbf{\color{blue} Null state}.\
Equation (\ref{MDynamics}) has a trivial fixed-point $\x^* = (0,\dots,0)^{\top}$, in which $M_0(x) = M_1(x) = M_2(x) = 0$. This corresponds to Case III in Table \ref{TableNull}, in which the null-state is unstable. This instability, we emphasize, is different from our asymptotic instability of $S > 0$, as it is independent of network size ($N$) or of degree heterogeneity ($P(d)$). Here, even if we consider the one dimensional version of (\ref{MDynamics})

\begin{equation}
\dod {x}{t} = b \left( 1 - \dfrac{x}{c} \right) + \g x F(x),
\label{MDynamics1D}
\end{equation}

we find that $x = 0$ is unstable, independently of parameters $b,c,\g$. This is despite that fact that the one-dimensional (\ref{MDynamics1D}) is certainly not in the relevant asymptotic regime of $N \to \infty$ and $P(d)$ fat-tailed. Therefore, the null-state instability in this dynamics is unrelated to $\Ew$. Fortunately, it be directly analyzed without the need for our more advanced toolbox. 

\textbf{\color{blue} Active state}.\ 
Next we analyze the non-vanishing fixed-point/s of (\ref{MDynamics}) using our formalism. For $R(x), Y(x)$ and $Z(x)$ we have

\begin{eqnarray}
R(x) &=& -\dfrac{M_1(x)}{M_0(x)} = \dfrac{1}{x - 1}
\label{MR}
\\[5pt]
Y(x) &=& M_1(x)R^{\prime}(x) = - \dfrac{x}{(x - 1)^2}
\label{MY}
\end{eqnarray}

\begin{eqnarray}
Z(x) &=& R(x)M_2(x) = \dfrac{x}{x^2 - 1},
\label{MZ}
\end{eqnarray}

where for simplicity we set $b_i = c_i = 1$, as indeed these parameters have no effect on the scaling $\Omega$. Inverting $R(x)$ and $Z(x)$, we write 

\begin{eqnarray}
R^{-1}(x) &=& \dfrac{x + 1}{x},
\label{MRinv}
\\[5pt]
Z^{-1}(x) &=& \dfrac{1}{2x} \left(1 \pm \sqrt{1 + 4x^2} \right).
\label{MZinv}
\end{eqnarray}

Note that, similar to Regulatory, here too, $Z(x)$ is non-invertible, and hence we have two branches ($\pm$) for $Z^{-1}(x)$. In this case, however, the \textit{minus} branch corresponds to a purely negative fixed-point, which is physically irrelevant. Therefore, apart from the null fixed-point analyzed above, we are only left with the \textit{plus} branch of (\ref{MZinv}). Taking this branch we construct the Hahn expansions of (\ref{HahnFrame}) as

\begin{eqnarray}
M_2 \big( Z^{-1}(x) \big) &=& \dfrac{Z^{-1}(x)}{1 + Z^{-1}(x)} = 
\dfrac{1 + \sqrt{1 + 4x^2}}{2x + 1 + \sqrt{1 + 4x^2}} =
1 - x + \cdots
\label{MM2Z}
\\[5pt]
Y \big( R^{-1}(x) \big) &=& - \dfrac{R^{-1}(x)}{\big( R^{-1}(x) - 1 \big)^2} = 
x + x^2
\label{MYR}
\\[5pt]
M_1 \big( R^{-1}(x) \big) &=& \dfrac{x + 1}{x} = x^{-1} + 1
\label{MM1R}
\\[5pt]
M_2^{\prime} \big( R^{-1}(x) \big) &=& \dfrac{1}{\big( R^{-1}(x) + 1 \big)^2} =
\dfrac{x^2}{4x^2 + 4x + 1} = x^2 - 4x^3 + \cdots,
\label{MM2R}
\end{eqnarray}

whose leading powers are $\Psi_0 = 0, \Phi_0 = 1, \Pi_0 = -1$ and $\Theta_0 = 2$. Consequently, the dynamic exponents in (\ref{ExponentsFrame}) follow

\begin{equation}
\begin{array}{cccc}
\mu = 2 - \Phi_0 = 1;
&
\nu = -\Pi_0 = 1
&
\rho = -\Theta_0 = -2
&
\eta = -\Psi_0(\mu - \nu - \rho) = 0.
\end{array}
\label{Pop1Omega}
\end{equation}

As analyzed in Sec.\ \ref{ImpactPkKappa} we have, in Population 1, $\eta = 0$. This is due both to the \textit{Bounded activities} ($0 < x_i < c_i$) and to the \textit{Saturating} nature of the interaction function. Collecting all exponents we extract the stability classifier from (\ref{S}) as $S = \beta (1 + 1 - 2 - 1 - 0) = -\beta < 0$.

\begin{table}[t]
\includegraphics[width=16cm]{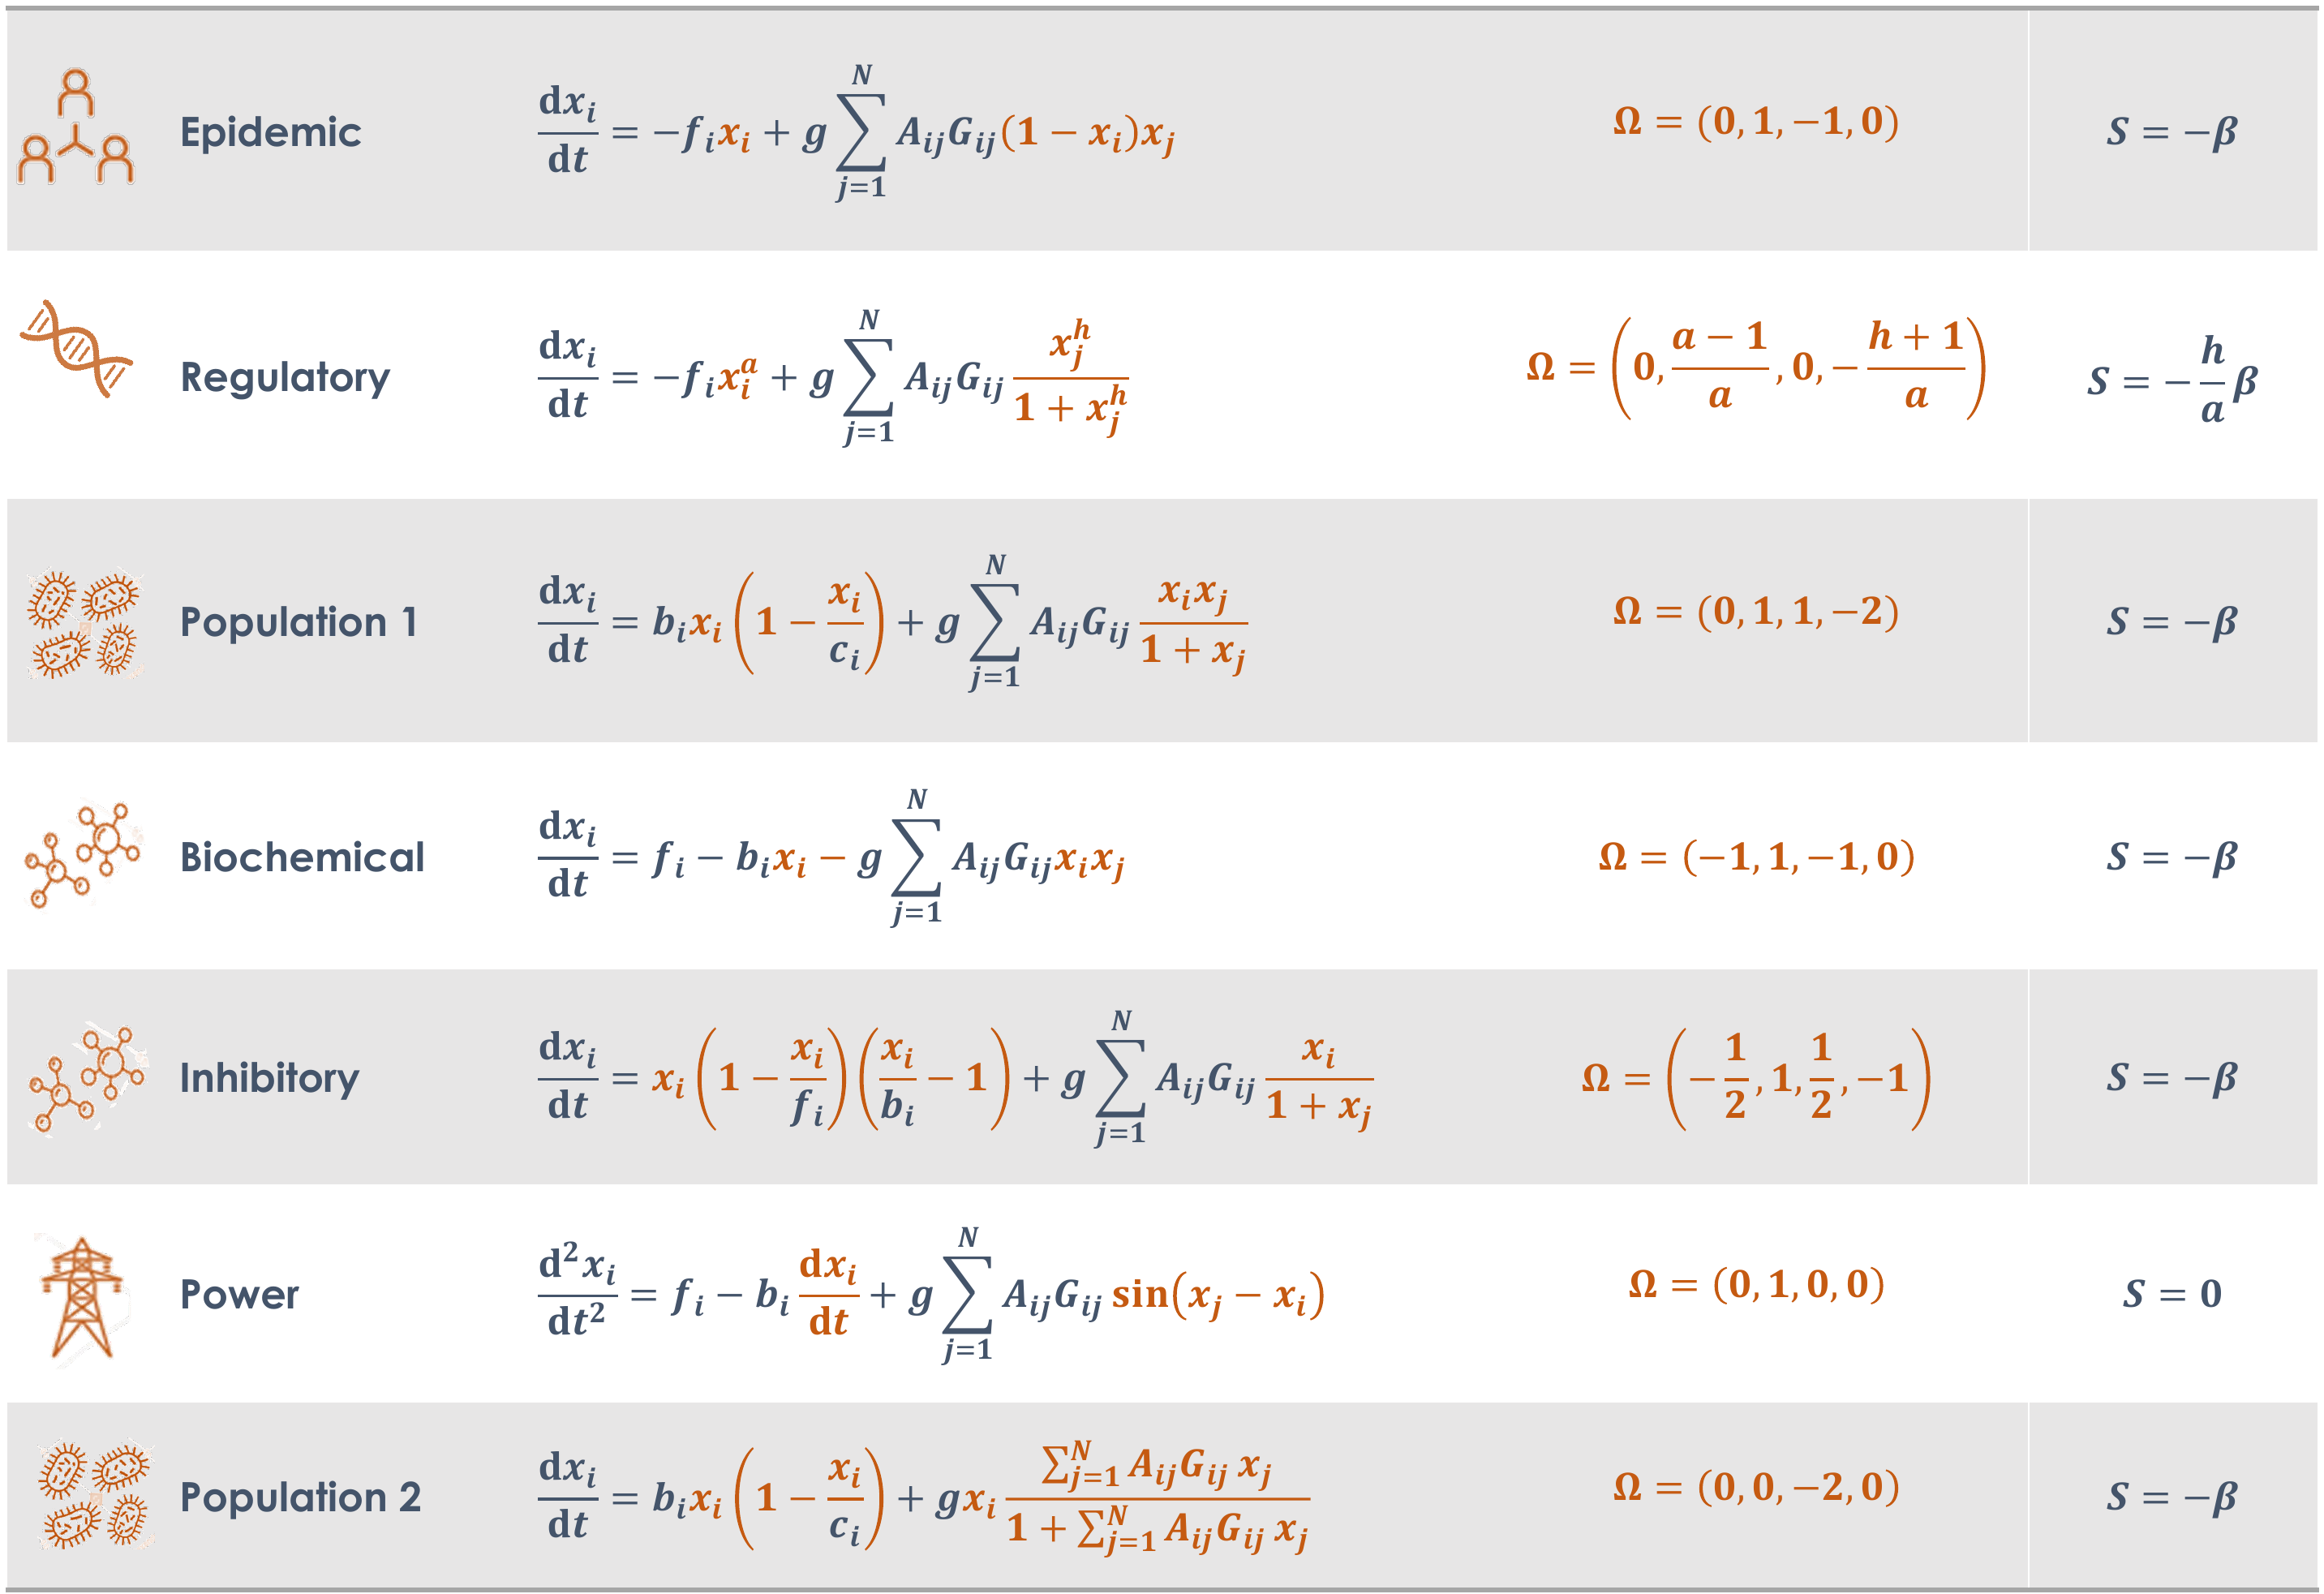}
\caption{\footnotesize \color{blue} \textbf{Dynamic models - summary}.
Our seven dynamic models and their associated exponents $\Omega$, as calculated around their active fixed point $\x_1$. For each model we also show the stability classifier $S$. Parameters ($f_i,b_i,$ etc.) appear in blue and the nonlinear functions themselves in orange. Only the orange terms feed into $\Omega$. The analysis of Power and Population 2, both beyond the scope of Eq.\ (\ref{Eq3}), appears in Sec.\ \ref{SecExtendedDynamics}.} 
\label{DynamicsTable}
\end{table}

\subsection{Biochemical dynamics}

As a Biochemical model we consider protein-protein interactions (PPI), which are driven by three processes:\ $\emptyset \rightarrow P_i$, describing the synthesis of the $i$th protein $P_i$ at a rate $f_i$; $P_i \rightarrow \emptyset$, describing protein degradation at rate $b_i; P_i + P_j \rightleftharpoons P_iP_j$ describing the binding and unbinding of a pair of interacting proteins at rates $\m Bij$ and $\m Uij$ respectively. The hetero-dimer $P_iP_j$ undergoes degradation $P_iP_j \rightarrow \emptyset$ at rate $\m Qij$. Using mass-action-kinetics we derive the dynamical equations for this system, providing \cite{voit2000,Barzel2011} 
	
\begin{eqnarray}
\dod {x_i}{t} &=& f_i - b_i x_i(t) + 
\sum_{j = 1}^N  \m Uij \m xij(t) - \sum_{j = 1}^N \m Aij \m Bij x_i(t)x_j(t)
\\[7pt]
\label{PPI1}
\dod {\m xij}{t} &=& \m Bij \m Aij x_i(t)x_j(t) - (\m Uij + \m Qij) \m xij(t),
\label{PPI2}
\end{eqnarray}	

where $x_i(t)$ is the concentration of $P_i$ and $\m xij(t)$ is the concentration of the hetero-dimer $P_iP_j$. Under time-scale separation we assume that the hetero-dimer concentration is at steady-state, setting $\dif \m xij/\dif t = 0$ in (\ref{PPI2}). This provides us with
 
\begin{equation}
\dod {x_i}{t} = f_i - b_i x_i(t) - \g \sum_{j = 1}^N \m Aij \m Gij x_i(t)x_j(t),
\label{PPI3}
\end{equation}

where the effective binding rate is $\g \m Gij = \m Qij \m Bij / (\m Uij + \m Qij)$. This has the form of Eq.\ (\ref{Eq3}), with $M_0(x_i,\m \f0i) = f_i - b_i x_i$, whose parameters are $\{f_i,b_i\}$, $M_1(x_i) = x_i$ and $M_2(x_j) = x_j$. Denoting the average rates by $f = \av f, b = \av b$, we write the dynamic functions (\ref{FunctionsFrame}) as
	
\begin{eqnarray}
R(x) &=& -\dfrac{M_1(x)}{M_0(x)} = \dfrac{x}{f - b x}
\label{PPIR}
\\[7pt]
Y(x) &=& M_1(x)R^{\prime}(x) = - \dfrac{ f x}{\big(  f - b x \big)^2}
\label{PPIY}
\\[7pt]
Z(x) &=& R(x)M_2(x) = \dfrac{x^2}{f - b x}.
\label{PPIZ}
\end{eqnarray}
	
The inverse functions are, therefore
	
\begin{eqnarray}
R^{-1}(x) &=& \dfrac{f x}{1 + b x}
\label{PPIRinv}
\\[7pt]
Z^{-1}(x) &=& \dfrac{b}{2} x \left(-1 + \sqrt{1 + \dfrac{4f}{b^2 x}} \right),
\label{PPIZinv}
\end{eqnarray}

where in $Z^{-1}(x)$ we choose the positive solution, corresponding to the positive fixed-point of (\ref{PPI3}), as we did in our analysis of Population 1 above. We can now compose the functions in (\ref{HahnFrame}), obtaining

\begin{eqnarray}
M_2 \big( Z^{-1}(x) \big) &=& Z^{-1}(x) = 
\sqrt{f} x^{\frac{1}{2}} + \dfrac{b^2}{8 \sqrt{f}} x^{\frac{3}{2}} +
\cdots
\label{PPIM2Z}
\\[7pt]
Y \big( R^{-1}(x) \big) &=& - \dfrac{f R^{-1}(x)}{\big( f - b R^{-1}(x) \big)^2} = f x + fb x^2
\label{PPIYR}
\\[7pt]
M_1 \big( R^{-1}(x) \big) &=& - \dfrac{f x}{1 + b x} = - f x + fb x^2 +
\cdots 
\label{PPIM1R}
\\[7pt]
M_2^{\prime} \big( R^{-1}(x) \big) &=& 1,
\label{PPIM2R}
\end{eqnarray}

allowing us to extract the leading powers as $\Psi_0 = 1/2, \Phi_0 = 1, \Pi_0 = 1$ and $\Theta_0 = 0$. These powers provide the Biochemical dynamic exponents via (\ref{ExponentsFrame}) as

\begin{equation}
\begin{array}{cccc}
\mu = 2 - \Phi_0 = 1;
&
\nu = -\Pi_0 = -1;
&
\rho = -\Theta_0 = 0;
&
\eta = -\Psi_0(\mu - \nu - \rho) = -1
\end{array}.
\label{BioOmega}
\end{equation}

As predicted, these exponents are independent of the parameters $f,b$, intrinsic to the Biochemical dynamics. Here, since the interactions are adversarial, as indicated by the $-\g$ pre-factor preceding the interaction term in (\ref{PPI3}), we have $\s = 0$. Therefore, we use (\ref{Sneg}) to obtain the stability classifier, providing us with $S = \beta (-1 + 0 - 1 + 1) = -\beta$, \textit{i.e}.\ asymptotically stable.

\subsection{Inhibitory dynamics}

To model inhibition, \textit{e.g}., between genes \cite{Karlebach2008} or between hosts and pathogens \cite{Wodarz2002}, we use 

\begin{equation}
\dod{x_i}{t} = x_i(t) \left( 1 - \dfrac{x_i(t)}{f_i} \right) \left( \dfrac{x_i(t)}{b_i} - 1 \right) + 
\g \sum_{j = 1}^N \m Aij \m Gij x_i(t) \dfrac{1}{1 + x_j(t)}.
\label{Inhibition}
\end{equation}

The self dynamics captures logistic growth, similar to Population 1, but here, also incorporating the Allee effect \cite{Allee1932}, which balances competition with the potentially added benefit of the \textit{tribe}. The competition is expressed in $M_0(x_i)$ through the negative growth occurring when $x_i > f_i$, \textit{i.e}.\ when $x_i$ exceeds the limited carrying capacity of the environment. This competition, however, is overcome by the enhanced growth at $b_i < x_i < f_i$, capturing the cooperative benefit of $i$ from being surrounded by a greater $i$ population, \textit{e.g}., hunting in pacts. Hence, Eq.\ (\ref{Inhibition}) is relevant under $b_i \le f_i$, predicting suppressed growth when $0 < x_i < b_i$ or $x_i > f_i$, and positive growth in the mid-range $b_i < x_i < f_i$. The interaction dynamics describes inhibition:\ $i$ grows linearly with its own instantaneous population $x_i$, but at a rate which approaches zero as $x_j \to \infty$. Consequently, the greater is $x_j$ the lower is $i$'s reproduction rate.

\textbf{\color{blue} Null state}.\
In (\ref{Inhibition}) the null state $\x^* = (0,\dots,0)^{\top}$ has $M_0^{\prime}(0) = -1$ and $M_2(0) = 1$, both non-zero. This adheres to Case I in Sec.\ \ref{TrivialSolution}, predicting $\m Wii \sim -1 + d_i$ and $\m Wij = 0$. Consequently, as Table \ref{TableNull} indicates, the null state is asymptotically unstable. This is indeed supported by Fig.\ 5 of the main text, where we show that the active state persists under arbitrary parameter perturbation.   

\textbf{\color{blue} Active state}.\
To analyze the active state of (\ref{Inhibition}) we first rewrite its self-dynamics in the Hahn form of Eq.\ (\ref{Hahn}) as

\begin{equation}
M_0(x_i,\f_i) = -x_i + B_i x_i^2 - Q_i x_i^3,
\end{equation}

where $B_i = (f_i + b_i)/f_ib_i$ and $Q_i = 1/f_ib_i$. Denoting $\av B = B$ and $\av Q = Q$, we construct the dynamic functions of (\ref{FunctionsFrame}), obtaining
	
\begin{eqnarray}
R(x) &=& -\dfrac{M_1(x)}{M_0(x)} = \dfrac{1}{1 - Bx + Qx^2}
\label{InhibitR}
\\[7pt]
Y(x) &=& M_1(x)R^{\prime}(x) = \dfrac{Bx - 2Qx^2}{\big( 1 - Bx + Qx^2 \big)^2}
\label{InhibitY}
\\[7pt]
Z(x) &=& R(x)M_2(x) = \dfrac{1}{1 + (1 - B)x + (Q - B) x^2 + Qx^3}.
\label{InhibitZ}
\end{eqnarray}

The inverse function $R^{-1}(x)$ takes the form

\begin{equation}
R^{-1}(x) = \dfrac{B + \sqrt{B^2 - 4Q + \dfrac{4Q}{x}}}{2Q},
\label{RinvInhibition}
\end{equation}

where once again, we omit the negative branch, as it represents a negative, and hence irrelevant, fixed-point. In the limit $x \to 0$ we have

\begin{equation}
R^{-1}(x) \approx Q^{-\frac{1}{2}} x^{-\frac{1}{2}}.
\label{RinvInhibitionLimit}
\end{equation}

Inverting $Z(x)$ in (\ref{InhibitZ}) is non-tractable analytically, however, as we only need to evaluate $Z^{-1}(x)$ in the limit of $x \to 0$, we can simplify the calculation, by seeking only the relevant leading terms. In Fig.\ \ref{FigureInhibitory} we show $Z(x)$ (red) and its inverse $Z^{-1}(x)$ (blue). Since $Z(x)$ is non-monotonic, its inverse is undefined, indeed showing several branches (Fig.\ \ref{FigureInhibitory}b):\ Branch 1, the top branch, which diverges in the limit $x \to 0$, Branch 2, intermediate, and Branch 3, for which $Z^{-1}(x) < 0$. Of these, the only relevant branch is Branch 1, as it is the only one covering the $x \to 0$ regime. The meaning is that, while $Z(x)$ is non-invertible for all $x \in \mathbb R$, the limit $Z^{-1}(x \to 0)$ \textit{is} well-defined, as the function is locally invertible around $x = 0$. Examining the corresponding branch in $Z(x)$ we observe that $Z^{-1}(x \to 0)$ is the mirror image of the original function $Z(x)$ in the limit $Z(x \to \infty)$ (Branch 1 in Fig.\ \ref{FigureInhibitory}a). Using (\ref{InhibitZ}) we write $Z(x \to \infty) \sim Q^{-1}x^{-3}$, and therefore we have

\begin{equation}
Z^{-1}(x \to 0) \sim Q^{-\frac{1}{3}}x^{-\frac{1}{3}}.
\label{ZinvInhibitionLimit}
\end{equation}

%%%%%%%%%%%%%%%%%%%%%%%%%%%%%%%%%%%%%%%%%%%%%%%%%%%%%%%%%%%%%%%%%%%%%%%
\begin{figure}[h!]
\includegraphics[width=16cm]{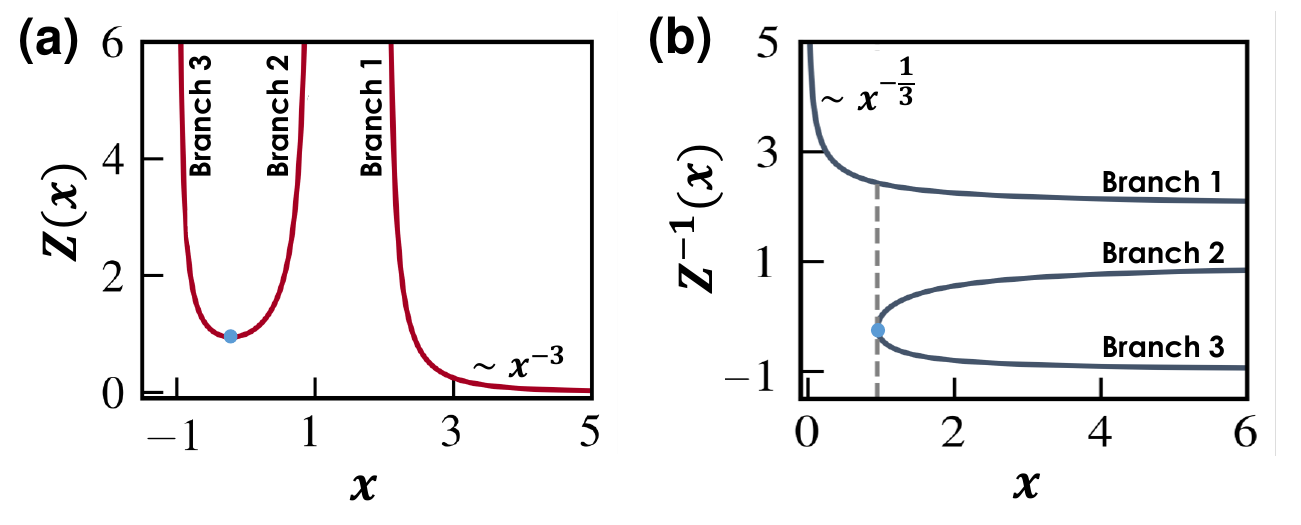}
\vspace{-10mm}
\caption{\footnotesize \color{blue} \textbf{Analyzing $Z(x)$ under Inhibitory dynamics}.\
(a) $Z(x)$ in (\ref{InhibitZ}) vs.\ $x$. The function is divided into three branches, separated by the minimum point (blue dot) between Branches 3 and 2, and by the asymptotic divergence between Branch 2 and Branch 1.
(b) $Z^{-1}(x)$ and its division into the corresponding three branches. To the right of the grey dashed line we observe overlapping solutions, and hence $Z^{-1}(x)$ is undefined. However, the limit $Z^{-1}(x \to 0)$ is well-defined, as in this regime, to the left of the dashed line, only Branch 1 is relevant. The limit $x \to 0$ in $Z^{-1}(x)$ is the mirror image of the limit $x \to \infty$ in $Z(x)$. Therefore, using the fact that $Z(x \to \infty) \sim x^{-3}$ we extrapolate $Z^{-1}(x \to 0) \sim x^{-1/3}$, as appears in Eq.\ (\ref{ZinvInhibitionLimit}). 
} 
\label{FigureInhibitory}
\end{figure}
%%%%%%%%%%%%%%%%%%%%%%%%%%%%%%%%%%%%%%%%%%%%%%%%%%%%%%%%%%%%%%%%%%%%%%%

With (\ref{RinvInhibitionLimit}) and (\ref{ZinvInhibitionLimit}) at hand we can now construct the relevant dynamic functions of (\ref{HahnFrame}), obtaining

\begin{eqnarray}
M_2 \big( Z^{-1}(x) \big) &=& \dfrac{1}{1 + Z^{-1}(x)} \sim 
\dfrac{1}{1 + Q^{-\frac{1}{3}}x^{-\frac{1}{3}}} \sim x^{\frac{1}{3}} + \cdots
\label{InhibitM2Z}
\\[7pt]
Y \big( R^{-1}(x) \big) &=& \dfrac{B R^{-1}(x) - 2Q \big( R^{-1}(x) \big)^2}
{\Big( 1 - B R^{-1}(x) + Q\big( R^{-1}(x) \big)^2 \Big)^2}
\nonumber \\[7pt]
&\sim& \dfrac{B Q^{-\frac{1}{2}} x^{-\frac{1}{2}} - 2 x^{-1}}
{\Big( 1 - B Q^{-\frac{1}{2}} x^{-\frac{1}{2}} + x^{-1} \Big)^2} \sim x + \cdots
\label{InhibitYR}
\end{eqnarray}

\begin{eqnarray}
M_1 \big( R^{-1}(x) \big) &=& R^{-1}(x) \sim  x^{-\frac{1}{2}} + \cdots
\label{InhibitM1R}
\\[7pt]
M_2^{\prime} \big( R^{-1}(x) \big) &=& - \dfrac{1}{\big( 1 + R^{-1}(x) \big)^2} \sim 
- \dfrac{1}{\big(1 + Q^{-\frac{1}{2}} x^{-\frac{1}{2}} \big)^2} \sim x + \cdots.
\label{InhibitM2R}
\end{eqnarray}

From here we extract the leading powers as $\Psi_0 = 1/3, \Phi_0 = 1, \Pi_0 = -1/2$ and $\Theta_0 = 1$, which using (\ref{ExponentsFrame}), predicts 

\begin{equation}
\begin{array}{cccc}
\mu = 2 - \Phi_0 = 1
&
\nu = -\Pi_0 = \dfrac{1}{2}
&
\rho = -\Theta_0 = -1
&
\eta = -\Psi_0(\mu - \nu - \rho) = -\dfrac{1}{2}.
\end{array}
\label{InhibitOmega}
\end{equation}

The inhibitory nature of the dynamics is expressed in $J$ through negative off-diagonal weights. This can be observed through (\ref{Qij2}), where the derivative $M_2^{\prime}(x) < 0$, and hence $\W$ is negative. Therefore in Inhibitory we have $\s = 0$, the stability classifier follows (\ref{Sneg}) and, consequently, $S = \beta (1/2 -1 - 1 + 1/2) = -\beta$, classifying the active state of Inhibitory as asymptotically stable.

\textbf{\color{blue} Suppressed state}.\ 
In addition to the null and active states of Inhibitory, this system also exhibits a \textit{suppressed} fixed-point, in which the activities $x_i$ become bimodal:\ $\sim 50\%$ of the nodes have $x_i \to 0$, and the remaining $\sim 50\%$ have $x_i$ large, positively scaling with $d_i$. This state emerges as a consequence of the mutual inhibition between neighboring nodes, each pushing its neighbors towards lower activity. To understand this consider a highly active node $i$ with $x_i \gg 1$. This activity in (\ref{Inhibition}) suppresses the growth rate of its neighbor $j$, leading to $x_j \ll 1$. Such suppressed $x_j$ benefits $j$'s neighbors $m$, who will, consequently, also reach $x_m \gg 1$. As a result the system enters a bifurcated state, in which node $i$ is active, its neighbors are suppressed, its next neighbors are active again and so on. This state breaks our assumed symmetry, in which all neighborhoods are considered similar, and hence cannot be analyzed via our formalism. Accordingly, its associated Jacobian is not covered by the $\Ew$ ensemble, therefore beyond the scope of our current analysis.    

%%%%%%%%%%%%%%%%%%%%%%%%%%%%%%%%%%%%%%%%%%%%%%%%%%%%%%%%%%%%%%%%%%%%%%%%%%%%%%%%%%%%% 
%%%%%%%%%%%%%%%%%%%%%%%%%%%%%%%%%%%%%%%%%%%%%%%%%%%%%%%%%%%%%%%%%%%%%%%%%%%%%%%%%%%%% 
{\color{blue} \rule{12cm}{1mm}}
\vspace{2mm}  	
\section{Extended dynamics}
\label{SecExtendedDynamics}

Our anaytical framework is centered around Assumptions 1 - 6 of Sec.\ \ref{SecFramework}. To examine its applicability beyond these limits, we now examine test cases, each designed to go beyond the scope of Sec.\ \ref{SecFramework}. 

\subsection{Power dynamics - testing Assumption 2}
\label{SecPowerDynamics}

Load balance in power systems requires synchronization between all generators and consumers, often tracked through the phases $x_i(t)$ of all nodes, following \cite{Filatrella2008}

\begin{equation}
\dod[2]{x_i}{t} = 
f_i - b_i \dod{x_i}{t} + \g \sum_{j = 1}^N \m Aij \m Gij \sin \big( x_j(t) - x_i(t) \big).
\label{Power}
\end{equation} 

Here $f_i$ is a node's power generation/consumption, depending on whether it is a generator/consumer, $b_i$ is the damping coefficient, and the interaction is designed to synchronize phases $x_i$ and $x_j$. The interaction strength is mediated by the conductivity of the $i,j$ transmission line, as controlled by $\g$ and $\m Gij$. Equation (\ref{Power}) offers two generalizations to the dynamics of Eq.\ (\ref{Dynamics}) - first, by introducing the second derivative $\dif^2/\dif x^2$, and second, through its non-separable interaction mechanism, which cannot be expressed in the form $M_1(x_i)M_2(x_j)$, \textit{i.e}.\ Assumption 2. Still, as we show below, its perturbative behavior around the synchronized fixed-point continues to be characterized by a Jacobian within the family of $\Ew$.

The synchronized state has $x_i(t) = x_j(t)$ for all $i,j$, which, by shifting to the rotating frame, can be all set to zero, namely $\x^* = (0,\dots,0)^{\top}$. Under a small fixed-point perturbation $\delta \x$ we have

\begin{equation}
\dod[2]{\delta x_i}{t} = -b_i \dod{\delta x_i}{t} + 
\g \sum_{j = 1}^N \m Aij \m Gij \sin \big( \delta x_j(t) - \delta x_i(t) \big),
\end{equation}  

whose linear approximation becomes

\begin{equation}
\dod[2]{\delta x_i}{t} = -b_i \dod{\delta x_i}{t} + 
\g \sum_{j = 1}^N \m Aij \m Gij \big( \delta x_j(t) - \delta x_i(t) \big) + O(\delta x^2).
\label{PowerLinear}
\end{equation} 

Neglecting the nonlinear terms, Eq.\ (\ref{PowerLinear}) can be written as

\begin{equation}
\dod[2]{\delta x_i}{t} = -b_i \dod{\delta x_i}{t} + \m Jii \delta x_i(t) + 
\sum_{\substack{j = 1 \\ j \ne i}}^N \m Jij \delta x_j(t),
\label{PowerLinear2}
\end{equation} 

where

\begin{eqnarray}
\m Jii &=& - \g d_i
\label{JiiPower}
\\[7pt]
\m Jij &=& \m Aij \m Gij
\label{JijPower}
\end{eqnarray}

is the system's Jacobian. The resulting Jacobian is precisely in the form of $J \in \Ew$, where $C(\f,\g) = \g$ and the exponents are $\mu = 1$ and $\eta = \nu = \rho = 0$. It also, incidentally, equals to the graph Laplacian \cite{Newman2010} - recovering an already well-known connection. Under these conditions of $\Omega = (0,1,0,0)$, we have $S$ in (\ref{S}) equaling $S = \beta(1 + 0 + 0 -1 -0) = 0$, placing Power in the sensitive dynamics class. Here, even if $\lambda > 0$, sufficient damping ($b_i$) may still stabilize the system. This captures precisely the \textit{sensitivity} under $S = 0$, in which \textit{parameters} govern the value of $\lambda$. 

Note that in this system, due to the second derivative, $J$ plays a different role as compared to its role in (\ref{Dynamics}). Specifically, here $J$ governs not just stability but also the system's potential oscillations around $\x^*$. Still, our main goal is to show that even for this system, not covered by (\ref{Eq3}) we continue to observe $J \in \Ew$, further strengthening the importance and relevance of this previously unknown ensemble.

\subsection{Non-additive dynamics - testing Assumption 3}
\label{SecNonAdditiveDynamics}
 
In Assumption 3 we take the impact of $i$'s interacting partners on $i$ to be additive, as expressed via Eq.\ (\ref{Eq3})'s summation over the nonlinear $M_2(x_j)$, namely $\sum_{j = 1}^N M_2(x_j)$. To push the limits of this assumption we consider Population 2 dynamics, in which 

\begin{equation}
\dod{x_i}{t} = b_i x_i(t) \left( 1 - \dfrac{x_i(t)}{c_i} \right) + 
 x_i(t) \dfrac{\sum_{j = 1}^N \m Aij \m Gij x_j(t)}{1 + \sum_{j = 1}^N \m Aij \m Gij x_j(t)},
\label{Population2}
\end{equation}

replacing the $\sum_j M_2(x_j)$ structure of (\ref{Eq3}) by $M_2(\sum_j x_j)$, a non-additive form of interaction. Once again, despite violating our analytical assumptions, we can still analyze this system using a dedicated derivation. First, we use (\ref{M2xOdot}) together with (\ref{fXodotd}) to write

\begin{equation}
\sum_{j = 1}^N \m Aij \m Gij x_j = d_i \av x_{i,\odot} \approx d_i x_{\nn}, 
\label{Pop2NNAv}
\end{equation}

substituting the sum by the nearest neighbor average, and already implementing the fact that $f_{M,\odot}(d) \sim 1$, and hence $\av x_{i,\odot} \approx x_{\nn}$. This allows us to express the \textit{non-vanishing} fixed-point activity of a node $i$ as

\begin{equation}
1 - x_i + \dfrac{d_i x_{\nn}}{1 + d_i x_{\nn}} = 0,
\label{Pop2FixedPoint}
\end{equation}

where, for simplicity we have taken $b_i = c_i = 1$, wishing to avoid cumbersome derivations. Extracting $x_i$ from (\ref{Pop2FixedPoint}) we obtain

\begin{equation}
x_i = \dfrac{1 + 2 d_i x_{\nn}}{1 + d_i x_{\nn}} \sim d_i^0,
\label{XdPop2}
\end{equation}

namely that in the limit of large $d_i$, the fixed-point activities approach a constant and do not scale with degree.

Next, we seek the diagonal Jacobian terms $\m Jii$, writing

\begin{equation}
\m Jii = \pd{}{x_i} \left( x_i(1 - x_i) + x_i 
\dfrac{\sum_{j = 1}^N \m Aij \m Gij x_j}{1 + \sum_{j = 1}^N \m Aij \m Gij x_j} \right),
\end{equation}

which, using (\ref{Pop2NNAv}), provides us with

\begin{equation}
\m Jii = 1 - 2x_i + x_i \dfrac{d_i x_{\nn}}{1 + d_i x_{\nn}}.
\label{Pop2Jii}
\end{equation}

In (\ref{Pop2Jii}) there are no terms that contribute to the scaling with $d_i$, as indeed $x_i \sim d_i^0$ and the fraction term on the r.h.s.\ approaches unity in the limit $d_i \to \infty$. Therefore, we obtain

\begin{equation}
\m Jii \sim d_i^0,
\label{Pop2Jii2}
\end{equation} 

predicting $\mu = 0$ in $\Ew$.

For the off-diagonal terms we write

\begin{equation}
\m Jij = \pd{}{x_j} \left( x_i(1 - x_i) + x_i 
\dfrac{\sum_{m = 1}^N \m Aim \m Gim x_m}{1 + \sum_{m = 1}^N \m Aim \m Gim x_m} \right),
\end{equation}

which we break down into the form

\begin{equation}
\m Jij = \pd{}{x_j} \left( x_i(1 - x_i) + x_i 
\dfrac{\m Aij \m Gij x_j + \displaystyle \sum_{\substack{m = 1 \\ m \ne j}}^N \m Aim \m Gim x_m}
{1 + \displaystyle \sum_{m = 1}^N \m Aim \m Gim x_m} 
\right).
\end{equation}

Extracting the $x_j$ partial derivative we obtain

\begin{equation}
\m Jij = x_i \m Aij \m Gij \left(
\dfrac{1 + \displaystyle \sum_{m = 1}^N \m Aim \m Gim x_m - \m Aij \m Gij x_j -
\displaystyle \sum_{\substack{m = 1 \\ m \ne j}}^N \m Aim \m Gim x_m}
{\left( 1 + \displaystyle \sum_{m = 1}^N \m Aim \m Gim x_m \right)^2}
\right),
\end{equation}

which after collecting all terms provides

\begin{equation}
\m Jij = x_i \m Aij \m Gij 
\dfrac{1}
{\left( 1 + \displaystyle \sum_{m = 1}^N \m Aim \m Gim x_m \right)^2}.
\label{Pop2Jij1}
\end{equation}

In (\ref{Pop2Jij1}) the only term that contributes to the scaling with $d_i$ or $d_j$ is the summation in the denominator. Using (\ref{Pop2NNAv}) we can express this summation as $\sum_{m = 1}^N \m Aim \m Gim x_m = d_i x_{\nn}$, leading to

\begin{equation}
\m Jij = x_i \m Aij \m Gij 
\dfrac{1}
{\left( 1 + d_i x_{\nn} \right)^2},
\label{Pop2Jij2}
\end{equation}

which in the limit $d_i \to \infty$ provides us with

\begin{equation}
\m Jij \sim d_i^{-2},
\label{Pop2Jij}
\end{equation}

namely, an $\Ew$ Jacobian with $\nu = -2$ and $\rho = 0$. Therefore, despite not being within the form of (\ref{Eq3}) our Population 2 dynamics is also part of the broad $\Ew$ family with

\begin{equation}
\Omega = (0,0,-2,0).
\label{Pop2Omega}
\end{equation}

This represents an asymptotically stable system with $S = \beta(1 - 2 + 0 - 0 - 0) = -\beta$.

\subsection{Extinction dynamics - testing Assumption 4}
\label{SecExtinctionDynamics}

We consider population dynamics with mixed positive/negative interactions. This represents mutualistic links \textit{a l\`{a}} Population 1, alongside competitive and predatory interactions. Here, due to the adversarial links, some species populations may reach the absorbing point of $x_i = 0$, and hence a subset of the species may become extinct. The challenge is that this specific subset depends on the initial conditions, and hence the system has no unique fixed-point, having a different set of eliminated species under different initial conditions $\x(t = 0)$. 

\begin{figure}[h!]
%\begin{center}
\includegraphics[width=16cm]{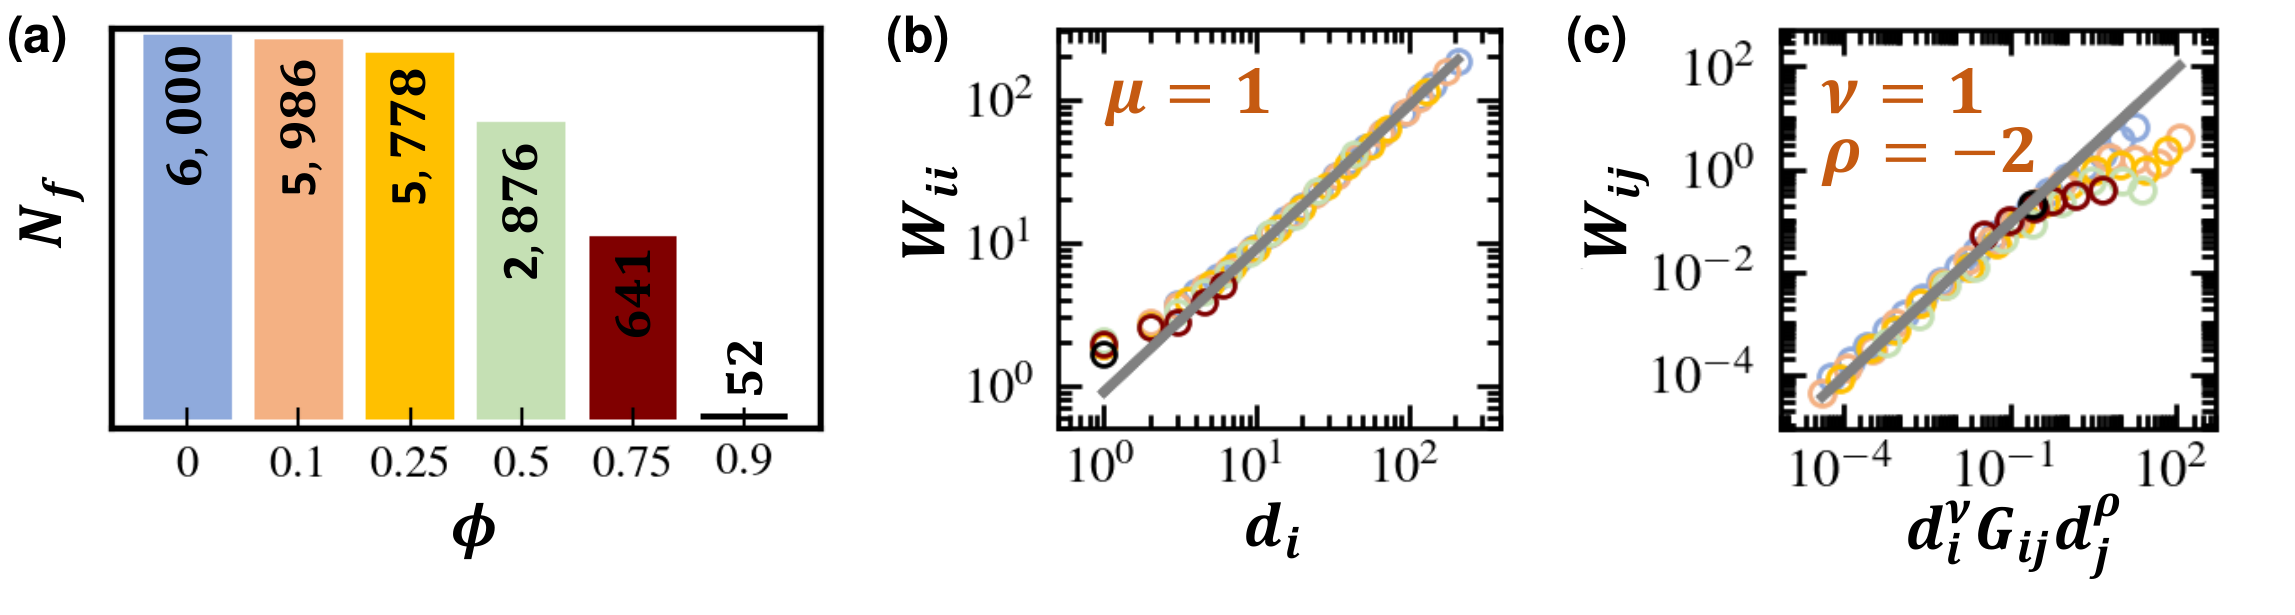}
\caption{\footnotesize \color{blue} \textbf{Emerging stability under mixed interactions}.\ 
(a) The number of surviving nodes $N_f$ vs.\ the fraction of adversarial links $\phi$. The more negative interactions the smaller the surviving node set.
(b) $\m Jii$ vs.\ $d_i$ as obtained from the $N_f$ surviving nodes.
(c) $\m Jij$ vs.\ $d_i^\nu \m Aij \m Gij d_j^\rho$ over the surviving node set. 
As long as enough nodes survive we continue to observe our predicted scaling patterns. Our prediction only breaks down under large $\phi$, where $N_f \ll N$, \textit{i.e}.\ the majority of nodes are removed.  
}
\label{FigureMixedInteractions}
\end{figure}

To test this, we constructed a scale-free $A$ with $N = 6,000$ nodes and $L = 18,000$ links, of which a fraction $0 \le \phi \le 1$ are negative ($\m Aij = -1$), and the remaining $1 - \phi$ are positive ($\m Aij = 1$). We then implemented Population 1 dynamics as appear in Eq.\ (\ref{MDynamics}), setting, for simplicity, all parameters and link weights to unity, \textit{i.e}.\ $b_i = c_i = \g = \m Gij = 1$. Starting from an arbitrary initial condition, we allowed the system to naturally reach its fixed-point. During the process, whenever a specific activity reached $x_i(t) \le \epsilon$ we set it permanently to zero (extinction), effectively removing it from the network; we used $\epsilon = 10^{-12}$. At its final state the network is reduced to $N_f \le N$ surviving nodes, upon which we examined our predicted scaling relationships. For example, under $\phi = 0.1$, starting from a randomly selected initial condition, we arrive at a final state of $N_f = 5,986$ surviving nodes, a total of $14$ extinctions (Fig.\ \ref{FigureMixedInteractions}a). Increasing $\phi$ to $25\%$ or $50\%$ the network incurs higher losses, down to $N_f = 5,778$ and $N_f = 2,876$. The crucial point is that the remaining $N_f$ nodes continue to follow the predicted scaling with $\mu = \nu = 1$ and $\rho = -2$ as obtained in Eq.\ (\ref{Pop1Omega}). 

We emphasize that the specific set of surviving nodes is different across the different realizations, and hence the system has no well-defined fixed-point. Still, despite these microscopic differences between the realizations, which depend on the detailed structure of $A$ and on the specific initial condition, the macroscopic scaling patterns remain valid, over the resulting set of surviving nodes in each realization. Of course, as we increase $\phi$, extinctions begin to dominate the final state of the system, until at a certain point, the surviving node set becomes too diluted and our predicted Jacobian structure breaks down. Our results in Fig.\ \ref{FigureMixedInteractions}b,c indicate that this breakdown occurs around $\phi = 0.75$ or $0.9$, a limit in which the majority of the nodes are lost to extinction.

%%%%%%%%%%%%%%%%%%%%%%%%%%%%%%%%%%%%%%%%%%%%%%%%%%%%%%%%%%%%%%%%%%%%%%%%%%%%%%%%%%
%%%%%%%%%%%%%%%%%%%%%%%%%%%%%%%%%%%%%%%%%%%%%%%%%%%%%%%%%%%%%%%%%%%%%%%%%%%%%%%%%%
\begin{figure}[t]
\center
\includegraphics[width=16cm]{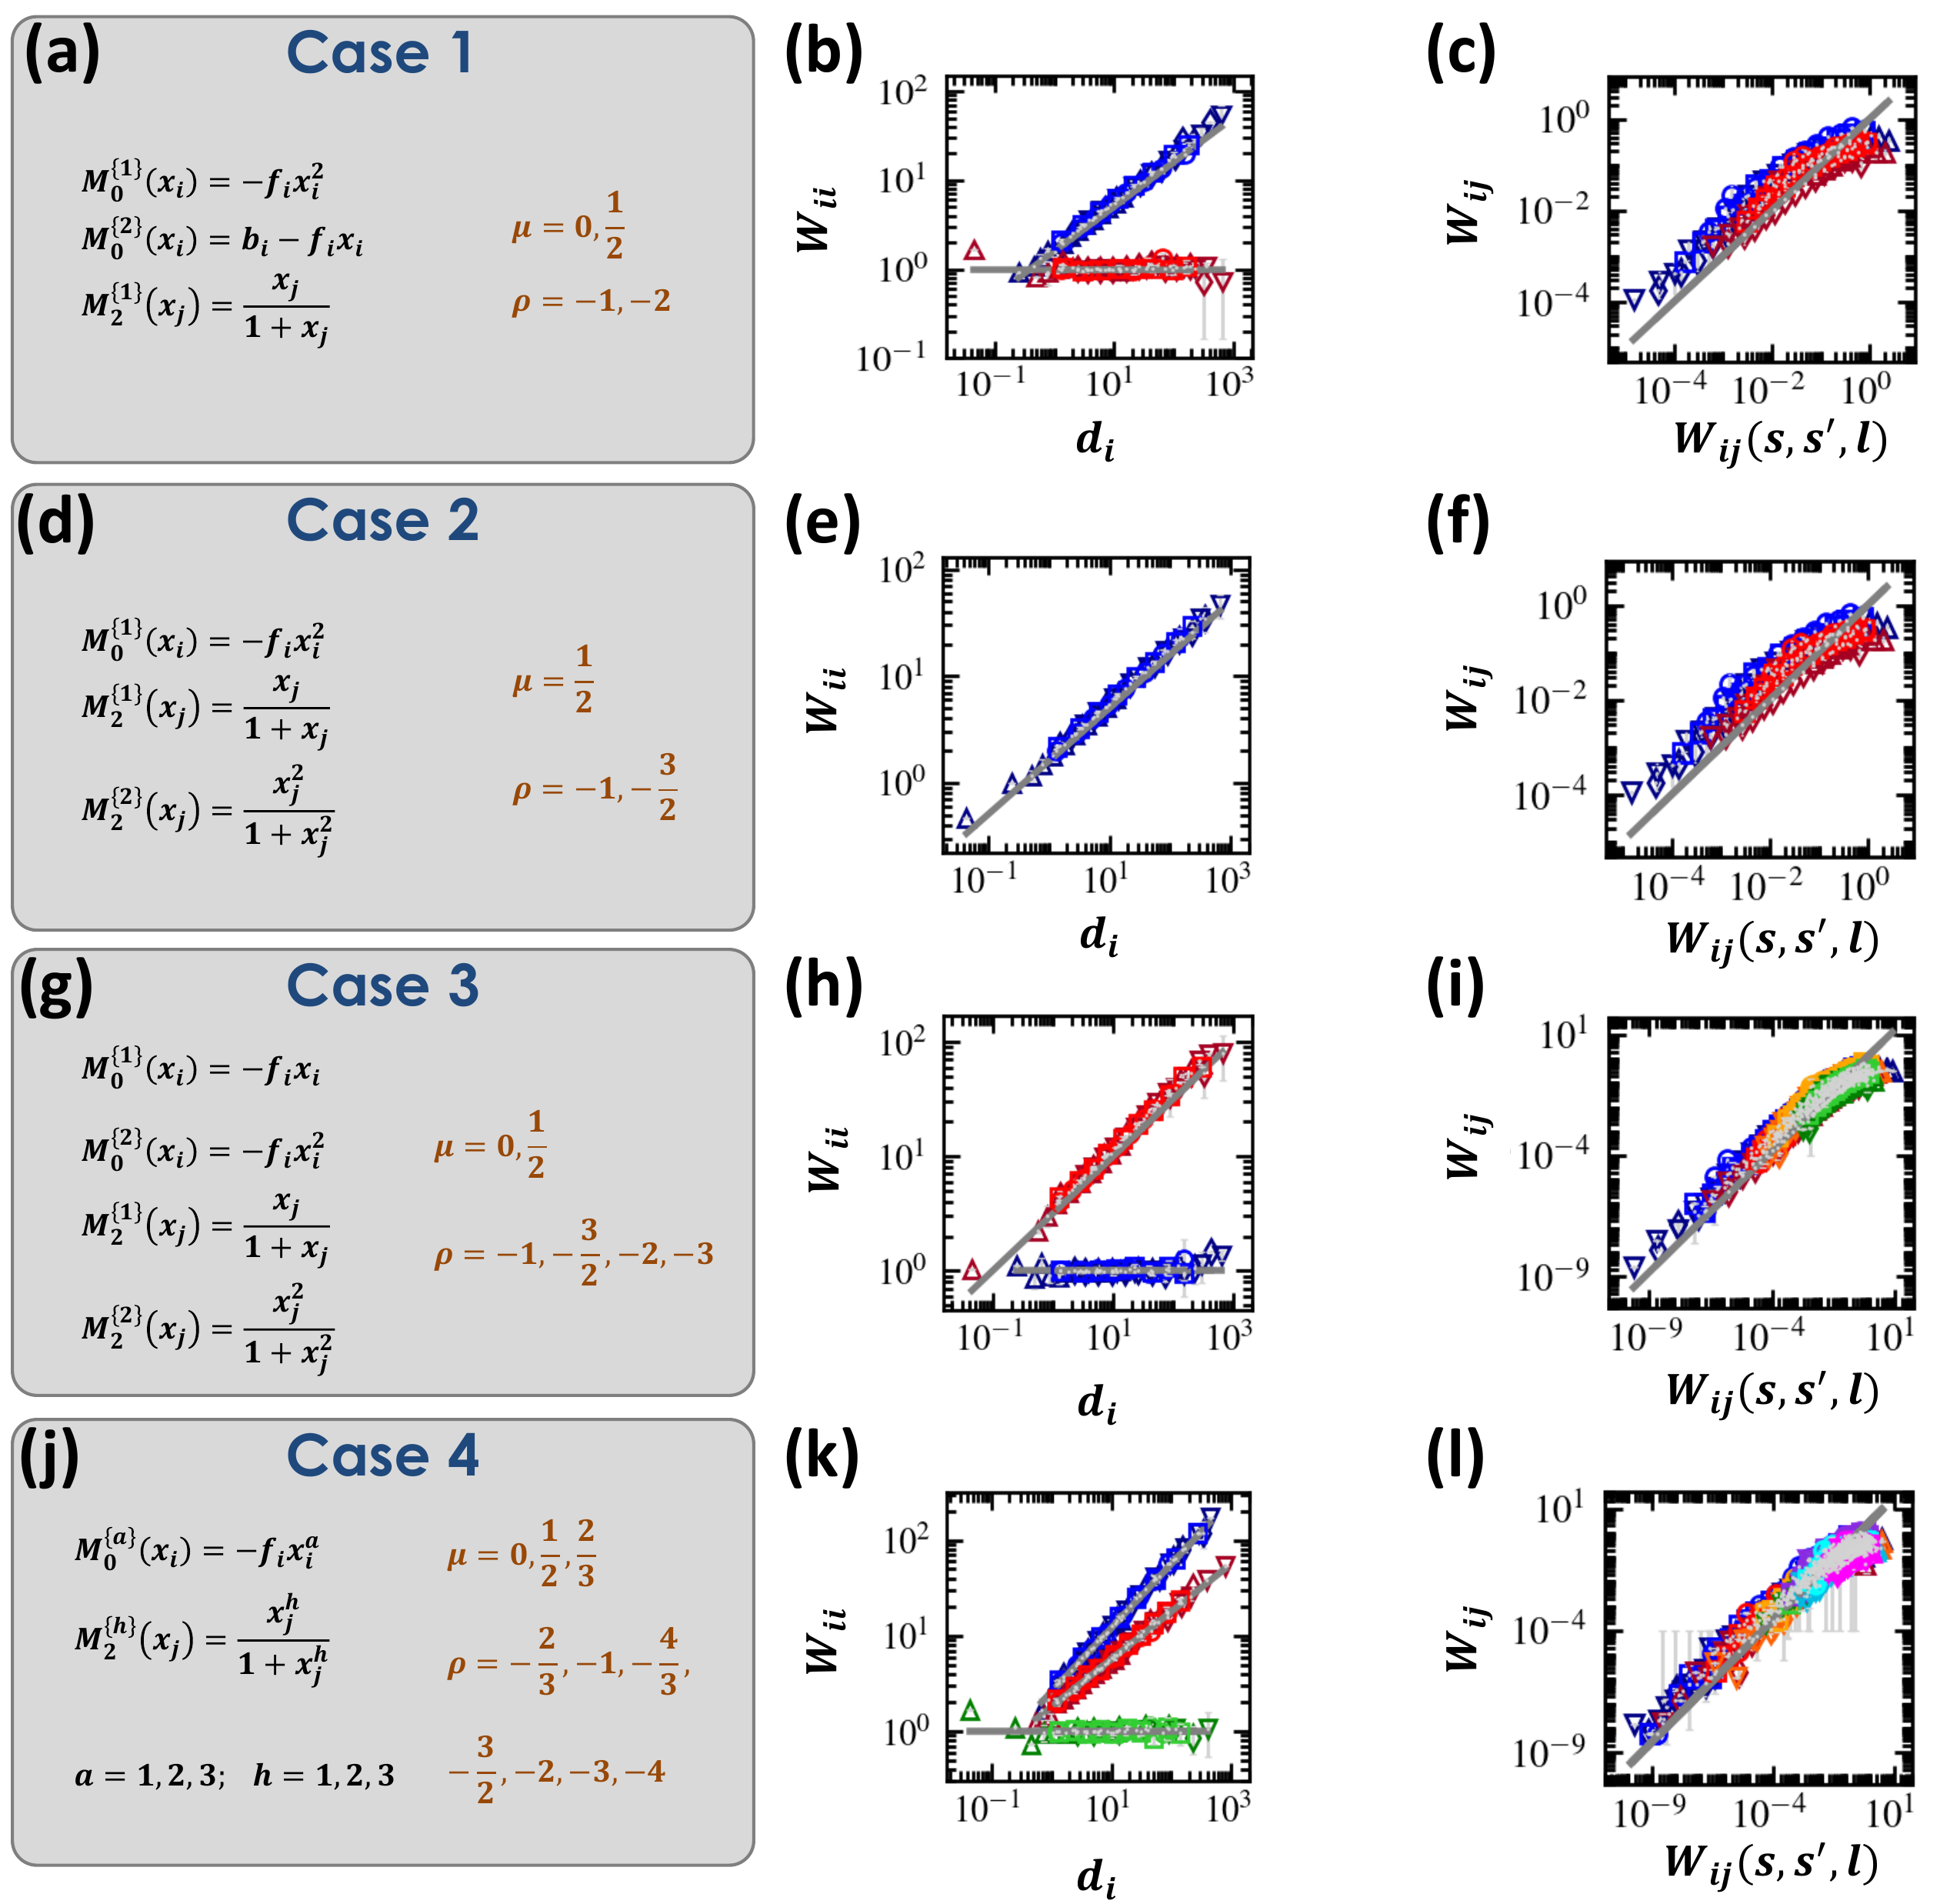}
\vspace{-8mm}
\caption{\footnotesize \color{blue} \textbf{The dynamic Jacobian ensemble under mixed dynamics}.\
We consider four examples of increasing complexity. 
(a) \textbf{Case 1}.\ Two competing self-dynamics and a single interaction dynamics distributed randomly across all nodes (left, black). The resulting coexisting values of $\mu$ and $\rho$ are listed on the right (orange).\ 
(b) The diagonal weights $\m Wii$ vs.\ degree $d_i$. Nodes belonging to $M_0^{\{1\}}(x_i)$ have $\mu(1) = 1/2$ (blue), whereas those following $M_0^{\{2\}}(x_i)$ have $\mu(2) = 0$ (red).
(c) The off-diagonal terms $\m Wij$ vs.\ the theoretically predicted $\m Wij(s,s^\prime,l)$ in Eq.\ (\ref{WijMixed}). We observe the two coexisting scaling relationships (red, blue), precisely as predicted - the red data points having $\nu(1,1) = 0, \rho(1,1) = -1$, the blue data points having $\nu(2,1) = 0, \rho(2,1) = -2$.
(d)-(f) \textbf{Case 2}.\ A similar partition into independent scaling relationships is also observed under mixed link-dynamics. 
(g)-(i) \textbf{Case 3}.\ Incorporating both mixed self and link-dynamics, we observe the diagonal $\m Wii$ split into two scaling rules, and the off-diagonal $\m Wij$ into four independently observed scaling relationships, all in accordance with predictions (\ref{WiiMixed}) and (\ref{WijMixed}).
(j)-(l) \textbf{Case 4}.\ We randomly assign three different forms of self ($a = 1,2,3$) and interaction ($h = 1,2,3$) dynamics. This system is predicted to exhibit $3$ distinct scaling relationships for $\m Wii$ (panel j, $\mu$, orange) and seven for $\m Wij$ (panel j, $\rho$, orange).
Each panel includes results from five networks (ER, SF, SF1, PPI1 and PPI2), whose nodes/links were divided into logarithmic bins $\mathbb{B}(b), b = 1,\dots,B$ (Supplementary Sec.\ \ref{LogBinning}). The number of bins ranges from $B = 10$ to $20$ for the nodes (panels b,e,h,k), and $B = 20$ to $30$ for the links (panels c,f,i,l). Therefore, the sample size within each bin is $|\mathbb{B}(b)| \in (300,600)$ for nodes and $|\mathbb{B}(b)| \in (1,200,1,800)$ for links. The error bars represent $95\%$ confidence intervals within each bin.}
\label{FigMixedDynamics}
\end{figure}
%%%%%%%%%%%%%%%%%%%%%%%%%%%%%%%%%%%%%%%%%%%%%%%%%%%%%%%%%%%%%%%%%%%%%%%%%%%%%%%%%%
%%%%%%%%%%%%%%%%%%%%%%%%%%%%%%%%%%%%%%%%%%%%%%%%%%%%%%%%%%%%%%%%%%%%%%%%%%%%%%%%%%

\subsection{Mixed-dynamics - testing Assumption 1}
\label{SecMixedDynamics}

The structure of (\ref{Eq3}) allows for diverse parameters $\f_i$, but at the same time assumes uniform dynamics, as captured via the defined set of powers $\m \Gamma qn$ in (\ref{Hahn}). The rationale is that the network components posses specific physical properties that constrain the mechanisms by which they can interact, an assumption mathematically captured by the uniformity of $\m \Gamma qn$. More realistically, however, some systems may comprise $2$ or $3$ types of nodes/links, in which case (\ref{Eq3}) may incorporate a mixture of few coexisting dynamics. To expressed this we consider the generalization

\begin{equation}
\dod{x_i}{t} = \sum_{s = 1}^S B_i^{\{ s \}} 
\left( M_0^{\{ s \}}(x_i) + \g \sum_{j = 1}^N \sum_{l = 1}^L 
M_1^{\{ s \}}(x_i) \m Aij^{\{ l \}} \m Gij M_2^{\{ l \}}(x_j) 
\right),
\label{MixedDynamics} 
\end{equation} 

capturing a coexistence of $s = 1,\dots,S$ self-dynamics and $l = 1,\dots,L$ link-dynamics. Here $B_i^{\{ s \}} = 1$ if node $i$ has self-dynamics $s$ and zero otherwise; similarly $\m Aij^{\{ l \}} = 1$ in case $i$ and $j$ interact via the $l$th link-dynamics and zero otherwise. Additionally, $\m Aij^{\{ l \}} \times \m Aij^{\{ l^\prime \}} = 0$ in case $l \ne l^\prime$, ensuring that $i$ and $j$ can interact through only a single defined mechanism. We focus on cases where the number of coexisting mechanisms is $S,L \sim 1,2,\dots$, \textit{i.e}.\ a limited discrete set of potential competing dynamics. 

While we cannot analytically extract $J$ from the generalized (\ref{MixedDynamics}), we can heuristically assume that the coexisting dynamics are manifested in $J$ through an equivalently coexisting exponent set. For example, consider the diagonal weights $\m Wii$ and their dependence on $d_i$. Instead of having all terms follow a single scaling relationship $\mu$, we now expect the nodes to partition into $S$ independent scaling functions 

\begin{equation}
\m Wii = \m Wii(s) \sim B_i^{\{ s \}} d_i^{\mu(s)}, 
\label{WiiMixed}
\end{equation}

a set of $S$ scaling functions, in which each node follows its $s$-dependent exponent $\mu(s)$. 

For the off-diagonal weights $\m Wij$, we expect such partition to be dictated by $i$'s self-dynamics $s$, $j$'s self-dynamics $s^\prime$ and the $i,j$ link dynamics $l$. Therefore $\m Wij$ will be divided into a potential of $S^2 \times L$ coexisting scaling functions, capturing the potential number of $s,s^\prime,l$ combinations. We can express this as 

\begin{equation}
\m Wij = \m Wij(s,s^\prime,l) \sim d_i^{\nu(s,l)} 
B_i^{\{ s \}} \m Aij^{\{ l \}} \m Gij B_j^{\{ s^\prime \}}
d_j^{\rho(s^\prime,l)},
\label{WijMixed}
\end{equation}

in which $\nu(s,l)$ is the exponent $\nu$ derived under self/link-dynamics $s$ and $l$, and $\rho(s^\prime,l)$ is the exponent $\rho$ matching the combination $s^\prime$ and $l$, \textit{i.e}.\ using $j$'s self-dynamics.

Together, this provides a straightforward generalization in which each of the Jacobian weights follows one of the potential $S^2 \times L$ scaling relationships with the exponent sets

\clearpage

\begin{equation}
\Omega^{ \{ s,s^\prime,l\} } = 
\Big(
\eta(s,s^\prime,l),\mu(s), \nu(s,l), \rho(s^\prime,l)
\Big).
\end{equation}

Each individual exponent is calculated via our formalism, by selecting the appropriate $M_0(x),M_1(x)$ and $M_2(x)$. We emphasize that this is a heuristic expansion of our formalism, and hence, to validate it we examine it below, numerically, for a set of four dynamic combinations of varying complexity (Fig.\  \ref{FigMixedDynamics}a,d,g,j). We also note that one may consider other potential forms of mixed-dynamics generalization, some more complex to analyze than our proposed (\ref{MixedDynamics}). However, we reserve the full analysis of mixed-dynamics for future works on the topic.  

\textbf{Case 1.\ Mixed self-dynamics} (Fig.\ \ref{FigMixedDynamics}a-c).\
We consider a system with $S = 2$ self-dynamics and a single ($L = 1$) link-dynamics. The diagonal weights $\m Wii$ have $\mu(1) = 1/2$ (blue) and $\mu(2) = 0$ (red). For $\m Wij$ we observe $\nu(1,1) = \nu(2,1) = 0$ and $\rho(1,1) = -1, \rho(2,1) = -2$. In principle, while this system has four potential scaling combinations, it reduces to just two, thanks to the shared value of $\nu$. Hence, $\m Wij(s,s^\prime,l)$ splits between a scaling $\m Wij(s,1,1) \sim d_i^0 \m Gij d_j^{-1}$ in case $j$ has self-dynamics $s^\prime = 1$ (blue) and $\m Wij(s,2,1) \sim d_i^0 \m Gij d_j^{-2}$ under $j$ in self-dynamics $s^\prime = 2$ (red); the value of $s$, denoting $i$'s self-dynamics plays no role in $\m Wij(s,s^\prime,l)$. 

\textbf{Case 2.\ Mixed interaction-dynamics} (Fig.\ \ref{FigMixedDynamics}d-f).\
Here we have $L = 2$ forms of link-dynamics, predicting a single scaling for $\m Wii$ of $\mu(1) = 1/2$, and two potential scaling rules for $\m Wij$:\ $\nu(1,1) = 0, \rho(1,1) = -1$ (red) and $\nu(1,2) = 0, \rho(1,2) = -3/2$ (blue).

\textbf{Case 3.\ Mixed self/interaction-dynamics} (Fig.\ \ref{FigMixedDynamics}g-i).\
We now incorporate a mixture of both self and link-dynamics, \textit{i.e}.\ $S = L = 2$. This leads to $\mu(1) = 0$ (blue) and $\mu(2) = 1/2$ (red); $\nu(s,l) = 0$ for all $s,l$; and $\rho(1,1) = -2$ (red), $\rho(1,2) = -3$ (blue), $\rho(2,1) = -1$ (green), $\rho(2,2) = -3/2$ (orange).  

\textbf{Case 4.\ Mixed self/interaction-dynamics} (Fig.\ \ref{FigMixedDynamics}j-l).\
To increase the challenge we consider $M_0^{\{a \}}(x_i) = -f_i x_i^a$ and $M_2^{\{h \}}(x_j) = x_j^h / (1 + x_j^h)$ for $a,h = 1,2,3$. This represents a mixture of three independently distributed self and interaction dynamics, $9$ combinations altogether. We predict three coexisting exponents $\mu(s)$ and seven (distinct) coexisting $\rho(s^\prime,l)$, all fully corroborated in Fig.\ \ref{FigMixedDynamics}k,l.

\subsection{Distributed powers - testing Assumption 1}
\label{SecDistributedPowers}

%%%%%%%%%%%%%%%%%%%%%%%%%%%%%%%%%%%%%%%%%%%%%%%%%%%%%%%%%%%%%%%%%%%%%
%%%%%%%%%%%%%%%%%%%%%%%%%%%%%%%%%%%%%%%%%%%%%%%%%%%%%%%%%%%%%%%%%%%%%
\begin{figure}[h!]
\includegraphics[width=16cm]{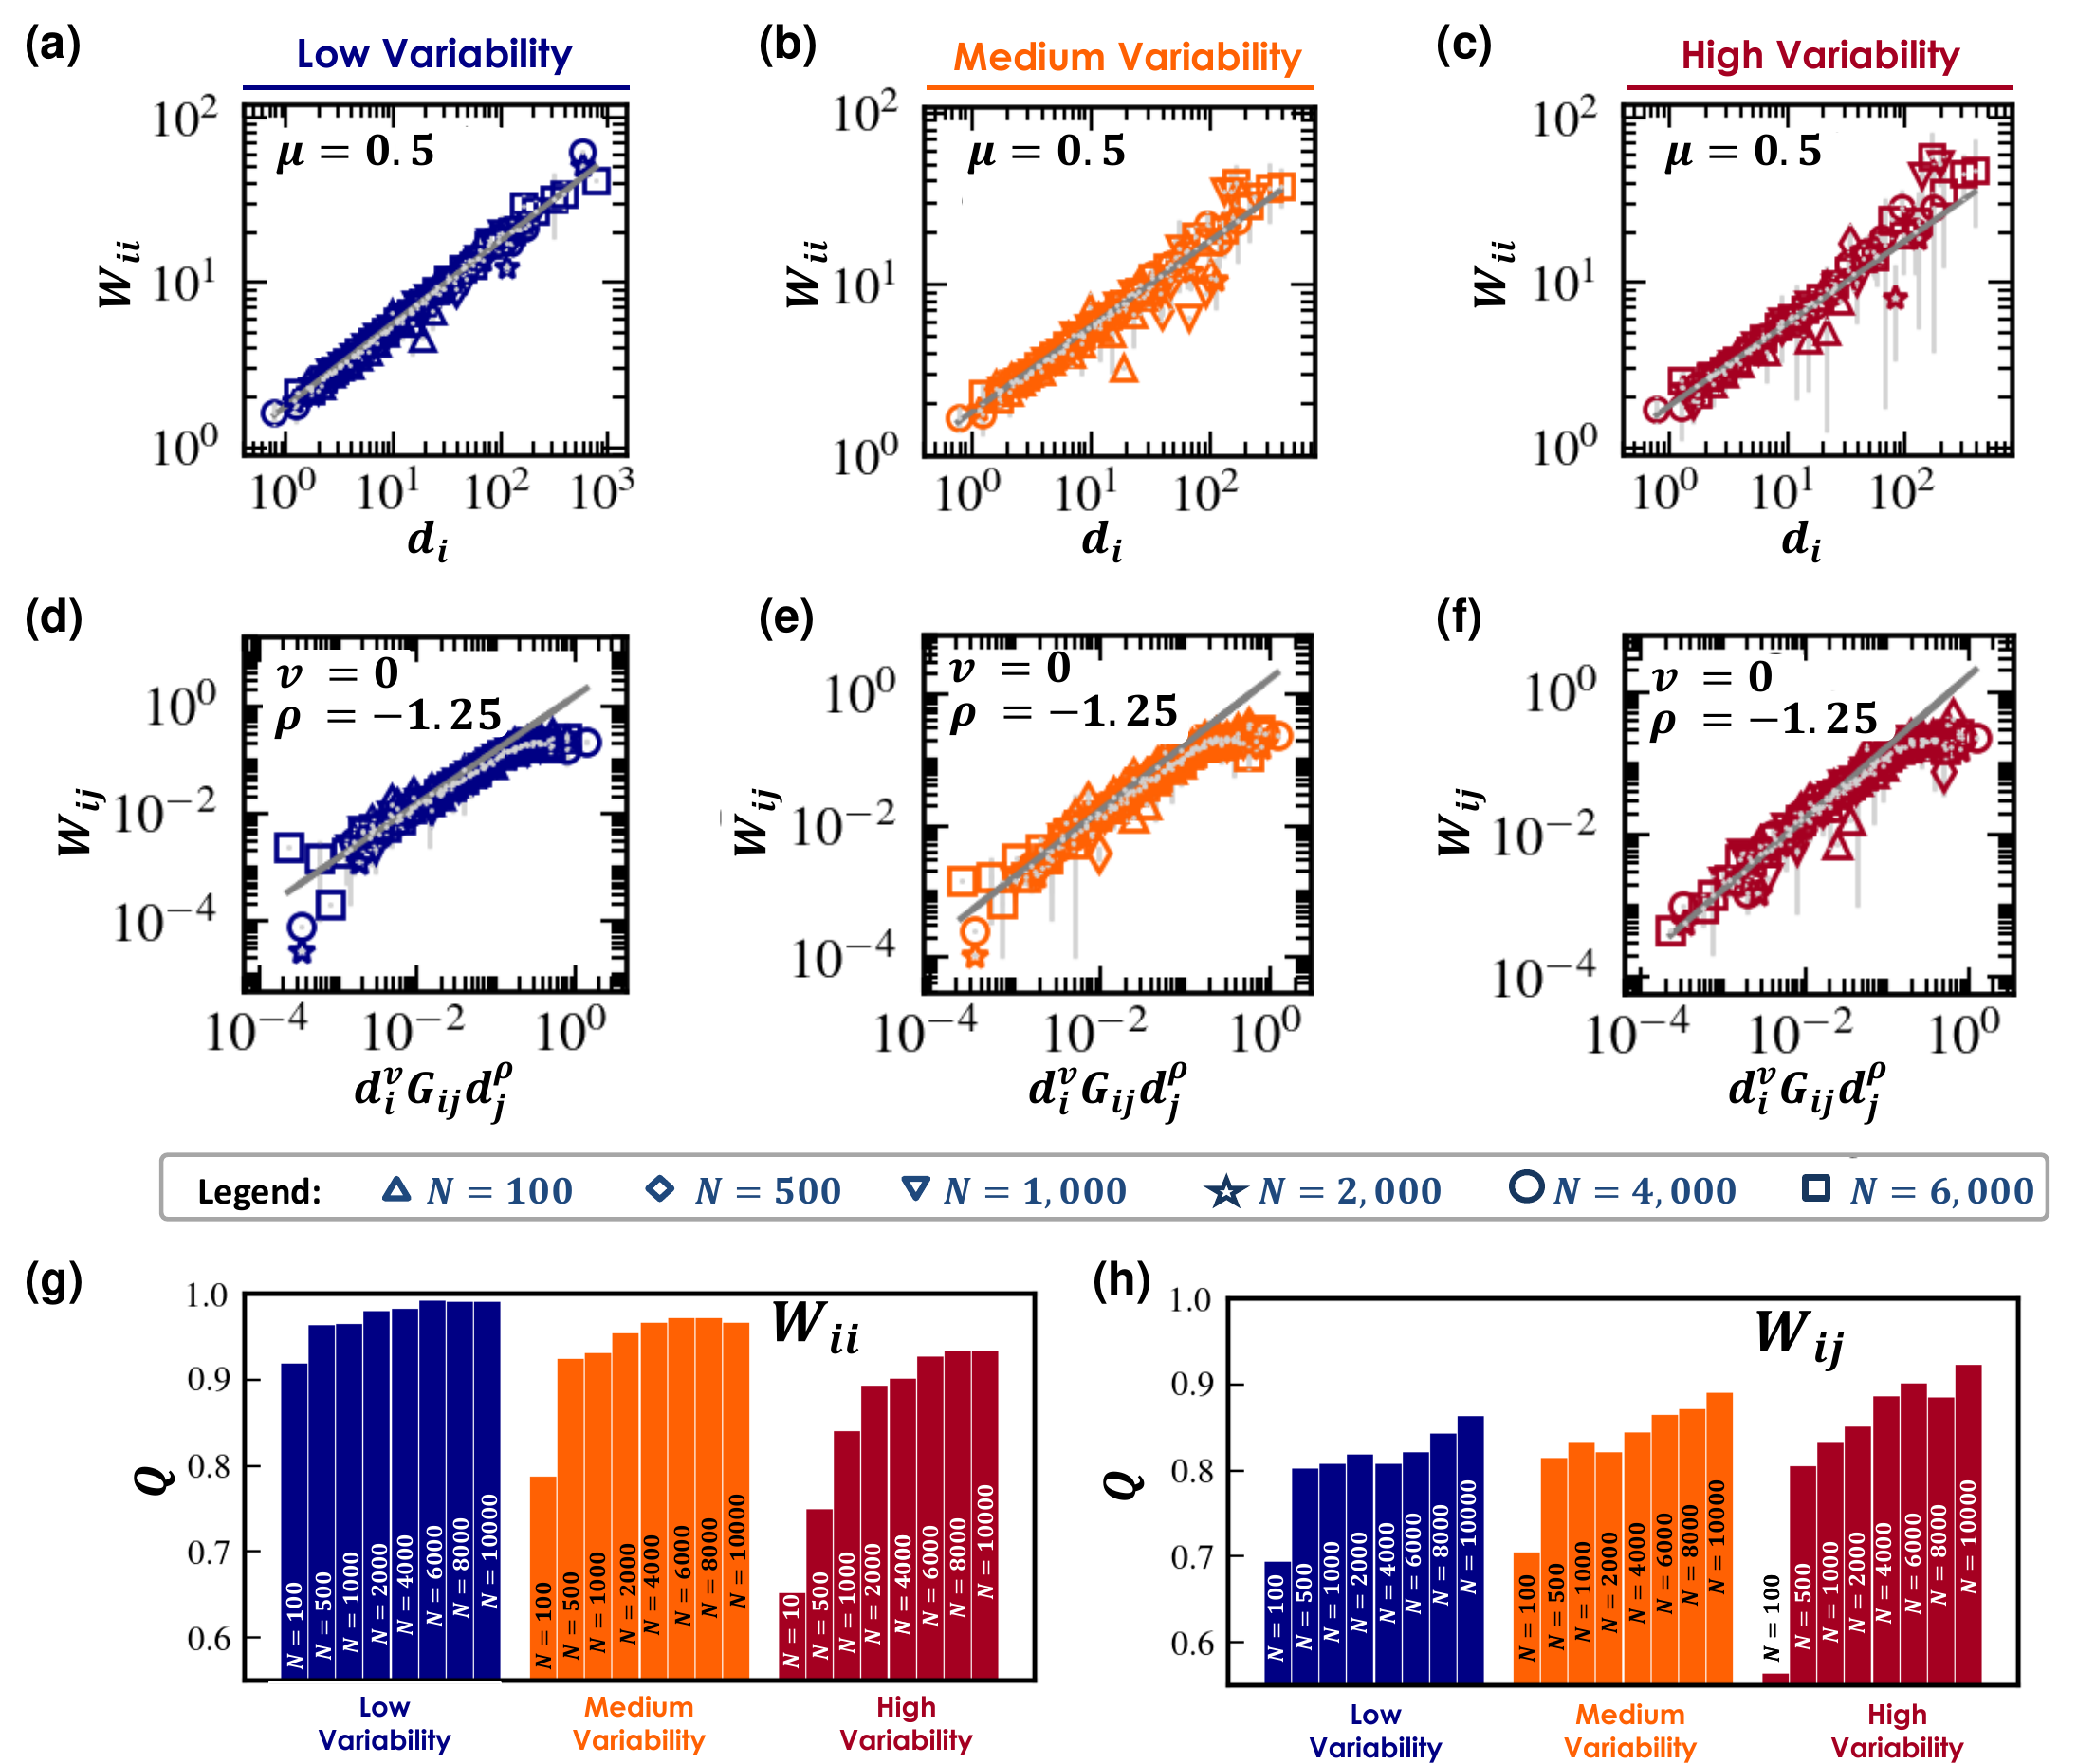}
\vspace{-5mm}
\caption{\footnotesize \color{blue} \textbf{Our Jacobian scaling patterns under distributed powers}.\
(a)-(c) The diagonal weights $\m Wii$ vs.\ $d_i$ as obtained from Regulatory dynamics on networks of size $N = 100,\dots,6,000$ (symbols) under distributed $a,h$. The data is well-approximated by our analytically predicted scaling $\mu = 0.5$ (grey), which is extracted from $\av a, \av h$. We implemented three scenarios - low (blue), medium (orange) and high (red) variability. Here the data are logarithmically binned (Sec.\ \ref{LogBinning}), and the error bars (grey) capture the noise within each bin. As expected under high variability we observe higher noise levels.
(d)-(f) Similar results for the off-diagonal weights $\m Wij$.
(g)-(h) The quality of the linear fit $Q$ for $\m Wii$ and $\m Wij$, as obtained from networks of size $N = 10^2,\dots,10^4$, under the three variability levels (low - blue;\ medium - orange;\ high - red). As the system size $N$ is increased the quality of the predicted scaling is improved, indicating that our analysis is asymptotically robust against power variability.        
Each panel includes results from networks of size $N = 100,500,1,000,2,000,4,000$ and $6,000$ nodes with $\av k = 6$. In panels a-f we divided all nodes/links into logarithmic bins $\mathbb{B}(b), b = 1,\dots,B$ (Supplementary Sec.\ \ref{LogBinning}). The number of node bins ranges from $B = 10$ for the smallest network to $B = 24$ for the largest. For the links the range is $B = 12$ to $26$. Therefore, the sample size within each bin is $|\mathbb{B}(b)| \in (50,250)$ for nodes and $|\mathbb{B}(b)| \in (250,1,400)$ for links. The error bars represent $95\%$ confidence intervals within each bin.
}
\label{FigDistributedPowers}
\end{figure}
%%%%%%%%%%%%%%%%%%%%%%%%%%%%%%%%%%%%%%%%%%%%%%%%%%%%%%%%%%%%%%%%%%%%%
%%%%%%%%%%%%%%%%%%%%%%%%%%%%%%%%%%%%%%%%%%%%%%%%%%%%%%%%%%%%%%%%%%%%%

Another potential generalization of Assumption 1 is to have the powers $\m \Gamma qn$ in the expansion (\ref{Hahn}) of $M_q(x)$ drawn from a continuous distribution. When this is the case, our analysis captures the scaling patterns extracted from the \textit{average} powers. This naturally prompts us to test its robustness against potential power-variability. To examine this we consider Regulatory dynamics of the form of Eq.\ (\ref{Regulatory}), only this time we extract the powers $a$, characterizing the nodes, and $h$, characterizing the links, from a continuous distribution. Specifically, we use $h \sim U(10^{-3},3)$, a uniform distribution ranging from $h = 10^{-3}$ to $h = 3$; we set the bottom limit just slightly above zero to ensure no link has $h = 0$, a limit in which $M_2(x)$ becomes independent of $x$. This sets the average link-dynamics at $\av h = 1.5$ with a standard deviation of $\sigma_h \approx 0.87$.

For the self-dynamic power $a$ we examine three scenarios 
$\bullet$ Low variability, where $a \sim U(1.8,2.2)$
$\bullet$ Medium variability, where $a \sim U(1.5,2.5)$
$\bullet$ High variability, where $a \sim U(1,3)$. In all three cases we have $\av a = 2$, but with a gradually increasing standard deviation $\sigma_a = 0.11,0.30$ and $0.60$ across the different settings.

Using the analysis of Sec.\ \ref{SecRegulatory} we extract the Jacobian scaling from the average powers, writing

\begin{equation}
\begin{array}{ccc}
\mu = \dfrac{\av a - 1}{\av a} = 0.5;
&
\nu = 0; 
&
\rho = -\dfrac{\av h + 1}{\av a} = -1.25.
\end{array}
\label{DistExponents}
\end{equation}

In Fig.\ \ref{FigDistributedPowers} we display the numerically obtained Jacobian weights, $\m Wii$ and $\m Wij$, finding that, indeed, they can be well approximated by our predicted scaling with the averaged exponents in (\ref{DistExponents}). Under low variability (blue) the plots are rather clean, as expected, and as we increase the variability (orange, red) we observe increasing levels of noise, expressed via the growing error bars (grey), that are designed to quantify the scaling uncertainty. 

In our analysis, we examined networks with $N = 100$ to $N = 6,000$ nodes (symbols, Fig.\ \ref{FigDistributedPowers} legend). As we increase the network size we observe a convergence to the mean. This means that the confounding effect of the $a,h$ variability is exacerbated by finite size, and as we approach the asymptotic limit $N \to \infty$, our analysis becomes robust against such variability in the powers. 

To systematically quantify this asymptotic convergence we used the mean-square-error $R^2$ to assess the deviation between the observed numerical results and our theoretically predicted scaling. To understand this, consider our scaling predictions, taking the form $Y \sim X^\alpha$. They can be expressed in log-space as linear functions, namely $y = \alpha x + \beta$ where $y = \log Y$ and $x = \log X$. Here the slope $\alpha$ captures the exponential scaling, which we \textit{predict}, and hence treat as fixed. The constant $\beta$, on the other hand, can be set arbitrarily. Upon measuring $y$ we obtain $N$ data-points $(x_i,y_i)$, $i = 1,\dots,N$, which we fit to a linear function with our fixed slope $\alpha$, then select $\beta$ to attain the best fit, \textit{i.e}.\ minimizing $R^2$. The quality of the resulting fit is then captured by $Q = 1 - R^2$, such that $Q \to 0$ represents a failed fitting and $Q \to 1$ is a perfect fit. In Fig.\ \ref{FigDistributedPowers}g,h we show $Q$ vs.\ $N$, finding that, indeed, the greater is $N$ the better is the quality of our analytical prediction in (\ref{DistExponents}). Hence, for a sufficiently large network, our results are robust against such deviations from Assumption 1, conforming to the average powers \textit{a l\`{a}} Eq.\ (\ref{DistExponents}). 

\begin{Frame}
Taken together, Secs.\ \ref{SecPowerDynamics} - \ref{SecDistributedPowers} exemplify that real-world Jacobians, under rather broad conditions, follow the scaling patterns predicted for $\Ew$. We wish to emphasize that we do not claim that this ensemble covers \textit{all} network dynamics, as indeed, these sections provide just a few anecdotal examples beyond the coverage of our original Eq.\ (\ref{Eq3}) under Assumptions 1-6. Still, these examples do indicate the potential merit in further studying this Jacobian ensemble and its relevance to a potentially vast range of real-world dynamic applications.
\end{Frame}
\vspace{-3mm}

%%%%%%%%%%%%%%%%%%%%%%%%%%%%%%%%%%%%%%%%%%%%%%%%%%%%%%%%%%%%%%%%%%%%%%%%%%%%%%%%%%%%% 
%%%%%%%%%%%%%%%%%%%%%%%%%%%%%%%%%%%%%%%%%%%%%%%%%%%%%%%%%%%%%%%%%%%%%%%%%%%%%%%%%%%%% 
{\color{blue} \rule{12cm}{1mm}}
\vspace{2mm}  	
\section{Local vs.\ global stability}
\label{SecLocalStability}
 
Our asymptotically stable class ($S < 0$) represents a robust stability, that remains unaffected by microscopic discrepancies, such as parameter or topological perturbations. But what if we explicitly form an unstable motif and introduce it \textit{brute force} into the network. Can such a local intervention destabilize the system? Here, we demonstrate that an asymptotically stable system remains insensitive to such local instabilities, whose impact on the network becomes negligible as $N \to \infty$.

%%%%%%%%%%%%%%%%%%%%%%%%%%%%%%%%%%%%%%%%%%%%%%%%%%%%%%%%%%%%%%%%%%%%%%%%%%%%%%%%%%%%% 
%%%%%%%%%%%%%%%%%%%%%%%%%%%%%%%%%%%%%%%%%%%%%%%%%%%%%%%%%%%%%%%%%%%%%%%%%%%%%%%%%%%%% 
\begin{figure}[h!]
\includegraphics[width=16cm]{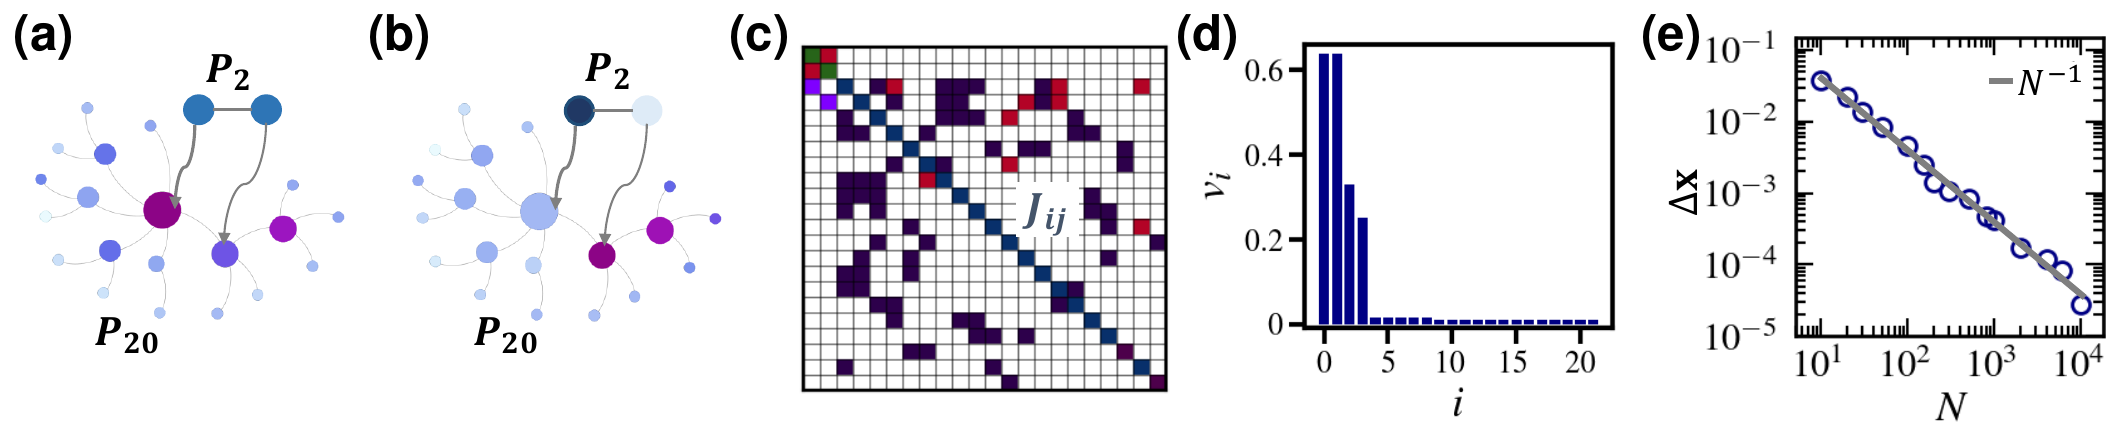}
\vspace{-5mm}
\caption{\footnotesize \color{blue} \textbf{Local vs.\ global instability}.\
(a) The system $P_N$ (here $N = 20$), an asymptotically stable network of $N$ nodes is coupled with $P_2$ of Eq.\ (\ref{MotifDynamics}), an exclusion motif, set at the unstable coexisting state $y_1 = y_2 > 0$. The global state of the two systems together is denoted by $\x_0$.
(b) Following perturbation $P_2$ transitions to the exclusion state, thus affecting its neighboring nodes in $P_N$. The system settles at the new state $\x_1$. Therefore, in principle, $\x_0$ is unstable. This indicates that a microscopic intervention, here coupling $P_2 \to P_N$, can destabilize an otherwise asymptotically unstable system.
(c) The Jacobian $J$, as obtained from the coupled $P_2 \to P_N$ system. The nodes in $P_2$ are represented by the entries at the top-left corner (red, green), and their immediate neighborhood directly below (purple).
(d) The principal eigenvector entries $v_i$ are highly localized around $P_2$ ($i = 1,2$) and its immediate neighborhood ($i = 3,4,5$). Therefore, the instability of $\x_0$ is strictly localized and has no discernible effect on the majority of the nodes.
(e) The global response $\Delta \x$ vs.\ the size of $P_N$ (circles). Indeed, $\Delta \x \to 0$, scaling with $N^{-1}$ (grey solid line). This asserts $P_N$'s asymptotic stability. 
}
\label{FigLocalInstability}
\end{figure} 
%%%%%%%%%%%%%%%%%%%%%%%%%%%%%%%%%%%%%%%%%%%%%%%%%%%%%%%%%%%%%%%%%%%%%%%%%%%%%%%%%%%%% 
%%%%%%%%%%%%%%%%%%%%%%%%%%%%%%%%%%%%%%%%%%%%%%%%%%%%%%%%%%%%%%%%%%%%%%%%%%%%%%%%%%%%% 

To examine this we implemented Population 1 dynamics, as in (\ref{MDynamics}), on a scale-free network of size $N$. We denote this system by $P_N$. We also constructed a two node exclusion motif $P_2$, whose dynamics is given by

\begin{eqnarray}
\dod {y_1}{t} &=& y_1(1- y_1) - g y_1 y_2
\nonumber 
\\[4pt] 
\dod {y_2}{t} &=& y_2(1- y_2) - g y_1 y_2.
\label{MotifDynamics}
\end{eqnarray}
 
The motif $P_2$ exhibits three fixed-points:\ two stable \textit{exclusion} states, in which only one of the species survives, \textit{i.e}.\ $y_1 > 0$ \textit{or} $y_2 > 0$, and a single unstable \textit{coexisting} state, in which both $y_1 = y_2 > 0$. We now directionally couple $P_2 \to P_N$, by adding the terms $\dots + C y_1$ and $\dots + C y_2$ to the equations of two randomly selected nodes in $P_N$. Under such coupling the activities $y_1,y_2$ of $P_2$ affect the state of $P_N$, but not vice versa, as no coupling exists in the opposite direction. Hence, $P_2$'s fixed-points remain unaffected by this coupling.

We next set $P_2$ at its unstable coexisting state and allow the coupled system $P_2 \to P_N$ to reach its global fixed-point $\x_0$. This state $\x_0$, the fixed-point of the $N + 2$ nodes of $P_N$ and $P_2$ combined is, by definition, unstable. Indeed, even the slightest perturbation to $y_1$ or $y_2$ will drive $P_2$ into its exclusion state. Then, through the coupling $C$ this change in state of $P_2$ will spillover to affect the activities of the nodes in $P_N$, driving them towards a new state $\x_1$. Consequently, while the original $P_N$ had an asymptotically stable $\x_0$ state, the coupling with $P_2$, a microscopic perturbation, caused it to no longer be stable. To demonstrate this, we extracted $J$ from the complete $N + 2$ node system, and, as expected, found that the principal eigenvalue $\lambda$ is, indeed, positive (Fig.\ \ref{FigLocalInstability}c).

The crucial point is that $\x_0$'s instability remains strictly local. To observe this we examine the principal eigenvector $\v$, associated with $\lambda$. In Fig.\ \ref{FigLocalInstability}d we observe that $\v$ is highly localized, with most its mass condensed on $P_2$, and a small fraction on the nearby nodes of $P_N$, directly neighboring $P_2$. Therefore, while $\x_0$ is, indeed, unstable, the final state $\x_1$ reached by the system is, for the most part, identical to $\x_0$, barring a localized discrepancy on $P_2$ and its immediate vicinity. For a sufficiently large system, such local instability, becomes asymptotically negligible.

To observe this we measure the global response 

\begin{equation}
\Delta \x = \dfrac{1}{N} \sum_{j = 1}^N \big| \m x1j - \m x0j \big|,
\label{DxLocal}
\end{equation}

capturing the average long-term shift in the state of all nodes, as a result of the perturbation to $\x_0$. Obtaining $\Delta \x$ from networks $P_N$ of different size, ranging from $N = 10$ to $N = 10^4$ we observe that $\Delta \x \sim N^{-1}$, approaching $\Delta \x \to 0$ in the limit $N \to \infty$. Under these conditions $\x_0$, our initial \textit{unstable} state, is asymptotically identical to $\x_1$, the system's perturbed state. Therefore, if $\x_0 \to \x_1$, we can say that $x_0$ it \textit{is} stable, as it is robust against perturbation. This captures precisely the local nature of the instability, as it remains confined to a bounded neighborhood around $P_2$, and hence, when averaged over the entire system vanishes as $1/N$. More broadly, it demonstrates the notion of asymptotic stability, that under $N \to \infty$ the system becomes insensitive to perturbation, here withstanding the forced coupling with the unstable motif $P_2$.

%%%%%%%%%%%%%%%%%%%%%%%%%%%%%%%%%%%%%%%%%%%%%%%%%%%%%%%%%%%%%%%%%%%%%%%%%%%%%%%%%%%%% 
%%%%%%%%%%%%%%%%%%%%%%%%%%%%%%%%%%%%%%%%%%%%%%%%%%%%%%%%%%%%%%%%%%%%%%%%%%%%%%%%%%%%% 
{\color{blue} \rule{12cm}{1mm}}
\vspace{2mm}  	
\section{Methods and data analysis}
\label{Supplementary Information 3: Methods and Data Analysis}

\subsection{Numerical integration}
\label{numerical_inte}

To numerically test our predictions we constructed Eq.\ (\ref{Eq3}) for each of the systems in Sec.\ \ref{Models}, using the appropriate network $A,G$ (Scale-free, Erd\H{o}s-R\'{e}nyi, empirical, etc.). We then used a fourth-order Runge-Kutta stepper (Matlab's ode45) to numerically solve the resulting equations. Starting from an arbitrary initial condition $x_i(t = 0)$, $i = 1,\dots,N$, we allowed the system to reach steady-state by waiting for $\dot x_i \rightarrow 0$. To numerically realize this limit we implemented the termination condition 

\begin{equation}
\max_{i = 1}^N \left| \frac{x_i(t_n) - x_i(t_{n - 1})}{x_i(t_n) \Delta t_n}\right| < \varepsilon,
\label{TerminationCondition}
\end{equation}
    
\noindent
where $t_n$ is the time stamp of the $n$th Runge-Kutta step and $\Delta t_n = t_n - t_{n - 1}$. As the system approaches a steady-state, the activities $x_i(t_n)$ become almost independent of time, and the numerical derivative $\dot x_i = (x_i(t_n) - x_i(t_{n - 1})) / \Delta t_n$ becomes small compared to $x_i(t_n)$. The condition (\ref{TerminationCondition}) guarantees that the maximum of $\dot x_i/x_i$ over all activities $x_i(t_n)$ is smaller than the pre-defined termination variable $\varepsilon$. In our simulations, across the different dynamics we tested, we set $\varepsilon \le 10^{-12}$, a rather strict condition, to ensure that our system is sufficiently close to the {\it true} steady-state.

\subsubsection{Numerical analysis of Power dynamics}

To analyze Power dynamics we used the Newton-Raphson method to extract the roots of 
	
\begin{equation}
0 = f_i + \g \sum_{j = 1}^N \m Aij \m Gij \sin \big( x_j(t) - x_i(t) \big),
\label{PowerFixedPoint}
\end{equation} 
	
providing the fixed-point of (\ref{Power}), under $\ddot{x}_i = \dot{x}_i = 0$. For a system with $n_{\rm gen}$ generators and $n_{\rm load}$ loads, we set $f_i = -1$ for load nodes and $f_i = n_{\rm load}/n_{\rm gen}$ for generators. This ensures a global balance of power generation vs.\ demand. The global weight was set to $\g = 1$, and the link weights were also set uniformly to $\m Gij = 1$, \textit{i.e}.\ a binary network. In our empirical power-networks (Sec.\ \ref{Networks}) the number of loads $n_{\rm load}$ vs.\ generators $n_{\rm gen}$ is specified in the data. For the model networks we used a balanced network with $50\%$ generators and $50\%$ loads, assigned at random. As our initial condition we extracted $x_i$ from a uniform distribution, seeking a starting point from which the system converges to a fully positive solution. This was satisfied for $x_i \sim U(0.8,1.5)$ for the model networks and for $x_i \sim U(3.5,4.5)$ for the empirical ones. Using the obtained roots $\x = (x_1,\dots,x_N)^{\top}$ we constructed the relevant Jacobian matrix as explained below in Sec.\ \ref{SecNumericalJij}.
	
\subsection{Numerically estimating $J$}
\label{SecNumericalJij}

Once the steady state $\mathbf{x} = (x_1, \dots, x_N)^{\top}$ is reached we construct the \textit{numerical} Jacobian by substituting the numerically obtained states $x_i$ into (\ref{Dii}) and (\ref{Qij2}). This represents the system's \textit{actual} stability matrix, as obtained for each dynamics on its relevant networks. For example, consider our Epidemic model in Eq.\ (\ref{SISDynamics}), where $M_0(x) = -f_i x_i, M_1(x_i) = 1 - x_i$ and $M_2(x) = x_j$, and hence $M_0^{\prime}(x) = -f_i, M_1^{\prime} = -1$ and $M_2^{\prime} = 1$. Once we obtain $\mathbf{x}$ we introduce all numerically calculated $x_i$ into $\m Wii$ and $\m Wij$, which for Epidemic take the form

\begin{equation}
\m Wii = - f - \g \sum_{j = 1}^N \m Aij \m Gij x_j
\label{SISDii}
\end{equation}

and

\begin{equation}
\m Wij = \g \m Aij \m Gij (1 - x_i).
\label{SISQij}
\end{equation}
    
This construction, directly from the numerically obtained fixed-point $\x^*$ is \textit{exact}, incorporating all the potential confounding factors of the specific system, from the fine-structure and potential degree-correlations in $A$, to the random distribution of $\m \f qi$ and $\m Gij$, or the varying interaction strength $\g$. In Fig.\ 3 of the main text we compare the scaling of these numerically estimated $\m Wii$ and $\m Wij$ vs.\ the theoretically predicted ensemble $\Ew$, as provided by (\ref{JiiFrame}) and (\ref{JijFrame}).    
    
\subsection{Logarithmic binning}
\label{LogBinning}

Our main theoretical prediction focuses on scaling relationships, such as $W(d) \sim d^{\mu}$, which we observe by their linear slope in a log-log plot (\textit{e.g}., Fig.\ 3 of main text). To construct such plots we employed logarithmic binning \cite{Milojevic2010}. First we divide all nodes into $B$ bins
      
\begin{equation}
\mathbb{B}(b) = \left\{ i \in \{1,\dots,N\} 
\left| c^{b-1} < \dfrac{d_i}{d_{\rm min}} \le c^b \right. 
\right\},
\label{wbinning}
\end{equation}

where $b = 1,...,B$, $c$ is a constant and $d_{\rm min} = \min_{i = 1}^N d_i$ is the minimal weighted degree in $A \otimes G$. In (\ref{wbinning}) the $b$th bin includes all nodes $i$ whose weighted degree $d_i$ is between $d_{\rm min}c^{b-1}$ and $d_{\rm min}c^{b}$. The parameter $c$ is selected such that the unity of all bins $\cup_{b = 1}^B \mathbb{B}(b)$ includes all nodes, hence we set $c^{B} = d_{\rm max}/d_{\rm min}$. Therefore, the first bin $b = 1$ is bounded from below by $d_{\rm min}$, and the final bin bounded from above by $d_{\rm max}$. Dividing the nodes according to (\ref{wbinning}) generates exponentially growing bins in $d_i$, which are \textit{linear} in $\log d_i$, allowing to naturally observe the scaling in the logarithmic plots. 

After dividing all nodes into bins, we plot the average degree of the nodes in each bin 

\begin{equation} 
d_b = \langle d_i \rangle_{i \in \mathbb{B}(b)} = 
\dfrac{1}{|\mathbb{B}(b)|}\sum_{i \in \mathbb{B}(b)} d_i
\label{kBinning}
\end{equation}

\noindent
versus the average $W(d)$ term of nodes in that bin

\begin{equation}    
W(d_b) = \langle \m Wii \rangle _{i \in \mathbb{B}(b)} = 
\dfrac{1}{|\mathbb{B}(b)|}\sum_{i \in \mathbb{B}(b)} \m Wii.
\label{DBinning}
\end{equation}

In a similar fashion we plot $\m Wij \sim d_i^{\nu} \m Gij d_j^{\rho}$, this time applying the binning to $W_{ij}^{\rm Theory} = d_i^{\nu} \m Gij d_j^{\rho}$, instead of to $d_i$. Therefore, the bins are defined as 

\begin{equation}
\mathbb{B}(b) = 
\left\{ (i,j) \big{|} \m Aij = 1, c^{b-1} < \dfrac{W_{ij}^{\rm Theory}}{W_{\rm min}} \le c^b \right\},
\label{wbinning2}
\end{equation}

such that in each bin we include all node pairs whose product $d_i^{\nu} \m Gij d_j^{\rho}$ is within a given range. Similarly to (\ref{wbinning}) we set $W_{\rm min} = \min (W_{ij}^{\rm Theory})$, and select $c$ such that the entire range of $W_{ij}^{\rm Theory}$ is covered. As above, we then plot the average \textit{real} $\m Wij$ in each bin vs.\ the theoretically predicted $W_{ij}^{\rm Theory}$. Specifically, these averages take the form

\begin{eqnarray}    
W^{\rm Real}(b) &=& \langle \m Wij \rangle _{(i,j) \in \mathbb{B}(b)} = 
\dfrac{1}{|\mathbb{B}(b)|}\sum_{(i,j) \in \mathbb{B}(b)} \m Wij
\label{QBinning1}
\\[5pt]
W^{\rm Theory}(b) &=& \langle d_i^{\nu} \m Gij d_j^{\rho} \rangle _{(i,j) \in \mathbb{B}(b)} = 
\dfrac{1}{|\mathbb{B}(b)|}\sum_{(i,j) \in \mathbb{B}(b)} W_{ij}^{\rm Theory},
\label{QBinning2}
\end{eqnarray}

where $\m Wij$ in (\ref{QBinning1}) is constructed via Sec.\ \ref{SecNumericalJij}.

\subsection{Model and empirical networks}
\label{Networks}

\begin{table}[t!]
\includegraphics[width=16cm]{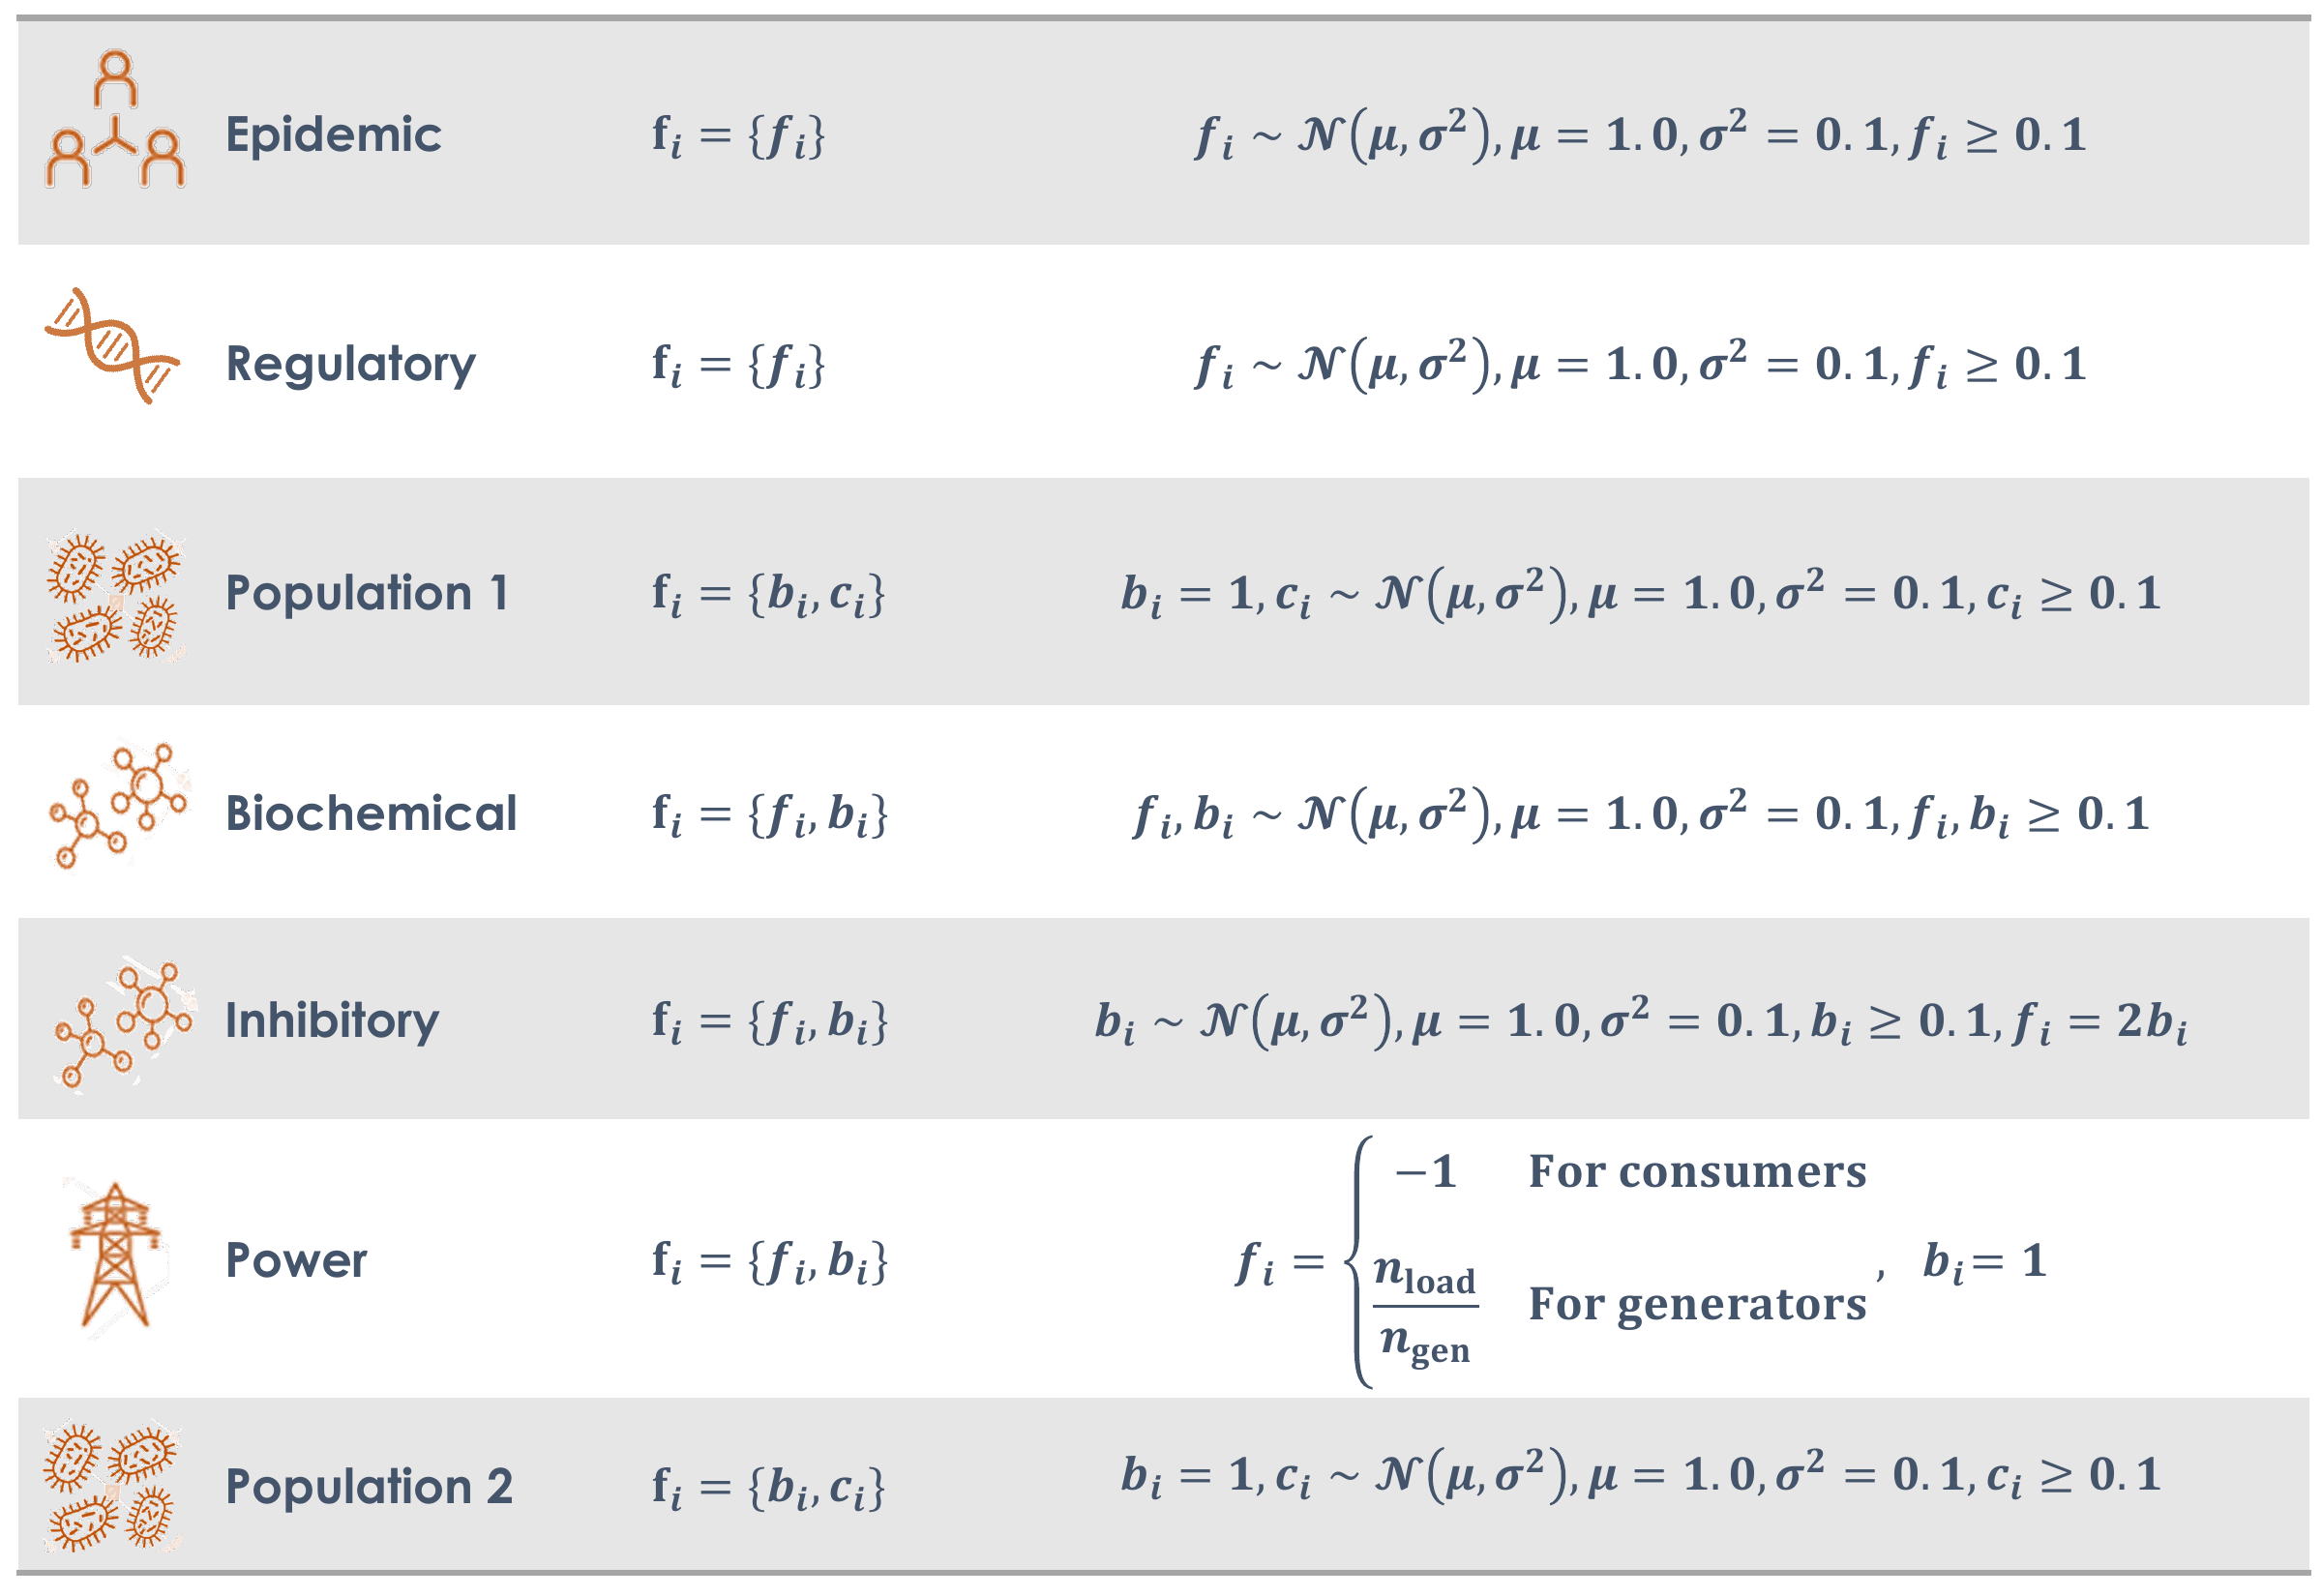}
\caption{\footnotesize \color{blue} \textbf{Model parameters}.
For each of our dynamic models we summarize the dynamic parameters used in our simulations. For example, in Epidemic the recovery rate was extracted from a truncated normal distribution with mean $\mu = 1.0$ and variance $\sigma^2 = 0.1$. To avoid the irrelevant scenraio of a negative recovery rate we truncated this distribution at $f_i \ge 0.1$. Biochemical, Inhibitory and Power have two parameters $\f_i = (f_i,b_i)$. In Inhibitory the Alee effect required $f_i > b_i$ for all species. To ensure this we extracted $b_i$ from a truncated normal distribution, then set $f_i = 2b_i$. In Power the loads were set to $-1$ for consumer nodes, then the generation was gauged to ensure a balanced network.} 
\label{ParametersTable}
\end{table}

To test our predictions we used model and empirical networks, as summarized below:

\noindent {\bf ER}.\ 
An Erd\H{o}s-R\'{e}nyi random network with $N = 6,000$ nodes and an average degree of $\langle k \rangle = 6$. Weights were added using $\m Gij \sim \N(1.0,0.1)$, a normal distribution function with mean $\mu=1.0$ and variance $\sigma^2 = 0.1$. Note that this weight distribution allows for a small number of negative weights, hence, in practice, it test out predictions under a coexistence of a majority positive along side a small minority of negative links. 
	
\noindent {\bf SF}.\ 
A binary scale-free network with $N = 6,000$ nodes, average degree $\langle k \rangle = 6$, and degree distribution following $P(k) \sim k^{-\gamma}$ with  $\gamma = 2.5$. Under this distribution we have $\knn \sim N^\beta$ with $\beta = 0.6$, allowing us to examine our asymptotic limits (which require $\beta > 0$).
	
\noindent {\bf SF1}.\ 
Using the underlying topology of SF we added weights $ \m Gij$, extracted from a normal distribution with mean $\mu=1.0$ and variance $\sigma^2 = 0.1$, \textit{i.e}.\ $\m Gij \sim \N(1.0, 0.1)$. Also here we did not limit the weights from becoming negative.
	
\noindent {\bf SF2}.\ 
Using the underlying topology of SF we added weights $\m Gij$, from a scale-free probability density function $P(G) \sim G^{-\alpha}$ with $\alpha = 3$. Hence, SF2 represents an extremely heterogeneous network, featuring both scale-free topology and scale-free weights.
	 
\noindent {\bf UCIonline}.\ 
An instant messaging network from the University of California Irvine \cite{Opsahl2009}, capturing $61,040$ transactions between $1,893$ users during a $T = 218$ day period. Connecting all individuals who exchanged messages throughout the period, we obtain a network of $1,893$ nodes with $27,670$ links, exhibiting a fat-tailed degree distribution. Here weights $\m Gij$ are taken from a scale-free probability density function $P(G) \sim G^{-\alpha}$ with $\alpha = 3$, once again examining conditions of extreme heterogeneity.
	 
\noindent {\bf Email Epoch}.\ 
This dataset monitors $\sim 3 \times 10^5$ emails exchanged between $3,185$ individuals over the course of $\sim 6$ months \cite{Eckmann2004}, giving rise to a scale-free social network with $31,885$ binary links.
Here too weights $\m Gij$ were extracted from a scale-free probability density function $P(G) \sim G^{-\alpha}$ with $\alpha = 3$.

\noindent {\bf PPI1}.\
The yeast scale-free protein-protein interaction network, consisting of $1,647$ nodes (proteins) and $5,036$ undirected links, representing chemical interactions between proteins \cite{Yu2008}. Weights were assigned via $\m Gij \sim \N(1.0, 0.1)$.
	 
\noindent {\bf PPI2}.\ 
The human protein-protein interaction network, a scale-free network, consisting of $N = 2,035$ nodes (proteins) and $L = 13,806$ protein-protein interaction links \cite{Rual2005}. Here too, weights were assigned via $\m Gij \sim \N(1.0, 0.1)$.
	
\noindent {\bf Microbial 1}.\
To construct microbial networks we collected data on $844$ microbial species and $283$ associated metabolites \cite{lim2020large}. This allowed us to construct an $844 \times 283$ directed bipartite network $B$ whose links capture the production and consumption of metabolites among the microbial species:\ $\m Bim = 1$ if species $i$ \textit{produces} metabolite $m$; $\m Bmi = 1$ if species $i$ \textit{consumes} metabolite $m$ ($i = 1,\dots,844; m = 1,\dots,283$). We then used 

\begin{equation}
\m Kij = 
\dfrac{\displaystyle \sum_{m = 1}^{283} \m Bmi \m Bmj}
{\displaystyle \sum_{m = 1}^{283} \m Bmi}
\label{Kij}
\end{equation}

to construct a weighted directed complemnetarity network. In this network the links connect species that compete over the same metabolites. The link weights capture the strength of the competition, quantifying the fraction of $i$'s consumed matebolites (denominator) over which it must compete with $j$ (numerator). The resulting $K$ has a small fraction of isolated species, hence we consider only its giant connected components, which includes $N = 737$ microbial species linked through $L = 113,350$ competitive interactions.
	
\noindent {\bf Microbial 2}.\
Using $B$ above we now construct a mutualistic network via

\begin{equation}
\m Kij = 
\dfrac{\displaystyle \sum_{m = 1}^{283} \m Bjm \m Bmi}
{\displaystyle \sum_{m = 1}^{283} \m Bmi},
\label{Kij2}
\end{equation}

now describing the fraction of $i$'s total consumption (denominator) that is produced by $j$ (numerator). Here, the connected component remains with $N = 496$ nodes and $L=43,964$ links. 

The two networks are of different nature:\ Microbial 1 is adversarial, relevant \textit{e.g}., for Inhibitory, while Microbial 2 is cooperative, naturally fitting our Population 1/2 dynamics. Still, for the purpose of examining our theoretical predictions, and mainly for confronting them with empirically observed networks, we applied our Population 1/2 dynamics on both Microbial 1 and 2, despite the fact that the former, is, perhaps, less relevant.	 
	
\noindent {\bf Power 1}.\
Mapping a segment from the power network of Great Britain, consisting of $N = 2,224$ nodes and $L = 2,804$ links. The nodes are split into $394$ generators and $1,830$ consumer loads. The network data can be downloaded from \textit{\color{blue} http://www.nationalgrid.com}
	
\noindent {\bf Power 2}.\
A segment of the Polish power network, typically referred to as "case2383" \cite{zimmerman2010matpower,motter2013spontaneous,nishikawa2015comparative}. The network has $N = 2,383$ nodes, $327$ of which are generators and the remaining $2,056$ are consumer loads. These loads and generators are linked through $L= 2,886$ transmission lines. This data can be downloaded from \textit{\color{blue} roman.korabat@polsl.pl}.

%%%%%%%%%%%%%%%%%%%%%%%%%%%%%%%%%%%%%%%%%%%%%%%%%%%%%%%%%%%%%%%%%%%%%%%%%%%%%%%%%%%%% 
%%%%%%%%%%%%%%%%%%%%%%%%%%%%%%%%%%%%%%%%%%%%%%%%%%%%%%%%%%%%%%%%%%%%%%%%%%%%%%%%%%%%% 
{\color{blue} \rule{12cm}{1mm}}

%%%%%%%%%%%%%%%%%%
%% BIBLIOGRAPHY %%
%%%%%%%%%%%%%%%%%%

%\clearpage

\clearpage

%\bibliographystyle{unsrt}
%\bibliographystyle{unsrtnat}
%\bibliography{./SI.bib}

%\end{document}
